# Supplementary material for: Scheme and gauge dependence of QCD fixed points at five loops
Source: arXiv:2306.09056 ancillary file (2023-07-13)
Supplement: Supplementary file 1 [file qcdexps5spm.pdf]

# Supplementary Material

| $N_f$ | $a_\infty$ | $\alpha_\infty$ | $\omega_1$ | $\omega_2$ | Infrared Stability |
|---|---|---|---|---|---|
| 0 | $-0.107843$ | $0.000000$ | $-1.186275$ | $0.070970$ | Saddle |
| | $-0.107843$ | $2.022676$ | $-0.178029$ | $-1.186275$ | Unstable |
| | $-0.107843$ | $-1.340858$ | $-0.118017$ | $-1.186275$ | Unstable |
| 1 | $-0.115672$ | $0.000000$ | $-1.195274$ | $0.077312$ | Saddle |
| | $-0.115672$ | $1.739654$ | $-0.168421$ | $-1.195274$ | Unstable |
| | $-0.115672$ | $-1.476213$ | $-0.142917$ | $-1.195274$ | Unstable |
| 2 | $-0.126087$ | $0.000000$ | $-1.218841$ | $0.080517$ | Saddle |
| | $-0.126087$ | $1.397760$ | $-0.150403$ | $-1.218841$ | Unstable |
| | $-0.126087$ | $-1.610404$ | $-0.173284$ | $-1.218841$ | Unstable |
| 3 | $-0.140625$ | $0.000000$ | $-1.265625$ | $0.076630$ | Saddle |
| | $-0.140625$ | $0.986511$ | $-0.119932$ | $-1.265625$ | Unstable |
| | $-0.140625$ | $-1.745771$ | $-0.212237$ | $-1.265625$ | Unstable |
| 4 | $-0.162338$ | $0.000000$ | $-1.352814$ | $0.055211$ | Saddle |
| | $-0.162338$ | $0.493483$ | $-0.069651$ | $-1.352814$ | Unstable |
| | $-0.162338$ | $-1.886816$ | $-0.266307$ | $-1.352814$ | Unstable |
| 5 | $-0.198276$ | $0.000000$ | $-1.520115$ | $-0.016879$ | Unstable |
| | $-0.198276$ | $-0.093341$ | $0.016108$ | $-1.520115$ | Saddle |
| | $-0.198276$ | $-2.044340$ | $-0.352803$ | $-1.520115$ | Unstable |
| 6 | $-0.269231$ | $0.000000$ | $-1.884615$ | $-0.283469$ | Unstable |
| | $-0.269231$ | $-0.771796$ | $0.186320$ | $-1.884615$ | Saddle |
| | $-0.269231$ | $-2.252013$ | $-0.543661$ | $-1.884615$ | Unstable |
| 7 | $-0.475000$ | $0.000000$ | $-3.008333$ | $-1.951953$ | Unstable |
| | $-0.475000$ | $-1.456400$ | $0.875162$ | $-3.008333$ | Saddle |
| | $-0.475000$ | $-2.640091$ | $-1.586452$ | $-3.008333$ | Unstable |
| 8 | $-8.500000$ | $0.000000$ | $-1090.656250$ | $-48.166667$ | Unstable |
| | $-8.500000$ | $-1.911284$ | $496.814577$ | $-48.166667$ | Saddle |
| | $-8.500000$ | $-3.510285$ | $-912.455202$ | $-48.166667$ | Unstable |

Table SM.1: Two loop $\overline{\text{MS}}$ scheme $SU(3)$ fixed points in the linear covariant gauge for $0 \leq N_f \leq 8$.

| $N_f$ | $a_\infty$ | $\alpha_\infty$ | $\omega_1$ | $\omega_2$ | Infrared Stability |
|---|---|---|---|---|---|
| 9 | 0.416667 | 0.000000 | −4.153646 | 2.083333 | Saddle |
| | 0.416667 | −2.146730 | 2.353470 | 2.083333 | **Stable** |
| | 0.416667 | −4.953270 | −5.430293 | 2.083333 | Saddle |
| 10 | 0.175676 | 0.000000 | −1.118449 | 0.761261 | Saddle |
| | 0.175676 | −2.303972 | 0.749845 | 0.761261 | **Stable** |
| | 0.175676 | −6.990900 | −2.275239 | 0.761261 | Saddle |
| 11 | 0.098214 | 0.000000 | −0.520338 | 0.360119 | Saddle |
| | 0.098214 | −2.432707 | 0.391895 | 0.360119 | **Stable** |
| | 0.098214 | −9.855172 | −1.587611 | 0.360119 | Saddle |
| 12 | 0.060000 | 0.000000 | −0.290250 | 0.180000 | Saddle |
| | 0.060000 | −2.548046 | 0.237660 | 0.180000 | **Stable** |
| | 0.060000 | −14.063065 | −1.311685 | 0.180000 | Saddle |
| 13 | 0.037234 | 0.000000 | −0.171886 | 0.086879 | Saddle |
| | 0.037234 | −2.655694 | 0.149886 | 0.086879 | **Stable** |
| | 0.037234 | −20.749068 | −1.171065 | 0.086879 | Saddle |
| 14 | 0.022124 | 0.000000 | −0.099863 | 0.036873 | Saddle |
| | 0.022124 | −2.758253 | 0.091485 | 0.036873 | **Stable** |
| | 0.022124 | −32.875081 | −1.090390 | 0.036873 | Saddle |
| 15 | 0.011364 | 0.000000 | −0.050894 | 0.011364 | Saddle |
| | 0.011364 | −2.857085 | 0.048523 | 0.011364 | **Stable** |
| | 0.011364 | −61.309582 | −1.041235 | 0.011364 | Saddle |
| 16 | 0.003311 | 0.000000 | −0.014853 | 0.001104 | Saddle |
| | 0.003311 | −2.952985 | 0.014638 | 0.001104 | **Stable** |
| | 0.003311 | −203.880349 | −1.010609 | 0.001104 | Saddle |

Table SM.2: Two loop $\overline{\text{MS}}$ scheme $SU(3)$ fixed points in the linear covariant gauge for $9 \leq N_f \leq 16$.

| $N_f$ | $a_\infty$ | $\alpha_\infty$ | $\omega_1$ | $\omega_2$ | Infrared Stability |
|---|---|---|---|---|---|
| 0 | - | - | - | - | - |
| 1 | - | - | - | - | - |
| 2 | - | - | - | - | - |
| 3 | - | - | - | - | - |
| 4 | - | - | - | - | - |
| 5 | - | - | - | - | - |
| 6 | 1.012686 | 0.000000 | 40.841486 | 92.653913 | **Stable** |
| | $-0.212686$ | 0.000000 | $-1.801486$ | $-1.072394$ | Unstable |
| | 1.012686 | 0.599810 | $-108.808649$ | 40.841486 | Saddle |
| | $-0.212686$ | 0.973147 | 1.389878 | $-1.801486$ | Saddle |
| 7 | 0.195518 | 0.000000 | 0.161289 | 2.986261 | **Stable** |
| | $-0.138506$ | 0.000000 | $-1.498628$ | $-0.340879$ | Unstable |
| | 0.195518 | 0.102994 | $-0.164987$ | 2.986261 | Saddle |
| | $-0.138506$ | 1.092251 | 0.437838 | $-1.498628$ | Saddle |
| 8 | 0.116505 | 0.000000 | $-0.176683$ | 1.329441 | Saddle |
| | $-0.114930$ | 0.000000 | $-1.293733$ | $-0.226483$ | Unstable |
| | 0.116505 | $-0.384782$ | 0.165281 | 1.329441 | **Stable** |
| | $-0.114930$ | 1.195949 | 0.288321 | $-1.293733$ | Saddle |
| 9 | 0.081803 | 0.000000 | $-0.193341$ | 0.737728 | Saddle |
| | $-0.101786$ | 0.000000 | $-1.142187$ | $-0.183834$ | Unstable |
| | 0.081803 | $-0.858773$ | 0.172635 | 0.737728 | **Stable** |
| | $-0.101786$ | 1.309970 | 0.233233 | $-1.142187$ | Saddle |

Table SM.3: Three loop $\overline{\text{MS}}$ scheme $SU(3)$ fixed points in the linear covariant gauge for $0 \leq N_f \leq 9$.

| $N_f$ | $a_\infty$ | $\alpha_\infty$ | $\omega_1$ | $\omega_2$ | Infrared Stability |
|---|---|---|---|---|---|
| 10 | 0.060824 | 0.000000 | −0.175883 | 0.435887 | Saddle |
| | −0.093036 | 0.000000 | −1.019824 | −0.164069 | Unstable |
| | 0.060824 | −1.298293 | 0.154800 | 0.435887 | **Stable** |
| | −0.093036 | 1.437391 | 0.208534 | −1.019824 | Saddle |
| 11 | 0.046039 | 0.000000 | −0.151892 | 0.258488 | Saddle |
| | −0.086664 | 0.000000 | −0.915931 | −0.154656 | Unstable |
| | 0.046039 | −1.692825 | 0.134329 | 0.258488 | **Stable** |
| | −0.086664 | 1.579005 | 0.197855 | −0.915931 | Saddle |
| 12 | 0.034607 | 0.000000 | −0.125974 | 0.147759 | Saddle |
| | −0.081769 | 0.000000 | −0.824922 | −0.151024 | Unstable |
| | 0.034607 | −2.039860 | 0.113066 | 0.147759 | **Stable** |
| | −0.081769 | 1.735493 | 0.195342 | −0.824922 | Saddle |
| 13 | 0.025191 | 0.000000 | −0.099007 | 0.077790 | Saddle |
| | −0.077882 | 0.000000 | −0.743563 | −0.151207 | Unstable |
| | 0.025191 | −2.339613 | 0.090641 | 0.077790 | **Stable** |
| | −0.077882 | 1.907924 | 0.198629 | −0.743563 | Saddle |
| 14 | 0.017070 | 0.000000 | −0.071194 | 0.034949 | Saddle |
| | −0.074734 | 0.000000 | −0.669865 | −0.154336 | Unstable |
| | 0.017070 | −2.591922 | 0.066678 | 0.034949 | **Stable** |
| | −0.074734 | 2.097958 | 0.206887 | −0.669865 | Saddle |
| 15 | 0.009818 | 0.000000 | −0.042753 | 0.011153 | Saddle |
| | −0.072163 | 0.000000 | −0.602581 | −0.160122 | Unstable |
| | 0.009818 | −2.795125 | 0.041052 | 0.011153 | **Stable** |
| | −0.072163 | 2.308018 | 0.220201 | −0.602581 | Saddle |
| 16 | 0.003162 | 0.000000 | −0.014138 | 0.001102 | Saddle |
| | −0.070071 | 0.000000 | −0.540976 | −0.168684 | Unstable |
| | 0.003162 | −2.945839 | 0.013943 | 0.001102 | **Stable** |
| | −0.070071 | 2.541509 | 0.239440 | −0.540976 | Saddle |

Table SM.4: Three loop $\overline{\text{MS}}$ scheme $SU(3)$ fixed points in the linear covariant gauge for $10 \leq N_f \leq 16$.

| $N_f$ | $a_\infty$ | $\alpha_\infty$ | $\omega_1$ | $\omega_2$ | Infrared Stability |
|---|---|---|---|---|---|
| 0 | $-0.072415$ | 0.000000 | $-1.862385$ | 0.077318 | Saddle |
| | $-0.072415$ | 1.958995 | $-0.210635$ | $-1.862385$ | Unstable |
| | $-0.072415$ | $-1.858656$ | $-0.137925$ | $-1.862385$ | Unstable |
| 1 | $-0.076801$ | 0.000000 | $-1.850154$ | 0.090949 | Saddle |
| | $-0.076801$ | 1.876451 | $-0.238199$ | $-1.850154$ | Unstable |
| | $-0.076801$ | $-1.945237$ | $-0.168349$ | $-1.850154$ | Unstable |
| 2 | $-0.082085$ | 0.000000 | $-1.841408$ | 0.107011 | Saddle |
| | $-0.082085$ | 1.791106 | $-0.273312$ | $-1.841408$ | Unstable |
| | $-0.082085$ | $-1.986475$ | $-0.202414$ | $-1.841408$ | Unstable |
| 3 | $-0.088492$ | 0.000000 | $-1.833095$ | 0.127670 | Saddle |
| | $-0.088492$ | 1.718163 | $-0.324939$ | $-1.833095$ | Unstable |
| | $-0.088492$ | $-1.973316$ | $-0.240390$ | $-1.833095$ | Unstable |
| 4 | $-0.096211$ | 0.000000 | $-1.816819$ | 0.157478 | Saddle |
| | $-0.096211$ | 1.681791 | $-0.413554$ | $-1.816819$ | Unstable |
| | $-0.096211$ | $-1.897177$ | $-0.283624$ | $-1.816819$ | Unstable |
| 5 | $-0.105089$ | 0.000000 | $-1.772958$ | 0.204739 | Saddle |
| | $-0.105089$ | 1.716581 | $-0.585228$ | $-1.772958$ | Unstable |
| | $-0.105089$ | $-1.757724$ | $-0.336453$ | $-1.772958$ | Unstable |
| 6 | $-0.113620$ | 0.000000 | $-1.667057$ | 0.275179 | Saddle |
| | $-0.113620$ | 1.860505 | $-0.918472$ | $-1.667057$ | Unstable |
| | $-0.113620$ | $-1.572135$ | $-0.399739$ | $-1.667057$ | Unstable |
| 7 | $-0.116983$ | 0.000000 | $-1.483338$ | 0.331471 | Saddle |
| | $-0.116983$ | 2.137745 | $-1.392486$ | $-1.483338$ | Unstable |
| | $-0.116983$ | $-1.362906$ | $-0.427244$ | $-1.483338$ | Unstable |
| 8 | 0.123312 | 0.000000 | 0.595200 | 1.323045 | **Stable** |
| | 1.142863 | 0.000000 | $-610.561252$ | 5845.308783 | Saddle |
| | $-0.109864$ | 0.000000 | $-1.290397$ | 0.292714 | Saddle |
| | 0.123312 | 0.868700 | $-0.835990$ | 1.323045 | Saddle |
| | 0.123312 | $-4.722120$ | $-3.896822$ | 1.323045 | Saddle |
| | 1.142863 | 2.015974 | $-16492.492395$ | $-610.561252$ | Unstable |
| | 1.142863 | $-2.881123$ | $-9121.625730$ | $-610.561252$ | Unstable |
| | $-0.109864$ | 2.548531 | $-1.651208$ | $-1.290397$ | Unstable |
| | $-0.109864$ | $-1.148748$ | $-0.344929$ | $-1.290397$ | Unstable |

Table SM.5: Four loop $\overline{\text{MS}}$ scheme $SU(3)$ fixed points in the linear covariant gauge for $0 \leq N_f \leq 8$.

| $N_f$ | $a_\infty$ | $\alpha_\infty$ | $\omega_1$ | $\omega_2$ | Infrared Stability |
|---|---|---|---|---|---|
| 9 | 0.085291 | 0.000000 | 0.017807 | 0.732193 | **Stable** |
| | 0.962002 | 0.000000 | −542.394739 | 3638.528050 | Saddle |
| | −0.096487 | 0.000000 | −1.131329 | 0.207740 | Saddle |
| | 0.085291 | 0.078057 | −0.018214 | 0.732193 | Saddle |
| | 0.085291 | −5.882389 | −1.983191 | 0.732193 | Saddle |
| | 0.962002 | 2.372214 | −12107.306162 | −542.394739 | Unstable |
| | 0.962002 | −2.710372 | −4877.065906 | −542.394739 | Unstable |
| | −0.096487 | 3.067092 | −1.597506 | −1.131329 | Unstable |
| | −0.096487 | −0.983642 | −0.231735 | −1.131329 | Unstable |
| 10 | 0.064860 | 0.000000 | −0.096514 | 0.426703 | Saddle |
| | 0.446940 | 0.000000 | −72.410221 | 216.607652 | Saddle |
| | −0.083591 | 0.000000 | −0.984127 | 0.149490 | Saddle |
| | 0.064860 | −0.758788 | 0.084116 | 0.426703 | **Stable** |
| | 0.064860 | −7.285851 | −1.593756 | 0.426703 | Saddle |
| | 0.446940 | 2.631336 | −770.095520 | −72.410221 | Unstable |
| | 0.446940 | −2.802990 | −276.712319 | −72.410221 | Unstable |
| | −0.083591 | 3.656712 | −1.486077 | −0.984127 | Unstable |
| | −0.083591 | −0.905248 | −0.161980 | −0.984127 | Unstable |
| 11 | 0.049832 | 0.000000 | −0.125835 | 0.249017 | Saddle |
| | 0.262159 | 0.000000 | −18.805627 | 32.056161 | Saddle |
| | −0.072993 | 0.000000 | −0.843350 | 0.118865 | Saddle |
| | 0.049832 | −1.444524 | 0.107670 | 0.249017 | **Stable** |
| | 0.049832 | −9.164022 | −1.495291 | 0.249017 | Saddle |
| | 0.262159 | 2.797166 | −114.552315 | −18.805627 | Unstable |
| | 0.262159 | −3.009747 | −40.855724 | −18.805627 | Unstable |
| | −0.072993 | 4.294343 | −1.409230 | −0.843350 | Unstable |
| | −0.072993 | −0.905709 | −0.127024 | −0.843350 | Unstable |
| 12 | 0.037434 | 0.000000 | −0.121873 | 0.141164 | Saddle |
| | 0.182641 | 0.000000 | −8.151111 | 9.044557 | Saddle |
| | −0.064423 | 0.000000 | −0.711375 | 0.103736 | Saddle |
| | 0.037434 | −1.945284 | 0.106950 | 0.141164 | **Stable** |
| | 0.037434 | −11.872619 | −1.477787 | 0.141164 | Saddle |
| | 0.182641 | 2.874023 | −31.268962 | −8.151111 | Unstable |
| | 0.182641 | −3.270103 | −11.852903 | −8.151111 | Unstable |
| | −0.064423 | 4.973543 | −1.366444 | −0.711375 | Unstable |
| | −0.064423 | −0.966448 | −0.110272 | −0.711375 | Unstable |

Table SM.6: Four loop $\overline{\text{MS}}$ scheme $SU(3)$ fixed points in the linear covariant gauge for $9 \leq N_f \leq 12$.

| $N_f$ | $a_\infty$ | $\alpha_\infty$ | $\omega_1$ | $\omega_2$ | Infrared Stability |
|---|---|---|---|---|---|
| 13 | 0.026853 | 0.000000 | −0.101310 | 0.074565 | Saddle |
| | 0.141687 | 0.000000 | −4.907150 | 3.754144 | Saddle |
| | −0.057340 | 0.000000 | −0.589242 | 0.096633 | Saddle |
| | 0.026853 | −2.312632 | 0.091708 | 0.074565 | **Stable** |
| | 0.026853 | −16.124358 | −1.476144 | 0.074565 | Saddle |
| | 0.141687 | 2.881045 | −12.298078 | −4.907150 | Unstable |
| | 0.141687 | −3.553712 | −5.175980 | −4.907150 | Unstable |
| | −0.057340 | 5.699812 | −1.346245 | −0.589242 | Unstable |
| | −0.057340 | −1.073342 | −0.102703 | −0.589242 | Unstable |
| 14 | 0.017793 | 0.000000 | −0.073373 | 0.033906 | Saddle |
| | 0.117756 | 0.000000 | −3.633611 | 1.980404 | Saddle |
| | −0.051298 | 0.000000 | −0.476616 | 0.093737 | Saddle |
| | 0.017793 | −2.588296 | 0.068423 | 0.033906 | **Stable** |
| | 0.017793 | −23.713794 | −1.471549 | 0.033906 | Saddle |
| | 0.117756 | 2.842775 | −6.094849 | −3.633611 | Unstable |
| | 0.117756 | −3.843479 | −2.923578 | −3.633611 | Unstable |
| | −0.051298 | 6.488747 | −1.340441 | −0.476616 | Unstable |
| | −0.051298 | −1.217861 | −0.099942 | −0.476616 | Unstable |
| 15 | 0.010001 | 0.000000 | −0.043478 | 0.010988 | Saddle |
| | 0.102368 | 0.000000 | −3.051413 | 1.218110 | Saddle |
| | −0.045958 | 0.000000 | −0.372592 | 0.093047 | Saddle |
| | 0.010001 | −2.795819 | 0.041706 | 0.010988 | **Stable** |
| | 0.010001 | −41.152460 | −1.462900 | 0.010988 | Saddle |
| | 0.102368 | 2.778768 | −3.516462 | −3.051413 | Unstable |
| | 0.102368 | −4.129750 | −1.950938 | −3.051413 | Unstable |
| | −0.045958 | 7.368878 | −1.344138 | −0.372592 | Unstable |
| | −0.045958 | −1.395950 | −0.099753 | −0.372592 | Unstable |
| 16 | 0.003170 | 0.000000 | −0.014174 | 0.001099 | Saddle |
| | 0.091700 | 0.000000 | −2.761435 | 0.828759 | Saddle |
| | −0.041033 | 0.000000 | −0.276077 | 0.093380 | Saddle |
| | 0.003170 | −2.945935 | 0.013978 | 0.001099 | **Stable** |
| | 0.003170 | −126.835296 | −1.453369 | 0.001099 | Saddle |
| | 0.091700 | 2.700828 | −2.247803 | −2.761435 | Unstable |
| | 0.091700 | −4.407403 | −1.453956 | −2.761435 | Unstable |
| | −0.041033 | 8.392550 | −1.354522 | −0.276077 | Unstable |
| | −0.041033 | −1.607691 | −0.100819 | −0.276077 | Unstable |

Table SM.7: Four loop $\overline{\text{MS}}$ scheme $SU(3)$ fixed points in the linear covariant gauge for $13 \leq N_f \leq 16$.

| $N_f$ | $a_\infty$ | $\alpha_\infty$ | $\omega_1$ | $\omega_2$ | Infrared Stability |
|---|---|---|---|---|---|
| 0 | - | - | - | - | - |
| 1 | - | - | - | - | - |
| 2 | - | - | - | - | - |
| 3 | - | - | - | - | - |
| 4 | - | - | - | - | - |
| 5 | −0.125111 | 0.000000 | −1.547127 | 1.586547 | Saddle |
| | −0.279400 | 0.000000 | 22.006345 | 77.197903 | **Stable** |
| | −0.125111 | −3.674157 | −6.090596 | −1.547127 | Unstable |
| | −0.279400 | −4.231805 | −467.077204 | 22.006345 | Saddle |
| 6 | −0.113974 | 0.000000 | −1.664633 | 1.115774 | Saddle |
| | −9.122662 | 0.000000 | 17178776.772536 | 2766996660.359280 | **Stable** |
| | −0.113974 | −3.734328 | −4.662800 | −1.664633 | Unstable |
| | −9.122662 | −4.690539 | −26191416650.567139 | 17178776.772536 | Saddle |
| 7 | - | - | - | - | - |
| 8 | - | - | - | - | - |
| 9 | - | - | - | - | - |
| 10 | - | - | - | - | - |
| 11 | - | - | - | - | - |
| 12 | - | - | - | - | - |
| 13 | 0.032315 | 0.000000 | −0.122684 | 0.036682 | Saddle |
| | 0.041343 | 0.000000 | −0.151397 | −0.072312 | Unstable |
| | 0.032315 | −2.386609 | 0.109561 | 0.036682 | **Stable** |
| | 0.041343 | −2.470802 | 0.131351 | −0.072312 | Saddle |
| 14 | 0.018526 | 0.000000 | −0.076782 | 0.031152 | Saddle |
| | 0.046357 | 0.000000 | −0.365291 | −0.176646 | Unstable |
| | 0.018526 | −2.603426 | 0.071510 | 0.031152 | **Stable** |
| | 0.046357 | −2.932818 | 0.152600 | −0.365291 | Saddle |
| 15 | 0.010078 | 0.000000 | −0.043850 | 0.010828 | Saddle |
| | 0.047107 | 0.000000 | −0.587861 | −0.190657 | Unstable |
| | 0.010078 | −2.797897 | 0.042058 | 0.010828 | **Stable** |
| | 0.047107 | −3.326390 | 0.168639 | −0.587861 | Saddle |
| 16 | 0.003171 | 0.000000 | −0.014178 | 0.001098 | Saddle |
| | 0.046999 | 0.000000 | −0.780464 | −0.202969 | Unstable |
| | 0.003171 | −2.945965 | 0.013982 | 0.001098 | **Stable** |
| | 0.046999 | −3.682521 | 0.185665 | −0.780464 | Saddle |

Table SM.8: Five loop $\overline{\text{MS}}$ scheme $SU(3)$ fixed points in the linear covariant gauge for $0 \leq N_f \leq 16$.

| $N_f$ | $a_\infty$ | $\alpha_\infty$ | $\omega_1$ | $\omega_2$ | Infrared Stability |
|---|---|---|---|---|---|
| 0 | $-0.107843$ | 0.000000 | $-1.186275$ | 0.070970 | Saddle |
| | $-0.107843$ | 1.709529 | $-0.090089$ | $-1.186275$ | Unstable |
| | $-0.107843$ | $-6.345892$ | $-0.334417$ | $-1.186275$ | Unstable |
| 1 | $-0.115672$ | 0.000000 | $-1.195274$ | 0.077312 | Saddle |
| | $-0.115672$ | 1.477840 | $-0.093750$ | $-1.195274$ | Unstable |
| | $-0.115672$ | $-6.950958$ | $-0.440947$ | $-1.195274$ | Unstable |
| 2 | $-0.126087$ | 0.000000 | $-1.218841$ | 0.080517 | Saddle |
| | $-0.126087$ | 1.183367 | $-0.093040$ | $-1.218841$ | Unstable |
| | $-0.126087$ | $-7.608654$ | $-0.598218$ | $-1.218841$ | Unstable |
| 3 | $-0.140625$ | 0.000000 | $-1.265625$ | 0.076630 | Saddle |
| | $-0.140625$ | 0.825598 | $-0.084212$ | $-1.265625$ | Unstable |
| | $-0.140625$ | $-8.344117$ | $-0.851106$ | $-1.265625$ | Unstable |
| 4 | $-0.162338$ | 0.000000 | $-1.352814$ | 0.055211 | Saddle |
| | $-0.162338$ | 0.405190 | $-0.057644$ | $-1.352814$ | Unstable |
| | $-0.162338$ | $-9.191856$ | $-1.307681$ | $-1.352814$ | Unstable |
| 5 | $-0.198276$ | 0.000000 | $-1.520115$ | $-0.016879$ | Unstable |
| | $-0.198276$ | $-0.074828$ | 0.016755 | $-1.520115$ | Saddle |
| | $-0.198276$ | $-10.200534$ | $-2.284076$ | $-1.520115$ | Unstable |
| 6 | $-0.269231$ | 0.000000 | $-1.884615$ | $-0.283469$ | Unstable |
| | $-0.269231$ | $-0.607732$ | 0.268410 | $-1.884615$ | Saddle |
| | $-0.269231$ | $-11.439887$ | $-5.052526$ | $-1.884615$ | Unstable |
| 7 | $-0.475000$ | 0.000000 | $-3.008333$ | $-1.951953$ | Unstable |
| | $-0.475000$ | $-1.182096$ | 1.774610 | $-3.008333$ | Saddle |
| | $-0.475000$ | $-13.010886$ | $-19.532461$ | $-3.008333$ | Unstable |
| 8 | $-8.500000$ | 0.000000 | $-1090.656250$ | $-48.166667$ | Unstable |
| | $-8.500000$ | $-1.781823$ | 961.626550 | $-48.166667$ | Saddle |
| | $-8.500000$ | $-15.061314$ | $-8128.392175$ | $-48.166667$ | Unstable |

Table SM.9: Two loop $\overline{\text{MS}}$ scheme $SU(3)$ fixed points in the Curci-Ferrari gauge for $0 \leq N_f \leq 8$.

| $N_f$ | $a_\infty$ | $\alpha_\infty$ | $\omega_1$ | $\omega_2$ | Infrared Stability |
|---|---|---|---|---|---|
| 9 | 0.416667 | 0.000000 | $-4.153646$ | 2.083333 | Saddle |
| | 0.416667 | $-2.387888$ | 3.596809 | 2.083333 | **Stable** |
| | 0.416667 | $-17.812112$ | $-26.829882$ | 2.083333 | Saddle |
| 10 | 0.175676 | 0.000000 | $-1.118449$ | 0.761261 | Saddle |
| | 0.175676 | $-2.981627$ | 0.964118 | 0.761261 | **Stable** |
| | 0.175676 | $-21.608116$ | $-6.987048$ | 0.761261 | Saddle |
| 11 | 0.098214 | 0.000000 | $-0.520338$ | 0.360119 | Saddle |
| | 0.098214 | $-3.548192$ | 0.452028 | 0.360119 | **Stable** |
| | 0.098214 | $-27.027566$ | $-3.443224$ | 0.360119 | Saddle |
| 12 | 0.060000 | 0.000000 | $-0.290250$ | 0.180000 | Saddle |
| | 0.060000 | $-4.078489$ | 0.256566 | 0.180000 | **Stable** |
| | 0.060000 | $-35.143733$ | $-2.210791$ | 0.180000 | Saddle |
| 13 | 0.037234 | 0.000000 | $-0.171886$ | 0.086879 | Saddle |
| | 0.037234 | $-4.569040$ | 0.155606 | 0.086879 | **Stable** |
| | 0.037234 | $-48.240484$ | $-1.642904$ | 0.086879 | Saddle |
| 14 | 0.022124 | 0.000000 | $-0.099863$ | 0.036873 | Saddle |
| | 0.022124 | $-5.020489$ | 0.092924 | 0.036873 | **Stable** |
| | 0.022124 | $-72.246178$ | $-1.337198$ | 0.036873 | Saddle |
| 15 | 0.011364 | 0.000000 | $-0.050894$ | 0.011364 | Saddle |
| | 0.011364 | $-5.435844$ | 0.048748 | 0.011364 | **Stable** |
| | 0.011364 | $-128.897489$ | $-1.155936$ | 0.011364 | Saddle |
| 16 | 0.003311 | 0.000000 | $-0.014853$ | 0.001104 | Saddle |
| | 0.003311 | $-5.819105$ | 0.014644 | 0.001104 | **Stable** |
| | 0.003311 | $-413.847562$ | $-1.041453$ | 0.001104 | Saddle |

Table SM.10: Two loop $\overline{\text{MS}}$ scheme $SU(3)$ fixed points in the Curci-Ferrari gauge for $9 \leq N_f \leq 16$.

| $N_f$ | $a_\infty$ | $\alpha_\infty$ | $\omega_1$ | $\omega_2$ | Infrared Stability |
|---|---|---|---|---|---|
| 0 | - | - | - | - | - |
| 1 | - | - | - | - | - |
| 2 | - | - | - | - | - |
| 3 | - | - | - | - | - |
| 4 | - | - | - | - | - |
| 5 | - | - | - | - | - |
| 6 | 1.012686 | 0.000000 | 40.841486 | 92.653913 | **Stable** |
| | $-0.212686$ | 0.000000 | $-1.801486$ | $-1.072394$ | Unstable |
| | 1.012686 | 0.773985 | $-101.745391$ | 40.841486 | Saddle |
| | $-0.212686$ | 1.371370 | 1.292577 | $-1.801486$ | Saddle |
| 7 | 0.195518 | 0.000000 | 0.161289 | 2.986261 | **Stable** |
| | $-0.138506$ | 0.000000 | $-1.498628$ | $-0.340879$ | Unstable |
| | 0.195518 | 0.134812 | $-0.163479$ | 2.986261 | Saddle |
| | $-0.138506$ | 1.679867 | 0.424432 | $-1.498628$ | Saddle |
| 8 | 0.116505 | 0.000000 | $-0.176683$ | 1.329441 | Saddle |
| | $-0.114930$ | 0.000000 | $-1.293733$ | $-0.226483$ | Unstable |
| | 0.116505 | $-0.525277$ | 0.169160 | 1.329441 | **Stable** |
| | $-0.114930$ | 1.949318 | 0.287924 | $-1.293733$ | Saddle |
| 9 | 0.081803 | 0.000000 | $-0.193341$ | 0.737728 | Saddle |
| | $-0.101786$ | 0.000000 | $-1.142187$ | $-0.183834$ | Unstable |
| | 0.081803 | $-1.239118$ | 0.177887 | 0.737728 | **Stable** |
| | $-0.101786$ | 2.228306 | 0.238144 | $-1.142187$ | Saddle |

Table SM.11: Three loop $\overline{\text{MS}}$ scheme $SU(3)$ fixed points in the Curci-Ferrari gauge for $0 \leq N_f \leq 9$.

| $N_f$ | $a_\infty$ | $\alpha_\infty$ | $\omega_1$ | $\omega_2$ | Infrared Stability |
|---|---|---|---|---|---|
| 10 | 0.060824 | 0.000000 | −0.175883 | 0.435887 | Saddle |
| | −0.093036 | 0.000000 | −1.019824 | −0.164069 | Unstable |
| | 0.060824 | −1.988405 | 0.158258 | 0.435887 | **Stable** |
| | −0.093036 | 2.524886 | 0.216576 | −1.019824 | Saddle |
| 11 | 0.046039 | 0.000000 | −0.151892 | 0.258488 | Saddle |
| | −0.086664 | 0.000000 | −0.915931 | −0.154656 | Unstable |
| | 0.046039 | −2.744498 | 0.135852 | 0.258488 | **Stable** |
| | −0.086664 | 2.841939 | 0.208196 | −0.915931 | Saddle |
| 12 | 0.034607 | 0.000000 | −0.125974 | 0.147759 | Saddle |
| | −0.081769 | 0.000000 | −0.824922 | −0.151024 | Unstable |
| | 0.034607 | −3.479125 | 0.113468 | 0.147759 | **Stable** |
| | −0.081769 | 3.181434 | 0.207609 | −0.824922 | Saddle |
| 13 | 0.025191 | 0.000000 | −0.099007 | 0.077790 | Saddle |
| | −0.077882 | 0.000000 | −0.743563 | −0.151207 | Unstable |
| | 0.025191 | −4.169158 | 0.090635 | 0.077790 | **Stable** |
| | −0.077882 | 3.545574 | 0.212631 | −0.743563 | Saddle |
| 14 | 0.017070 | 0.000000 | −0.071194 | 0.034949 | Saddle |
| | −0.074734 | 0.000000 | −0.669865 | −0.154336 | Unstable |
| | 0.017070 | −4.796907 | 0.066620 | 0.034949 | **Stable** |
| | −0.074734 | 3.937302 | 0.222503 | −0.669865 | Saddle |
| 15 | 0.009818 | 0.000000 | −0.042753 | 0.011153 | Saddle |
| | −0.072163 | 0.000000 | −0.602581 | −0.160122 | Unstable |
| | 0.009818 | −5.347954 | 0.041032 | 0.011153 | **Stable** |
| | −0.072163 | 4.360696 | 0.237312 | −0.602581 | Saddle |
| 16 | 0.003162 | 0.000000 | −0.014138 | 0.001102 | Saddle |
| | −0.070071 | 0.000000 | −0.540976 | −0.168684 | Unstable |
| | 0.003162 | −5.808458 | 0.013942 | 0.001102 | **Stable** |
| | −0.070071 | 4.821387 | 0.257876 | −0.540976 | Saddle |

Table SM.12: Three loop $\overline{\text{MS}}$ scheme $SU(3)$ fixed points in the Curci-Ferrari gauge for $10 \leq N_f \leq 16$.

| $N_f$ | $a_\infty$ | $\alpha_\infty$ | $\omega_1$ | $\omega_2$ | Infrared Stability |
|---|---|---|---|---|---|
| 0 | $-0.107843$ | $0.635873$ | $-0.441270$ | $-1.186275$ | Unstable |
| | $-0.107843$ | $-0.698616$ | $0.381724$ | $-1.186275$ | Saddle |
| | $-0.107843$ | $-9.253462$ | $-2.828799$ | $-1.186275$ | Unstable |
| 1 | $-0.115672$ | $0.702774$ | $-0.587925$ | $-1.195274$ | Unstable |
| | $-0.115672$ | $-0.795812$ | $0.501537$ | $-1.195274$ | Saddle |
| | $-0.115672$ | $-9.496022$ | $-3.413267$ | $-1.195274$ | Unstable |
| 2 | $-0.126087$ | $0.742844$ | $-0.781626$ | $-1.218841$ | Unstable |
| | $-0.126087$ | $-0.885927$ | $0.660372$ | $-1.218841$ | Saddle |
| | $-0.126087$ | $-9.756467$ | $-4.256857$ | $-1.218841$ | Unstable |
| 3 | $-0.140625$ | $0.758532$ | $-1.063897$ | $-1.265625$ | Unstable |
| | $-0.140625$ | $-0.974322$ | $0.893176$ | $-1.265625$ | Saddle |
| | $-0.140625$ | $-10.040248$ | $-5.566084$ | $-1.265625$ | Unstable |
| 4 | $-0.162338$ | $0.750735$ | $-1.528228$ | $-1.352814$ | Unstable |
| | $-0.162338$ | $-1.065501$ | $1.278297$ | $-1.352814$ | Saddle |
| | $-0.162338$ | $-10.354800$ | $-7.816258$ | $-1.352814$ | Unstable |
| 5 | $-0.198276$ | $0.719651$ | $-2.433662$ | $-1.520115$ | Unstable |
| | $-0.198276$ | $-1.164127$ | $2.032577$ | $-1.520115$ | Saddle |
| | $-0.198276$ | $-10.710533$ | $-12.333056$ | $-1.520115$ | Unstable |
| 6 | $-0.269231$ | $0.665331$ | $-4.768395$ | $-1.884615$ | Unstable |
| | $-0.269231$ | $-1.275791$ | $3.983173$ | $-1.884615$ | Saddle |
| | $-0.269231$ | $-11.122459$ | $-24.188500$ | $-1.884615$ | Unstable |
| 7 | $-0.475000$ | $0.588250$ | $-15.797835$ | $-3.008333$ | Unstable |
| | $-0.475000$ | $-1.407792$ | $13.213405$ | $-3.008333$ | Saddle |
| | $-0.475000$ | $-11.612952$ | $-80.769522$ | $-3.008333$ | Unstable |
| 8 | $-8.500000$ | $0.489989$ | $-5437.180907$ | $-48.166667$ | Unstable |
| | $-8.500000$ | $-1.570012$ | $4555.705172$ | $-48.166667$ | Saddle |
| | $-8.500000$ | $-12.216652$ | $-28100.822498$ | $-48.166667$ | Unstable |

Table SM.13: Two loop $\overline{\text{MS}}$ scheme $SU(3)$ fixed points in the MAG for $0 \leq N_f \leq 8$.

| $N_f$ | $a_\infty$ | $\alpha_\infty$ | $\omega_1$ | $\omega_2$ | Infrared Stability |
|---|---|---|---|---|---|
| 9 | 0.416667 | 0.373983 | −14.338702 | 2.083333 | Saddle |
| | 0.416667 | −1.775685 | 12.032176 | 2.083333 | **Stable** |
| | 0.416667 | −12.989602 | −74.798981 | 2.083333 | Saddle |
| 10 | 0.175676 | 0.246040 | −2.897017 | 0.761261 | Saddle |
| | 0.175676 | −2.041475 | 2.432727 | 0.761261 | **Stable** |
| | 0.175676 | −14.027308 | −15.179420 | 0.761261 | Saddle |
| 11 | 0.098214 | 0.113996 | −1.082583 | 0.360119 | Saddle |
| | 0.098214 | −2.385628 | 0.909308 | 0.360119 | **Stable** |
| | 0.098214 | −15.503072 | −5.681145 | 0.360119 | Saddle |
| 12 | 0.060000 | −0.013878 | −0.515865 | 0.180000 | Saddle |
| | 0.060000 | −2.822900 | 0.434197 | 0.180000 | **Stable** |
| | 0.060000 | −17.757425 | −2.742662 | 0.180000 | Saddle |
| 13 | 0.037234 | −0.131066 | −0.275179 | 0.086879 | Saddle |
| | 0.037234 | −3.356225 | 0.233719 | 0.086879 | **Stable** |
| | 0.037234 | −21.537553 | −1.551277 | 0.086879 | Saddle |
| 14 | 0.022124 | −0.234163 | −0.150092 | 0.036873 | Saddle |
| | 0.022124 | −3.968278 | 0.130471 | 0.036873 | **Stable** |
| | 0.022124 | −28.797559 | −0.998010 | 0.036873 | Saddle |
| 15 | 0.011364 | −0.322652 | −0.073940 | 0.011364 | Saddle |
| | 0.011364 | −4.620179 | 0.067083 | 0.011364 | **Stable** |
| | 0.011364 | −46.665865 | −0.723403 | 0.011364 | Saddle |
| 16 | 0.003311 | −0.397788 | −0.021258 | 0.001104 | Saddle |
| | 0.003311 | −5.263519 | 0.020511 | 0.001104 | **Stable** |
| | 0.003311 | −138.990867 | −0.584233 | 0.001104 | Saddle |

Table SM.14: Two loop $\overline{\text{MS}}$ scheme $SU(3)$ fixed points in the MAG for $9 \leq N_f \leq 16$.

| $N_f$ | $a_\infty$ | $\alpha_\infty$ | $\omega_1$ | $\omega_2$ | Infrared Stability |
|---|---|---|---|---|---|
| 0 | - | - | - | - | - |
| 1 | - | - | - | - | - |
| 2 | - | - | - | - | - |
| 3 | - | - | - | - | - |
| 4 | - | - | - | - | - |
| 5 | - | - | - | - | - |
| 6 | 1.012686 | 1.066181 | $-936.218875$ | 40.841486 | Saddle |
| | 1.012686 | $-0.302082$ | 614.234192 | 40.841486 | **Stable** |
| | 1.012686 | $-3.789323$ | $-1653.674943$ | 40.841486 | Saddle |
| | 1.012686 | $-14.751998$ | 22323.155240 | 40.841486 | **Stable** |
| | $-0.212686$ | 1.392926 | 7.940517 | $-1.801486$ | Saddle |
| | $-0.212686$ | $-0.000035$ | $-4.952978$ | $-1.801486$ | Unstable |
| | $-0.212686$ | $-3.026215$ | 12.373281 | $-1.801486$ | Saddle |
| | $-0.212686$ | $-14.237125$ | $-205.889410$ | $-1.801486$ | Unstable |
| 7 | 0.195518 | 0.707879 | $-5.833518$ | 2.986261 | Saddle |
| | 0.195518 | $-0.392201$ | 4.297884 | 2.986261 | **Stable** |
| | 0.195518 | $-4.599116$ | $-14.711952$ | 2.986261 | Saddle |
| | 0.195518 | $-14.877015$ | 148.756038 | 2.986261 | **Stable** |
| | $-0.138506$ | 0.364044 | $-1.117819$ | $-1.498628$ | Unstable |
| | $-0.138506$ | 1.421878 | 1.592184 | $-1.498628$ | Saddle |
| | $-0.138506$ | $-2.878417$ | 3.513639 | $-1.498628$ | Saddle |
| | $-0.138506$ | $-13.933994$ | $-55.326741$ | $-1.498628$ | Unstable |
| 8 | 0.116505 | 0.382036 | $-1.072675$ | 1.329441 | Saddle |
| | 0.116505 | $-0.513620$ | 0.854383 | 1.329441 | **Stable** |
| | 0.116505 | $-5.459359$ | $-3.633976$ | 1.329441 | Saddle |
| | 0.116505 | $-14.732061$ | 27.031397 | 1.329441 | **Stable** |
| | $-0.114930$ | 0.730356 | $-0.416495$ | $-1.293733$ | Unstable |
| | $-0.114930$ | 1.345308 | 0.508494 | $-1.293733$ | Saddle |
| | $-0.114930$ | $-2.863163$ | 2.142604 | $-1.293733$ | Saddle |
| | $-0.114930$ | $-13.742599$ | $-30.937411$ | $-1.293733$ | Unstable |

Table SM.15: Three loop $\overline{\text{MS}}$ scheme $SU(3)$ fixed points in the MAG for $0 \leq N_f \leq 8$.

| $N_f$ | $a_\infty$ | $\alpha_\infty$ | $\omega_1$ | $\omega_2$ | Infrared Stability |
|---|---|---|---|---|---|
| 9 | 0.081803 | 0.110647 | −0.405334 | 0.737728 | Saddle |
| | 0.081803 | −0.777901 | 0.330414 | 0.737728 | **Stable** |
| | 0.081803 | −6.679483 | −1.414481 | 0.737728 | Saddle |
| | 0.081803 | −14.196635 | 6.776714 | 0.737728 | **Stable** |
| | −0.101786 | −2.890522 | 1.597345 | −1.142187 | Saddle |
| | −0.101786 | −13.591674 | −21.083596 | −1.142187 | Unstable |
| 10 | 0.060824 | −0.052653 | −0.267212 | 0.435887 | Saddle |
| | 0.060824 | −1.269137 | 0.209188 | 0.435887 | **Stable** |
| | 0.060824 | −9.374058 | −0.420956 | 0.435887 | Saddle |
| | 0.060824 | −12.260630 | 0.747665 | 0.435887 | **Stable** |
| | −0.093036 | −2.940420 | 1.307727 | −1.019824 | Saddle |
| | −0.093036 | −13.463534 | −15.814471 | −1.019824 | Unstable |
| 11 | 0.046039 | −0.141846 | −0.217669 | 0.258488 | Saddle |
| | 0.046039 | −1.943195 | 0.161834 | 0.258488 | **Stable** |
| | −0.086664 | −3.005152 | 1.129858 | −0.915931 | Saddle |
| | −0.086664 | −13.350466 | −12.562837 | −0.915931 | Unstable |
| 12 | 0.034607 | −0.201159 | −0.179724 | 0.147759 | Saddle |
| | 0.034607 | −2.691103 | 0.132673 | 0.147759 | **Stable** |
| | −0.081769 | −3.081276 | 1.011085 | −0.824922 | Saddle |
| | −0.081769 | −13.248370 | −10.373222 | −0.824922 | Unstable |
| 13 | 0.025191 | −0.250104 | −0.141632 | 0.077790 | Saddle |
| | 0.025191 | −3.414438 | 0.109473 | 0.077790 | **Stable** |
| | −0.077882 | −3.167303 | 0.927860 | −0.743563 | Saddle |
| | −0.077882 | −13.154889 | −8.810930 | −0.743563 | Unstable |
| 14 | 0.017070 | −0.296880 | −0.102009 | 0.034949 | Saddle |
| | 0.017070 | −4.074876 | 0.084750 | 0.034949 | **Stable** |
| | −0.074734 | −3.262849 | 0.868324 | −0.669865 | Saddle |
| | −0.074734 | −13.068691 | −7.651252 | −0.669865 | Unstable |
| 15 | 0.009818 | −0.345873 | −0.061234 | 0.011153 | Saddle |
| | 0.009818 | −4.684705 | 0.054889 | 0.011153 | **Stable** |
| | −0.072163 | −3.368312 | 0.826141 | −0.602581 | Saddle |
| | −0.072163 | −12.989180 | −6.767673 | −0.602581 | Unstable |
| 16 | 0.003162 | −0.400455 | −0.020208 | 0.001102 | Saddle |
| | 0.003162 | −5.273175 | 0.019487 | 0.001102 | **Stable** |
| | −0.070071 | −3.484791 | 0.798022 | −0.540976 | Saddle |
| | −0.070071 | −12.916396 | −6.085067 | −0.540976 | Unstable |

Table SM.16: Three loop $\overline{\text{MS}}$ scheme $SU(3)$ fixed points in the MAG for $9 \leq N_f \leq 16$.

| $N_f$ | $a_\infty$ | $\alpha_\infty$ | $\omega_1$ | $\omega_2$ | Infrared Stability |
|---|---|---|---|---|---|
| 0 | $-0.107843$ | 0.000000 | $-1.186275$ | 0.040441 | Saddle |
| | $-0.105855$ | $-0.246752$ | $-1.154314$ | $-0.041484$ | Unstable |
| | 0.062130 | $-4.318897$ | $-0.574164$ | $-1.250753$ | Unstable |
| 1 | $-0.115672$ | 0.000000 | $-1.195274$ | 0.028810 | Saddle |
| | $-0.114064$ | $-0.165331$ | $-1.170336$ | $-0.029275$ | Unstable |
| | 0.062019 | $-4.267792$ | $-0.654642$ | $-0.990548$ | Unstable |
| 2 | $-0.126087$ | 0.000000 | $-1.218841$ | 0.006990 | Saddle |
| | $-0.125625$ | $-0.037377$ | $-1.212026$ | $-0.007011$ | Unstable |
| | 0.061712 | $-4.213555$ | $-0.728921 + 0.213061i$ | $\omega_1^*$ | Unstable |
| 3 | $-0.140625$ | 0.000000 | $-1.265625$ | $-0.034607$ | Unstable |
| | $-0.143463$ | 0.169953 | $-1.304161$ | 0.034429 | Saddle |
| | 0.061160 | $-4.155784$ | $-0.632042 + 0.322776i$ | $\omega_1^*$ | Unstable |
| 4 | $-0.162338$ | 0.000000 | $-1.352814$ | $-0.119381$ | Unstable |
| | $-0.174520$ | 0.515163 | $-1.494419$ | 0.127390 | Saddle |
| | 0.060307 | $-4.094010$ | $-0.532910 + 0.382441i$ | $\omega_1^*$ | Unstable |
| 5 | $-0.198276$ | 0.000000 | $-1.520115$ | $-0.316643$ | Unstable |
| | $-0.227518$ | 0.990044 | $-1.771321$ | 0.493974 | Saddle |
| | 0.059079 | $-4.027704$ | $-0.432932 + 0.412726i$ | $\omega_1^*$ | Unstable |
| 6 | $-0.269231$ | 0.000000 | $-1.884615$ | $-0.908654$ | Unstable |
| | $-0.292980$ | 1.382181 | $-2.032332$ | 1.951358 | Saddle |
| | 0.057391 | $-3.956274$ | $-0.334091 + 0.419738i$ | $\omega_1^*$ | Unstable |
| 7 | $-0.475000$ | 0.000000 | $-3.008333$ | $-4.123594$ | Unstable |
| | $-0.363219$ | 1.642430 | $-2.388160$ | 5.508400 | Saddle |
| | 0.055142 | $-3.879093$ | $-0.239047 + 0.406243i$ | $\omega_1^*$ | Unstable |
| 8 | $-8.500000$ | 0.000000 | $-48.166667$ | $-1858.312500$ | Unstable |
| | $-0.442660$ | 1.824415 | $-2.886038$ | 12.321451 | Saddle |
| | 0.052219 | $-3.795565$ | $-0.151187 + 0.374262i$ | $\omega_1^*$ | Unstable |

Table SM.17: Two loop mMOM scheme $SU(3)$ fixed points in the linear covariant gauge for $0 \leq N_f \leq 8$.

| $N_f$ | $a_\infty$ | $\alpha_\infty$ | $\omega_1$ | $\omega_2$ | Infrared Stability |
|---|---|---|---|---|---|
| 9 | 0.416667 | 0.000000 | 2.083333 | $-6.171875$ | Saddle |
| | $-0.539147$ | 1.961289 | $-3.550561$ | 24.610495 | Saddle |
| | 0.048504 | $-3.705259$ | $-0.074519 + 0.326283i$ | $\omega_1^*$ | Unstable |
| 10 | 0.175676 | 0.000000 | 0.761261 | $-1.508081$ | Saddle |
| | $-0.664589$ | 2.070008 | $-4.451464$ | 47.114455 | Saddle |
| | 0.043898 | $-3.608171$ | $-0.013262 + 0.266097i$ | $\omega_1^*$ | Unstable |
| 11 | 0.098214 | 0.000000 | 0.360119 | $-0.651766$ | Saddle |
| | $-0.840152$ | 2.159858 | $-5.737401$ | 90.894147 | Saddle |
| | 0.038351 | $-3.505155$ | $0.029014 + 0.199294i$ | $\omega_1^*$ | **Stable** |
| 12 | 0.060000 | 0.000000 | 0.180000 | $-0.342900$ | Saddle |
| | $-1.110035$ | 2.236348 | $-7.733265$ | 185.978418 | Saddle |
| | 0.031919 | $-3.398484$ | $0.050721 + 0.133051i$ | $\omega_1^*$ | **Stable** |
| 13 | 0.037234 | 0.000000 | 0.086879 | $-0.193548$ | Saddle |
| | $-1.587436$ | 2.302966 | $-11.280327$ | 436.351715 | Saddle |
| | 0.024812 | $-3.292241$ | $0.053562 + 0.074726i$ | $\omega_1^*$ | **Stable** |
| 14 | 0.022124 | 0.000000 | 0.036873 | $-0.108001$ | Saddle |
| | $-2.679730$ | 2.362044 | $-19.413741$ | 1403.533918 | Saddle |
| | 0.017389 | $-3.191979$ | $0.042741 + 0.029067i$ | $\omega_1^*$ | **Stable** |
| 15 | 0.011364 | 0.000000 | 0.011364 | $-0.053170$ | Saddle |
| | $-7.837922$ | 2.415202 | $-57.856511$ | 13381.743380 | Saddle |
| | 0.010070 | $-3.103310$ | 0.013247 | 0.037372 | **Stable** |
| 16 | 0.003311 | 0.000000 | 0.001104 | $-0.015057$ | Saddle |
| | 9.180347 | 2.463608 | 69.003267 | 20251.528282 | **Stable** |
| | 0.003200 | $-3.030182$ | 0.001115 | 0.014086 | **Stable** |

Table SM.18: Two loop mMOM scheme $SU(3)$ fixed points in the linear covariant gauge for $9 \leq N_f \leq 16$.

| $N_f$ | $a_\infty$ | $\alpha_\infty$ | $\omega_1$ | $\omega_2$ | Infrared Stability |
|---|---|---|---|---|---|
| 0 | - | - | - | - | - |
| 1 | - | - | - | - | - |
| 2 | - | - | - | - | - |
| 3 | - | - | - | - | - |
| 4 | - | - | - | - | - |
| 5 | - | - | - | - | - |
| 6 | 2.090553 | 0.000000 | 142.898462 | $-3494.872556$ | Saddle |
| | $-0.238514$ | 0.000000 | $-1.860084$ | 4.395749 | Saddle |
| 7 | 0.146213 | 0.000000 | 2.137076 | $-2.038774$ | Saddle |
| | $-0.111799$ | 0.000000 | $-1.249470$ | 0.508332 | Saddle |
| | $-0.216296$ | 1.405281 | $-1.906928$ | $-9.391681$ | Unstable |
| | 0.571599 | 1.447646 | 13.701373 | 216.929038 | **Stable** |
| 8 | 0.089050 | 0.000000 | 1.014521 | $-0.712285$ | Saddle |
| | $-0.088127$ | 0.000000 | $-0.993594$ | 0.292921 | Saddle |
| | $-0.155260$ | 1.559339 | $-1.717697$ | $-4.352091$ | Unstable |
| | 0.247362 | 1.634268 | 4.420438 | 26.650609 | **Stable** |
| 9 | 0.064438 | 0.000000 | 0.594550 | $-0.406353$ | Saddle |
| | $-0.076226$ | 0.000000 | $-0.831986$ | 0.221749 | Saddle |
| | $-0.136153$ | 1.654875 | $-1.786908$ | $-3.255224$ | Unstable |
| | 0.188070 | 1.757395 | 3.267307 | 15.301919 | **Stable** |
| 10 | 0.049421 | 0.000000 | 0.368071 | $-0.275001$ | Saddle |
| | $-0.068767$ | 0.000000 | $-0.712626$ | 0.188239 | Saddle |
| | $-0.126675$ | 1.705766 | $-2.040132$ | $-2.570925$ | Unstable |
| | 0.162126 | 1.839694 | 2.847656 | 11.795069 | **Stable** |
| | $-0.080724$ | $-2.060465$ | $-0.145296$ | $-1.738450$ | Unstable |
| | $-0.298345$ | $-3.076568$ | 1.596306 | $-129.975607$ | Saddle |

Table SM.19: Three loop mMOM scheme $SU(3)$ fixed points in the linear covariant gauge for $0 \leq N_f \leq 10$.

| $N_f$ | $a_\infty$ | $\alpha_\infty$ | $\omega_1$ | $\omega_2$ | Infrared Stability |
|---|---|---|---|---|---|
| 11 | 0.038603 | 0.000000 | 0.227456 | −0.199789 | Saddle |
| | −0.063602 | 0.000000 | −0.617440 | 0.169879 | Saddle |
| | −0.121261 | 1.722122 | $-2.184400 + 0.454140i$ | $\omega_1^*$ | Unstable |
| | 0.147705 | 1.893386 | 2.651692 | 10.179310 | **Stable** |
| | −0.069841 | −1.892714 | −1.120278 | −0.155154 | Unstable |
| | 0.481048 | −3.475076 | 2.964235 | 647.235163 | **Stable** |
| | 0.042908 | −3.513882 | 0.075548 | 0.453675 | **Stable** |
| | 0.093269 | −3.787885 | −0.107796 | 5.240065 | Saddle |
| 12 | 0.029962 | 0.000000 | 0.134887 | −0.148283 | Saddle |
| | −0.059849 | 0.000000 | −0.538194 | 0.159119 | Saddle |
| | −0.118055 | 1.710461 | $-2.102292 + 0.627569i$ | $\omega_1^*$ | Unstable |
| | 0.138858 | 1.925597 | 2.556433 | 9.295937 | **Stable** |
| | −0.064075 | −1.818074 | −0.869020 | −0.153103 | Unstable |
| | 0.031269 | −3.323533 | 0.087686 | 0.196713 | **Stable** |
| 13 | 0.022535 | 0.000000 | 0.073340 | −0.108285 | Saddle |
| | −0.057086 | 0.000000 | −0.470621 | 0.152765 | Saddle |
| | −0.116254 | 1.674941 | $-2.037945 + 0.722389i$ | $\omega_1^*$ | Unstable |
| | 0.133279 | 1.940673 | 2.518423 | 8.776404 | **Stable** |
| | −0.060361 | −1.782949 | −0.720076 | −0.150242 | Unstable |
| | 0.023188 | −3.213214 | 0.065347 | 0.109665 | **Stable** |
| 14 | 0.015786 | 0.000000 | 0.033847 | −0.074248 | Saddle |
| | −0.055108 | 0.000000 | −0.412477 | 0.149278 | Saddle |
| | −0.115452 | 1.618154 | $-1.981140 + 0.773992i$ | $\omega_1^*$ | Unstable |
| | 0.129903 | 1.941314 | 2.519382 | 8.470959 | **Stable** |
| | −0.057872 | −1.767616 | −0.616468 | −0.148402 | Unstable |
| | 0.016146 | −3.138534 | 0.033290 | 0.070371 | **Stable** |
| 15 | 0.009383 | 0.000000 | 0.011019 | −0.043354 | Saddle |
| | −0.053849 | 0.000000 | −0.362870 | 0.147883 | Saddle |
| | −0.115430 | 1.541578 | $-1.925838 + 0.791362i$ | $\omega_1^*$ | Unstable |
| | 0.128198 | 1.929163 | 2.551400 | 8.310242 | **Stable** |
| | −0.056305 | −1.760923 | −0.538598 | −0.148093 | Unstable |
| | 0.009537 | −3.080626 | 0.011009 | 0.041625 | **Stable** |
| 16 | 0.003118 | 0.000000 | 0.001100 | −0.014158 | Saddle |
| | −0.053361 | 0.000000 | −0.322215 | 0.148216 | Saddle |
| | −0.116064 | 1.445778 | $-1.867539 + 0.774628i$ | $\omega_1^*$ | Unstable |
| | 0.127908 | 1.905111 | 2.611967 | 8.260995 | **Stable** |
| | −0.055582 | −1.754144 | −0.478462 | −0.149810 | Unstable |
| | 0.003138 | −3.027421 | 0.001100 | 0.013960 | **Stable** |

Table SM.20: Three loop mMOM scheme $SU(3)$ fixed points in the linear covariant gauge for $11 \leq N_f \leq 16$.

| $N_f$ | $a_\infty$ | $\alpha_\infty$ | $\omega_1$ | $\omega_2$ | Infrared Stability |
|---|---|---|---|---|---|
| 0 | $-0.051632$ | $0.000000$ | $-1.578535$ | $-0.025057$ | Unstable |
| | $-0.051667$ | $0.268566$ | $-1.590443$ | $0.024399$ | Saddle |
| | $0.036773$ | $-5.053693$ | $-0.627352 + 0.787987i$ | $\omega_1^*$ | Unstable |
| 1 | $-0.054722$ | $0.000000$ | $-1.560291$ | $-0.019551$ | Unstable |
| | $-0.054711$ | $0.202326$ | $-1.567144$ | $0.019160$ | Saddle |
| | $0.038349$ | $-4.937754$ | $-0.607785 + 0.779408i$ | $\omega_1^*$ | Unstable |
| 2 | $-0.058423$ | $0.000000$ | $-1.543240$ | $-0.012476$ | Unstable |
| | $-0.058374$ | $0.123754$ | $-1.545631$ | $0.012326$ | Saddle |
| | $0.040143$ | $-4.812086$ | $-0.583037 + 0.768878i$ | $\omega_1^*$ | Unstable |
| 3 | $-0.062975$ | $0.000000$ | $-1.527049$ | $-0.002672$ | Unstable |
| | $-0.062949$ | $0.025145$ | $-1.527009$ | $0.002665$ | Saddle |
| | $0.042220$ | $-4.674109$ | $-0.551034 + 0.755677i$ | $\omega_1^*$ | Unstable |
| 4 | $-0.068790$ | $0.000000$ | $-1.510323$ | $0.012327$ | Saddle |
| | $-0.069031$ | $-0.108665$ | $-1.513911$ | $-0.012428$ | Unstable |
| | $0.044679$ | $-4.519847$ | $-0.508253 + 0.738637i$ | $\omega_1^*$ | Unstable |
| 5 | $-0.076675$ | $0.000000$ | $-1.488354$ | $0.038480$ | Saddle |
| | $-0.078193$ | $-0.314403$ | $-1.514390$ | $-0.038962$ | Unstable |
| | $0.047680$ | $-4.342632$ | $-0.448016 + 0.715632i$ | $\omega_1^*$ | Unstable |
| 6 | $-0.088664$ | $0.000000$ | $-1.443371$ | $0.093924$ | Saddle |
| | $-0.098150$ | $-0.769414$ | $-1.574742$ | $-0.082131$ | Unstable |
| | $0.051496$ | $-4.129910$ | $-0.355581 + 0.682047i$ | $\omega_1^*$ | Unstable |
| 7 | $0.140341$ | $0.000000$ | $2.120767$ | $-2.432969$ | Saddle |
| | $-0.114912$ | $0.000000$ | $-1.243302$ | $0.281981$ | Saddle |
| | $-1.892434$ | $0.000000$ | $2685.392590$ | $-16846.680819$ | Saddle |
| | $-0.212055$ | $-0.317905$ | $-0.095240 + 2.578223i$ | $\omega_1^*$ | Unstable |
| | $0.056507$ | $-3.854897$ | $-0.191478 + 0.623841i$ | $\omega_1^*$ | Unstable |
| 8 | $0.072796$ | $0.000000$ | $0.966044$ | $-0.474778$ | Saddle |
| | $0.363423$ | $0.712602$ | $31.432482$ | $87.465149$ | **Stable** |
| | $0.060959$ | $-3.485534$ | $0.121193 + 0.476810i$ | $\omega_1^*$ | **Stable** |
| 9 | $0.054935$ | $0.000000$ | $0.582834$ | $-0.292463$ | Saddle |
| | $0.164446$ | $0.956855$ | $5.810601 + 4.718666i$ | $\omega_1^*$ | **Stable** |
| | $0.055612$ | $-3.212828$ | $0.297571 + 0.228641i$ | $\omega_1^*$ | **Stable** |
| 10 | $0.044230$ | $0.000000$ | $0.368153$ | $-0.218958$ | Saddle |
| | $0.132289$ | $1.038384$ | $3.245073 + 3.666805i$ | $\omega_1^*$ | **Stable** |
| | $0.046629$ | $-3.124397$ | $0.254470 + 0.096501i$ | $\omega_1^*$ | **Stable** |

Table SM.21: Four loop mMOM scheme $SU(3)$ fixed points in the linear covariant gauge for $0 \leq N_f \leq 10$.

| $N_f$ | $a_\infty$ | $\alpha_\infty$ | $\omega_1$ | $\omega_2$ | Infrared Stability |
|---|---|---|---|---|---|
| 11 | 0.036070 | 0.000000 | 0.229542 | $-0.173654$ | Saddle |
| | 0.118918 | 1.056106 | $2.251850 + 3.334076i$ | $\omega_1^*$ | **Stable** |
| | 0.038443 | $-3.114044$ | $0.186719 + 0.043680i$ | $\omega_1^*$ | **Stable** |
| 12 | 0.028981 | 0.000000 | 0.136117 | $-0.137930$ | Saddle |
| | $-0.073651$ | 0.000000 | $-0.536927$ | 0.369006 | Saddle |
| | $-0.234703$ | 0.000000 | 14.008441 | 20.110624 | **Stable** |
| | 0.112300 | 1.032029 | $1.603291 + 3.208646i$ | $\omega_1^*$ | **Stable** |
| | 0.030859 | $-3.126726$ | $0.129691 + 0.017731i$ | $\omega_1^*$ | **Stable** |
| 13 | 0.022329 | 0.000000 | 0.073621 | $-0.105460$ | Saddle |
| | $-0.061102$ | 0.000000 | $-0.481881$ | 0.252828 | Saddle |
| | $-0.640390$ | 0.000000 | 420.455573 | 1148.570890 | **Stable** |
| | 0.109339 | 0.972815 | $1.038648 + 3.154356i$ | $\omega_1^*$ | **Stable** |
| | 0.023543 | $-3.131342$ | 0.071258 | 0.099595 | **Stable** |
| 14 | 0.015838 | 0.000000 | 0.033786 | $-0.074090$ | Saddle |
| | 1.129859 | 0.000000 | $-2949.963120$ | 10907.035799 | Saddle |
| | $-0.053118$ | 0.000000 | $-0.403569$ | 0.200340 | Saddle |
| | 0.109027 | 0.877422 | $0.435182 + 3.095324i$ | $\omega_1^*$ | **Stable** |
| | 0.016445 | $-3.114255$ | 0.033121 | 0.070396 | **Stable** |
| 15 | 0.009431 | 0.000000 | 0.010979 | $-0.043538$ | Saddle |
| | 0.315742 | 0.000000 | $-78.894602$ | 58.143613 | Saddle |
| | $-0.047172$ | 0.000000 | $-0.325416$ | 0.170005 | Saddle |
| | 0.111199 | 0.736988 | $-0.328756 + 2.911875i$ | $\omega_1^*$ | Unstable |
| | 0.009636 | $-3.076936$ | 0.010922 | 0.041922 | **Stable** |
| 16 | 0.003121 | 0.000000 | 0.001099 | $-0.014174$ | Saddle |
| | 0.190288 | 0.000000 | $-20.905119$ | 5.336964 | Saddle |
| | $-0.042321$ | 0.000000 | $-0.251048$ | 0.150031 | Saddle |
| | 0.116265 | 0.528607 | $-1.453173 + 2.166313i$ | $\omega_1^*$ | Unstable |
| | $-0.048949$ | $-2.446819$ | $-0.103392$ | $-0.671851$ | Unstable |
| | 0.003143 | $-3.027354$ | 0.001099 | 0.013980 | **Stable** |
| | $-0.131854$ | $-3.629565$ | 0.969650 | $-55.360457$ | Saddle |

Table SM.22: Four loop mMOM scheme $SU(3)$ fixed points in the linear covariant gauge for $11 \leq N_f \leq 16$.

| $N_f$ | $a_\infty$ | $\alpha_\infty$ | $\omega_1$ | $\omega_2$ | Infrared Stability |
|---|---|---|---|---|---|
| 0 | - | - | - | - | - |
| 1 | - | - | - | - | - |
| 2 | - | - | - | - | - |
| 3 | - | - | - | - | - |
| 4 | - | - | - | - | - |
| 5 | - | - | - | - | - |
| 6 | 0.089938 | 0.000000 | 3.559095 | $-1.647315$ | Saddle |
| | $-0.063886$ | 0.000000 | $-1.353571$ | 0.244791 | Saddle |
| 7 | 0.060257 | 0.000000 | 1.499477 | $-0.386721$ | Saddle |
| | $-0.056463$ | 0.000000 | $-1.165502$ | 0.153501 | Saddle |
| | $-0.058573$ | $-2.200995$ | $-1.888553$ | $-0.117042$ | Unstable |
| | 0.058382 | $-3.630919$ | 0.251450 | 2.160916 | **Stable** |
| 8 | 0.050162 | 0.000000 | 0.928758 | $-0.249221$ | Saddle |
| | $-0.053751$ | 0.000000 | $-1.029178$ | 0.132343 | Saddle |
| | 0.178070 | 1.377827 | 4.732069 | 173.467310 | **Stable** |
| | 8.186013 | 1.470023 | $-7742265.147766$ | 32959305743.666241 | Saddle |
| | $-0.054158$ | $-1.806074$ | $-1.237300$ | $-0.122990$ | Unstable |
| | 0.047937 | $-3.192836$ | 0.742629 | 0.261331 | **Stable** |
| 9 | 0.044015 | 0.000000 | 0.608228 | $-0.202835$ | Saddle |
| | $-0.053101$ | 0.000000 | $-0.919546$ | 0.128285 | Saddle |
| | 0.116454 | 1.315030 | 3.633119 | 18.970870 | **Stable** |
| | $-0.223975$ | 1.534604 | $-10.705283$ | $-427.049335$ | Unstable |
| | $-0.053177$ | $-1.706875$ | $-1.044788$ | $-0.119349$ | Unstable |
| | 0.043123 | $-3.003521$ | 0.510250 | 0.209211 | **Stable** |
| 10 | 0.039122 | 0.000000 | 0.391910 | $-0.178382$ | Saddle |
| | $-0.054160$ | 0.000000 | $-0.825093$ | 0.132420 | Saddle |
| | 0.103319 | 1.204261 | $5.029211 + 2.081153i$ | $\omega_1^*$ | **Stable** |
| | $-0.203351$ | 1.411529 | $-15.725593$ | $-161.694252$ | Unstable |
| | $-0.053856$ | $-1.713426$ | $-0.923223$ | $-0.119066$ | Unstable |
| | 0.039060 | $-2.975110$ | 0.348737 | 0.178474 | **Stable** |

Table SM.23: Five loop mMOM scheme $SU(3)$ fixed points in the linear covariant gauge for $0 \leq N_f \leq 10$.

| $N_f$ | $a_\infty$ | $\alpha_\infty$ | $\omega_1$ | $\omega_2$ | Infrared Stability |
|---|---|---|---|---|---|
| 11 | 0.034349 | 0.000000 | 0.239411 | $-0.158660$ | Saddle |
| | $-0.057838$ | 0.000000 | $-0.734981$ | 0.143787 | Saddle |
| | 0.096774 | 1.021248 | $2.047620 + 3.312087i$ | $\omega_1^*$ | **Stable** |
| | $-0.167440$ | 1.163708 | $-11.406531 + 16.028737i$ | $\omega_1^*$ | Unstable |
| | $-0.056435$ | $-1.791754$ | $-0.826390$ | $-0.118962$ | Unstable |
| | 0.034890 | $-3.025124$ | 0.223755 | 0.153415 | **Stable** |
| 12 | 0.028976 | 0.000000 | 0.136151 | $-0.135918$ | Saddle |
| | $-0.073254$ | 0.000000 | $-0.541149$ | 0.159805 | Saddle |
| | $-0.253169$ | 0.000000 | 17.040748 | $-73.735406$ | Saddle |
| | $-4.094843$ | 0.000000 | $-1456472.823034$ | $-109856191.029418$ | Unstable |
| | $-0.112269$ | 0.468605 | $0.520475 + 1.296970i$ | $\omega_1^*$ | **Stable** |
| | 0.092477 | 0.737912 | $0.042881 + 2.607927i$ | $\omega_1^*$ | **Stable** |
| | $-0.062875$ | $-2.036433$ | $-0.759535$ | $-0.103491$ | Unstable |
| | 0.029873 | $-3.093637$ | 0.119065 | 0.140522 | **Stable** |
| | $-0.093652$ | $-3.231818$ | 0.342242 | $-13.241761$ | Saddle |
| | $-0.187151$ | $-3.498850$ | $-6.832474$ | $-394.991840$ | Unstable |
| 13 | 0.022746 | 0.000000 | 0.071625 | $-0.107263$ | Saddle |
| | 0.103541 | 0.000000 | $-5.382778$ | 0.691961 | Saddle |
| | 0.088935 | 0.273310 | $-2.008768$ | $-0.682213$ | Unstable |
| | 0.023575 | $-3.130751$ | 0.068903 | 0.101307 | **Stable** |
| 14 | 0.016067 | 0.000000 | 0.032997 | $-0.075242$ | Saddle |
| | 0.073378 | 0.000000 | $-2.190706$ | $-0.257694$ | Unstable |
| | 0.083341 | $-0.745879$ | $-3.737705$ | 0.245837 | Saddle |
| | 0.016555 | $-3.118834$ | 0.032707 | 0.070665 | **Stable** |
| 15 | 0.009476 | 0.000000 | 0.010888 | $-0.043759$ | Saddle |
| | 0.062696 | 0.000000 | $-1.652417$ | $-0.333851$ | Unstable |
| | 0.009660 | $-3.078166$ | 0.010878 | 0.041996 | **Stable** |
| | 0.057124 | $-3.612651$ | $-0.513955$ | 0.630062 | Saddle |
| 16 | 0.003122 | 0.000000 | 0.001098 | $-0.014178$ | Saddle |
| | 0.057710 | 0.000000 | $-1.551958$ | $-0.359307$ | Unstable |
| | 0.003143 | $-3.027377$ | 0.001098 | 0.013982 | **Stable** |
| | 0.050584 | $-3.866561$ | $-0.515577$ | 0.687634 | Saddle |

Table SM.24: Five loop mMOM scheme $SU(3)$ fixed points in the linear covariant gauge for $11 \leq N_f \leq 16$.

| $N_f$ | $a_\infty$ | $\alpha_\infty$ | $\omega_1$ | $\omega_2$ | Infrared Stability |
|---|---|---|---|---|---|
| 0 | −0.107843 | 0.000000 | −1.186275 | 1.105084 | Saddle |
| | −0.107843 | −3.712914 | −3.045728 | −1.186275 | Unstable |
| 1 | −0.115672 | 0.000000 | −1.195274 | 1.041287 | Saddle |
| | −0.115672 | −3.511157 | −2.880505 | −1.195274 | Unstable |
| 2 | −0.126087 | 0.000000 | −1.218841 | 0.981252 | Saddle |
| | −0.126087 | −3.293533 | −2.733427 | −1.218841 | Unstable |
| 3 | −0.140625 | 0.000000 | −1.265625 | 0.922028 | Saddle |
| | −0.140625 | −3.053003 | −2.602916 | −1.265625 | Unstable |
| 4 | −0.162338 | 0.000000 | −1.352814 | 0.854357 | Saddle |
| | −0.162338 | −2.775527 | −2.477453 | −1.352814 | Unstable |
| 5 | −0.198276 | 0.000000 | −1.520115 | 0.744998 | Saddle |
| | −0.198276 | −2.426918 | −2.298849 | −1.520115 | Unstable |
| 6 | −0.269231 | 0.000000 | −1.884615 | 0.435343 | Saddle |
| | −0.269231 | −1.878058 | −1.707425 | −1.884615 | Unstable |
| 7 | −0.475000 | 0.000000 | −3.008333 | −1.515327 | Unstable |
| | −0.475000 | 2.375212 | 7.999731 | −3.008333 | Saddle |
| 8 | −8.500000 | 0.000000 | −1420.464120 | −48.166667 | Unstable |
| | −8.500000 | 2.991141 | 5932.485454 | −48.166667 | Saddle |
| 9 | 0.416667 | 0.000000 | −5.817419 | 2.083333 | Saddle |
| | 0.416667 | 3.457480 | 23.518988 | 2.083333 | **Stable** |
| 10 | 0.175676 | 0.000000 | −1.523369 | 0.761261 | Saddle |
| | 0.175676 | 3.922004 | 6.305961 | 0.761261 | **Stable** |
| 11 | 0.098214 | 0.000000 | −0.666726 | 0.360119 | Saddle |
| | 0.098214 | 4.460256 | 2.928346 | 0.360119 | **Stable** |
| 12 | 0.060000 | 0.000000 | −0.346950 | 0.180000 | Saddle |
| | 0.060000 | 5.152191 | 1.669764 | 0.180000 | **Stable** |
| 13 | 0.037234 | 0.000000 | −0.192463 | 0.086879 | Saddle |
| | 0.037234 | 6.124282 | 1.051979 | 0.086879 | **Stable** |
| 14 | 0.022124 | 0.000000 | −0.105959 | 0.036873 | Saddle |
| | 0.022124 | 7.642310 | 0.690431 | 0.036873 | **Stable** |
| | 0.022124 | −3.669491 | 0.072963 | 0.036873 | **Stable** |
| | 0.022124 | −6.861707 | −0.174940 | 0.036873 | Saddle |
| 15 | 0.011364 | 0.000000 | −0.052003 | 0.011364 | Saddle |
| | 0.011364 | 10.490230 | 0.440698 | 0.011364 | **Stable** |
| | 0.011364 | −3.217291 | 0.047339 | 0.011364 | **Stable** |
| | 0.011364 | −10.606272 | −0.240184 | 0.011364 | Saddle |
| 16 | 0.003311 | 0.000000 | −0.014888 | 0.001104 | Saddle |
| | 0.003311 | 19.559143 | 0.217309 | 0.001104 | **Stable** |
| | 0.003311 | −3.040393 | 0.014626 | 0.001104 | **Stable** |
| | 0.003311 | −20.296527 | −0.172184 | 0.001104 | Saddle |

Table SM.25: Two loop RI′ scheme $SU(3)$ fixed points in the linear covariant gauge for $0 \leq N_f \leq 16$.

| $N_f$ | $a_\infty$ | $\alpha_\infty$ | $\omega_1$ | $\omega_2$ | Infrared Stability |
|---|---|---|---|---|---|
| 0 | - | - | - | - | - |
| 1 | - | - | - | - | - |
| 2 | - | - | - | - | - |
| 3 | - | - | - | - | - |
| 4 | - | - | - | - | - |
| 5 | - | - | - | - | - |
| 6 | 1.012686 | 0.000000 | $-206.901313$ | 40.841486 | Saddle |
| | $-0.212686$ | 0.000000 | $-1.801486$ | 2.245456 | Saddle |
| | 1.012686 | 0.861545 | 313.847945 | 40.841486 | **Stable** |
| | $-0.212686$ | 0.927631 | $-3.418920$ | $-1.801486$ | Unstable |
| 7 | 0.195518 | 0.000000 | $-5.494140$ | 2.986261 | Saddle |
| | $-0.138506$ | 0.000000 | $-1.498628$ | 1.733095 | Saddle |
| | 0.195518 | 1.671843 | 12.600209 | 2.986261 | **Stable** |
| | $-0.138506$ | 1.574246 | $-3.533709$ | $-1.498628$ | Unstable |
| 8 | 0.116505 | 0.000000 | $-1.969208$ | 1.329441 | Saddle |
| | $-0.114930$ | 0.000000 | $-1.293733$ | 1.374533 | Saddle |
| | 0.116505 | 2.038116 | 5.178099 | 1.329441 | **Stable** |
| | $-0.114930$ | 1.794255 | $-3.013204$ | $-1.293733$ | Unstable |
| 9 | 0.081803 | 0.000000 | $-0.961698$ | 0.737728 | Saddle |
| | $-0.101786$ | 0.000000 | $-1.142187$ | 1.073551 | Saddle |
| | 0.081803 | 2.306390 | 2.796491 | 0.737728 | **Stable** |
| | $-0.101786$ | 1.868912 | $-2.402724$ | $-1.142187$ | Unstable |
| | $-0.101786$ | $-4.778438$ | $-2.388475$ | $-1.142187$ | Unstable |
| | $-0.101786$ | $-5.931431$ | 4.706855 | $-1.142187$ | Saddle |
| 10 | 0.060824 | 0.000000 | $-0.527751$ | 0.435887 | Saddle |
| | $-0.093036$ | 0.000000 | $-1.019824$ | 0.807886 | Saddle |
| | 0.060824 | 2.571364 | 1.711723 | 0.435887 | **Stable** |
| | $-0.093036$ | 1.850084 | $-1.796257$ | $-1.019824$ | Unstable |
| | $-0.093036$ | $-4.300844$ | $-2.697831$ | $-1.019824$ | Unstable |
| | $-0.093036$ | $-6.641878$ | 10.574267 | $-1.019824$ | Saddle |

Table SM.26: Three loop RI′ scheme $SU(3)$ fixed points in the linear covariant gauge for $0 \leq N_f \leq 10$.

| $N_f$ | $a_\infty$ | $\alpha_\infty$ | $\omega_1$ | $\omega_2$ | Infrared Stability |
|---|---|---|---|---|---|
| 11 | 0.046039 | 0.000000 | −0.309329 | 0.258488 | Saddle |
| | −0.086664 | 0.000000 | −0.915931 | 0.566924 | Saddle |
| | 0.046039 | 2.896474 | 1.149625 | 0.258488 | **Stable** |
| | −0.086664 | 1.742251 | −1.218396 | −0.915931 | Unstable |
| | −0.086664 | −3.935350 | −2.212275 | −0.915931 | Unstable |
| | −0.086664 | −7.132297 | 14.520495 | −0.915931 | Saddle |
| 12 | 0.034607 | 0.000000 | −0.190370 | 0.147759 | Saddle |
| | −0.081769 | 0.000000 | −0.824922 | 0.344313 | Saddle |
| | 0.034607 | 3.348119 | 0.838553 | 0.147759 | **Stable** |
| | −0.081769 | 1.510869 | −0.681446 | −0.824922 | Unstable |
| | −0.081769 | −3.537470 | −1.563999 | −0.824922 | Unstable |
| | −0.081769 | −7.532434 | 17.629385 | −0.824922 | Saddle |
| 13 | 0.025191 | 0.000000 | −0.121177 | 0.077790 | Saddle |
| | −0.077882 | 0.000000 | −0.743563 | 0.135596 | Saddle |
| | 0.025191 | 4.017183 | 0.652575 | 0.077790 | **Stable** |
| | 0.025191 | −4.223426 | 0.076471 | 0.077790 | **Stable** |
| | 0.025191 | −5.862951 | −0.156399 | 0.077790 | Saddle |
| | −0.077882 | 0.999964 | −0.213717 | −0.743563 | Unstable |
| | −0.077882 | −2.995329 | −0.844259 | −0.743563 | Unstable |
| | −0.077882 | −7.876904 | 20.237808 | −0.743563 | Saddle |
| 14 | 0.017070 | 0.000000 | −0.076742 | 0.034949 | Saddle |
| | −0.074734 | 0.000000 | −0.669865 | −0.062848 | Unstable |
| | 0.017070 | 5.077386 | 0.520008 | 0.034949 | **Stable** |
| | 0.017070 | −3.421636 | 0.069422 | 0.034949 | **Stable** |
| | 0.017070 | −7.516002 | −0.323899 | 0.034949 | Saddle |
| | −0.074734 | −8.181557 | 22.516571 | −0.669865 | Saddle |
| 15 | 0.009818 | 0.000000 | −0.043455 | 0.011153 | Saddle |
| | −0.072163 | 0.000000 | −0.602581 | −0.254435 | Unstable |
| | 0.009818 | 7.046555 | 0.391900 | 0.011153 | **Stable** |
| | 0.009818 | −3.136331 | 0.041592 | 0.011153 | **Stable** |
| | 0.009818 | −9.659469 | −0.307509 | 0.011153 | Saddle |
| | −0.072163 | −8.455255 | 24.576517 | −0.602581 | Saddle |
| 16 | 0.003162 | 0.000000 | −0.014147 | 0.001102 | Saddle |
| | −0.070071 | 0.000000 | −0.540976 | −0.442903 | Unstable |
| | 0.003162 | 13.288060 | 0.218266 | 0.001102 | **Stable** |
| | 0.003162 | −3.029389 | 0.013951 | 0.001102 | **Stable** |
| | 0.003162 | −15.948011 | −0.192931 | 0.001102 | Saddle |
| | −0.070071 | −8.703479 | 26.506734 | −0.540976 | Saddle |

Table SM.27: Three loop RI′ scheme $SU(3)$ fixed points in the linear covariant gauge for $11 \leq N_f \leq 16$.

| $N_f$ | $a_\infty$ | $\alpha_\infty$ | $\omega_1$ | $\omega_2$ | Infrared Stability |
|---|---|---|---|---|---|
| 0 | $-0.072415$ | 0.000000 | $-1.862385$ | 6.707519 | Saddle |
| | $-0.072415$ | $-4.600204$ | $-17.786839$ | $-1.862385$ | Unstable |
| 1 | $-0.076801$ | 0.000000 | $-1.850154$ | 6.012601 | Saddle |
| | $-0.076801$ | $-4.393277$ | $-15.343998$ | $-1.850154$ | Unstable |
| 2 | $-0.082085$ | 0.000000 | $-1.841408$ | 5.234577 | Saddle |
| | $-0.082085$ | $-4.138653$ | $-12.574374$ | $-1.841408$ | Unstable |
| 3 | $-0.088492$ | 0.000000 | $-1.833095$ | 4.297232 | Saddle |
| | $-0.088492$ | $-3.795342$ | $-9.273097$ | $-1.833095$ | Unstable |
| 4 | $-0.096211$ | 0.000000 | $-1.816819$ | 3.078500 | Saddle |
| | $-0.096211$ | $-3.235659$ | $-5.277632$ | $-1.816819$ | Unstable |
| 5 | $-0.105089$ | 0.000000 | $-1.772958$ | 1.429826 | Saddle |
| | $-0.105089$ | $-1.827165$ | $-1.389068$ | $-1.772958$ | Unstable |
| 6 | $-0.113620$ | 0.000000 | $-1.667057$ | $-0.587698$ | Unstable |
| | $-0.113620$ | 0.445894 | 0.724235 | $-1.667057$ | Saddle |
| 7 | $-0.116983$ | 0.000000 | $-1.971623$ | $-1.483338$ | Unstable |
| | $-0.116983$ | 1.046355 | 3.702061 | $-1.483338$ | Saddle |
| 8 | 0.123312 | 0.000000 | $-6.471485$ | 1.323045 | Saddle |
| | 1.142863 | 0.000000 | $-32282.812368$ | $-610.561252$ | Unstable |
| | $-0.109864$ | 0.000000 | $-1.427227$ | $-1.290397$ | Unstable |
| | 0.123312 | 1.454078 | 15.251556 | 1.323045 | **Stable** |
| | 1.142863 | 1.310571 | 71125.424907 | $-610.561252$ | Saddle |
| | $-0.109864$ | 1.111817 | 2.973272 | $-1.290397$ | Saddle |

Table SM.28: Four loop RI′ scheme $SU(3)$ fixed points in the linear covariant gauge for $0 \leq N_f \leq 8$.

| $N_f$ | $a_\infty$ | $\alpha_\infty$ | $\omega_1$ | $\omega_2$ | Infrared Stability |
|---|---|---|---|---|---|
| 9 | 0.085291 | 0.000000 | −1.758067 | 0.732193 | Saddle |
| | 0.962002 | 0.000000 | −12210.075742 | −542.394739 | Unstable |
| | −0.096487 | 0.000000 | −1.131329 | −0.212908 | Unstable |
| | 0.085291 | 1.577736 | 4.588481 | 0.732193 | **Stable** |
| | 0.962002 | 1.217379 | 26554.397667 | −542.394739 | Saddle |
| | 0.962002 | −4.254154 | 19087.264647 | −542.394739 | Saddle |
| | 0.962002 | −4.785856 | −30200.511682 | −542.394739 | Unstable |
| | −0.096487 | 0.621256 | 0.346799 | −1.131329 | Saddle |
| | −0.096487 | −2.749462 | 0.764590 | −1.131329 | Saddle |
| | −0.096487 | −4.830332 | −5.801724 | −1.131329 | Unstable |
| 10 | 0.064860 | 0.000000 | −0.655285 | 0.426703 | Saddle |
| | 0.446940 | 0.000000 | −212.501737 | −72.410221 | Unstable |
| | −0.083591 | 0.000000 | −0.984127 | 0.470548 | Saddle |
| | 0.064860 | 1.682620 | 1.914947 | 0.426703 | **Stable** |
| | 0.446940 | 0.781736 | 362.899110 | −72.410221 | Saddle |
| | 0.446940 | −2.887919 | 979.733760 | −72.410221 | Saddle |
| | 0.446940 | −5.607503 | −11960.577226 | −72.410221 | Unstable |
| | −0.083591 | −5.417047 | −10.236509 | −0.984127 | Unstable |
| 11 | 0.049832 | 0.000000 | −0.287141 | 0.249017 | Saddle |
| | 0.262159 | 0.000000 | −18.805627 | 34.873440 | Saddle |
| | −0.072993 | 0.000000 | −0.843350 | 0.699456 | Saddle |
| | 0.049832 | 1.886786 | 1.015151 | 0.249017 | **Stable** |
| | 0.049832 | −4.300134 | 0.244439 | 0.249017 | **Stable** |
| | 0.049832 | −4.929912 | −0.395983 | 0.249017 | Saddle |
| | 0.262159 | −5.991881 | −2607.263240 | −18.805627 | Unstable |
| | −0.072993 | −5.680263 | −8.765422 | −0.843350 | Unstable |
| 12 | 0.037434 | 0.000000 | −0.159018 | 0.141164 | Saddle |
| | 0.182641 | 0.000000 | −8.151111 | 25.940281 | Saddle |
| | −0.064423 | 0.000000 | −0.711375 | 0.705403 | Saddle |
| | 0.037434 | 2.309301 | 0.737790 | 0.141164 | **Stable** |
| | 0.037434 | −3.483133 | 0.186636 | 0.141164 | **Stable** |
| | 0.037434 | −5.645069 | −0.837385 | 0.141164 | Saddle |
| | 0.182641 | −6.272709 | −904.154985 | −8.151111 | Unstable |
| | −0.064423 | −5.787251 | −6.012934 | −0.711375 | Unstable |

Table SM.29: Four loop RI′ scheme $SU(3)$ fixed points in the linear covariant gauge for $9 \leq N_f \leq 12$.

| $N_f$ | $a_\infty$ | $\alpha_\infty$ | $\omega_1$ | $\omega_2$ | Infrared Stability |
|---|---|---|---|---|---|
| 13 | 0.026853 | 0.000000 | −0.107236 | 0.074565 | Saddle |
| | 0.141687 | 0.000000 | −4.907150 | 16.860752 | Saddle |
| | −0.057340 | 0.000000 | −0.589242 | 0.618631 | Saddle |
| | 0.026853 | 2.998702 | 0.649158 | 0.074565 | **Stable** |
| | 0.026853 | −3.183587 | 0.108380 | 0.074565 | **Stable** |
| | 0.026853 | −6.233305 | −0.648901 | 0.074565 | Saddle |
| | 0.141687 | −6.499993 | −434.503642 | −4.907150 | Unstable |
| | −0.057340 | −5.744670 | −3.506902 | −0.589242 | Unstable |
| 14 | 0.017793 | 0.000000 | −0.073867 | 0.033906 | Saddle |
| | 0.117756 | 0.000000 | −3.633611 | 11.961869 | Saddle |
| | −0.051298 | 0.000000 | −0.476616 | 0.501442 | Saddle |
| | 0.017793 | 4.034989 | 0.566596 | 0.033906 | **Stable** |
| | 0.017793 | −3.110067 | 0.070748 | 0.033906 | **Stable** |
| | 0.017793 | −7.141091 | −0.488575 | 0.033906 | Saddle |
| | 0.117756 | −6.692429 | −258.053045 | −3.633611 | Unstable |
| | −0.051298 | −5.502602 | −1.777653 | −0.476616 | Unstable |
| 15 | 0.010001 | 0.000000 | −0.043484 | 0.010988 | Saddle |
| | 0.102368 | 0.000000 | −3.051413 | 9.175760 | Saddle |
| | −0.045958 | 0.000000 | −0.372592 | 0.383263 | Saddle |
| | 0.010001 | 5.844876 | 0.438692 | 0.010988 | **Stable** |
| | 0.010001 | −3.074901 | 0.041840 | 0.010988 | **Stable** |
| | 0.010001 | −8.893650 | −0.370397 | 0.010988 | Saddle |
| | 0.102368 | −6.858264 | −175.161341 | −3.051413 | Unstable |
| | −0.045958 | −5.018562 | −0.939104 | −0.372592 | Unstable |
| 16 | 0.003170 | 0.000000 | −0.014174 | 0.001099 | Saddle |
| | 0.091700 | 0.000000 | −2.761435 | 7.417104 | Saddle |
| | −0.041033 | 0.000000 | −0.276077 | 0.278076 | Saddle |
| | 0.003170 | 11.407063 | 0.243998 | 0.001099 | **Stable** |
| | 0.003170 | −3.027317 | 0.013978 | 0.001099 | **Stable** |
| | 0.003170 | −14.459972 | −0.220432 | 0.001099 | Saddle |
| | 0.091700 | −7.001486 | −129.137055 | −2.761435 | Unstable |
| | −0.041033 | −4.418610 | −0.597616 | −0.276077 | Unstable |

Table SM.30: Four loop RI′ scheme $SU(3)$ fixed points in the linear covariant gauge for $13 \leq N_f \leq 16$.

| $N_f$ | $a_\infty$ | $\alpha_\infty$ | $\omega_1$ | $\omega_2$ | Infrared Stability |
|---|---|---|---|---|---|
| 0 | - | - | - | - | - |
| 1 | - | - | - | - | - |
| 2 | - | - | - | - | - |
| 3 | - | - | - | - | - |
| 4 | - | - | - | - | - |
| 5 | $-0.125111$ | 0.000000 | $-7.135574$ | $-1.547127$ | Unstable |
| | $-0.279400$ | 0.000000 | $-480.049936$ | 22.006345 | Saddle |
| | $-0.125111$ | $-0.642827$ | 6.119476 | $-1.547127$ | Saddle |
| | $-0.279400$ | $-0.733474$ | 408.389524 | 22.006345 | **Stable** |
| 6 | $-0.113974$ | 0.000000 | $-1.664633$ | 6.849098 | Saddle |
| | $-9.122662$ | 0.000000 | 17178776.772536 | 24421135408.894386 | **Stable** |
| | $-0.113974$ | 0.816276 | $-11.364517$ | $-1.664633$ | Unstable |
| | $-9.122662$ | 0.768937 | $-38741697330.861984$ | 17178776.772536 | Saddle |
| 7 | - | - | - | - | - |
| 8 | - | - | - | - | - |
| 9 | - | - | - | - | - |
| 10 | - | - | - | - | - |
| 11 | - | - | - | - | - |
| 12 | - | - | - | - | - |
| 13 | 0.032315 | 0.000000 | $-0.070465$ | 0.036682 | Saddle |
| | 0.041343 | 0.000000 | $-0.072312$ | 0.059503 | Saddle |
| | 0.032315 | 2.234097 | 0.611895 | 0.036682 | **Stable** |
| | 0.032315 | $-1.726095$ | 0.068845 | 0.036682 | **Stable** |
| | 0.032315 | $-6.244816$ | $-1.933961$ | 0.036682 | Saddle |
| | 0.041343 | $-6.275659$ | $-5.660794$ | $-0.072312$ | Unstable |
| 14 | 0.018526 | 0.000000 | $-0.073887$ | 0.031152 | Saddle |
| | 0.046357 | 0.000000 | $-0.365291$ | 0.312954 | Saddle |
| | 0.018526 | 3.542651 | 0.651214 | 0.031152 | **Stable** |
| | 0.018526 | $-2.998799$ | 0.069622 | 0.031152 | **Stable** |
| | 0.018526 | $-6.916493$ | $-0.619130$ | 0.031152 | Saddle |
| | 0.046357 | $-6.408426$ | $-10.473152$ | $-0.365291$ | Unstable |
| 15 | 0.010078 | 0.000000 | $-0.043744$ | 0.010828 | Saddle |
| | 0.047107 | 0.000000 | $-0.587861$ | 0.381455 | Saddle |
| | 0.010078 | 5.303059 | 0.492938 | 0.010828 | **Stable** |
| | 0.010078 | $-3.071076$ | 0.041973 | 0.010828 | **Stable** |
| | 0.010078 | $-8.551579$ | $-0.425420$ | 0.010828 | Saddle |
| | 0.047107 | $-6.462481$ | $-10.742283$ | $-0.587861$ | Unstable |
| 16 | 0.003171 | 0.000000 | $-0.014178$ | 0.001098 | Saddle |
| | 0.046999 | 0.000000 | $-0.780464$ | 0.324491 | Saddle |
| | 0.003171 | 10.552329 | 0.271776 | 0.001098 | **Stable** |
| | 0.003171 | $-3.027350$ | 0.013982 | 0.001098 | **Stable** |
| | 0.003171 | $-13.778184$ | $-0.247828$ | 0.001098 | Saddle |
| | 0.046999 | $-6.454812$ | $-8.786639$ | $-0.780464$ | Unstable |

Table SM.31: Five loop RI′ scheme $SU(3)$ fixed points in the linear covariant gauge for $0 \leq N_f \leq 16$.

| $N_f$ | $a_\infty$ | $\alpha_\infty$ | $\omega_1$ | $\omega_2$ | Infrared Stability |
|---|---|---|---|---|---|
| 0 | $-0.107843$ | $0.000000$ | $-1.186275$ | $-0.297090$ | Unstable |
| | $-0.143876$ | $1.757109$ | $-1.687527$ | $0.505026$ | Saddle |
| | $0.017885$ | $-7.839379$ | $-0.278608 + 0.065837i$ | $\omega_1^*$ | Unstable |
| 1 | $-0.115672$ | $0.000000$ | $-1.195274$ | $-0.319677$ | Unstable |
| | $-0.148772$ | $1.599774$ | $-1.613854$ | $0.533241$ | Saddle |
| | $0.018817$ | $-7.642767$ | $-0.276294 + 0.084853i$ | $\omega_1^*$ | Unstable |
| 2 | $-0.126087$ | $0.000000$ | $-1.218841$ | $-0.359757$ | Unstable |
| | $-0.157707$ | $1.490681$ | $-1.576304$ | $0.604867$ | Saddle |
| | $0.019835$ | $-7.439467$ | $-0.272716 + 0.102379i$ | $\omega_1^*$ | Unstable |
| 3 | $-0.140625$ | $0.000000$ | $-1.265625$ | $-0.431939$ | Unstable |
| | $-0.171897$ | $1.424848$ | $-1.575813$ | $0.747308$ | Saddle |
| | $0.020951$ | $-7.228280$ | $-0.267511 + 0.119271i$ | $\omega_1^*$ | Unstable |
| 4 | $-0.162338$ | $0.000000$ | $-1.352814$ | $-0.570438$ | Unstable |
| | $-0.193817$ | $1.400092$ | $-1.621538$ | $1.029052$ | Saddle |
| | $0.022175$ | $-7.007676$ | $-0.260192 + 0.135899i$ | $\omega_1^*$ | Unstable |
| 5 | $-0.198276$ | $0.000000$ | $-1.520115$ | $-0.872493$ | Unstable |
| | $-0.228379$ | $1.414932$ | $-1.738561$ | $1.626456$ | Saddle |
| | $0.023520$ | $-6.775662$ | $-0.250101 + 0.152372i$ | $\omega_1^*$ | Unstable |
| 6 | $-0.269231$ | $0.000000$ | $-1.884615$ | $-1.717759$ | Unstable |
| | $-0.286178$ | $1.466486$ | $-1.990512$ | $3.054616$ | Saddle |
| | $0.024998$ | $-6.529586$ | $-0.236345 + 0.168560i$ | $\omega_1^*$ | Unstable |
| 7 | $-0.475000$ | $0.000000$ | $-3.008333$ | $-5.970498$ | Unstable |
| | $-0.394693$ | $1.549080$ | $-2.551477$ | $7.195620$ | Saddle |
| | $0.026612$ | $-6.265829$ | $-0.217702 + 0.183998i$ | $\omega_1^*$ | Unstable |
| 8 | $-8.500000$ | $0.000000$ | $-48.166667$ | $-2234.669905$ | Unstable |
| | $-0.655088$ | $1.654624$ | $-4.053436$ | $24.826161$ | Saddle |
| | $0.028350$ | $-5.979315$ | $-0.192517 + 0.197658i$ | $\omega_1^*$ | Unstable |

Table SM.32: Two loop MOMc scheme $SU(3)$ fixed points in the linear covariant gauge for $0 \leq N_f \leq 8$.

| $N_f$ | $a_\infty$ | $\alpha_\infty$ | $\omega_1$ | $\omega_2$ | Infrared Stability |
|---|---|---|---|---|---|
| 9 | 0.416667 | 0.000000 | 2.083333 | $-6.559457$ | Saddle |
| | $-2.005279$ | 1.774537 | $-12.274877$ | 288.925968 | Saddle |
| | 0.030157 | $-5.662741$ | $-0.158644 + 0.207470i$ | $\omega_1^*$ | Unstable |
| 10 | 0.175676 | 0.000000 | 0.761261 | $-1.485115$ | Saddle |
| | 1.877605 | 1.901669 | 11.687629 | 308.993407 | **Stable** |
| | 0.031863 | $-5.305495$ | $-0.113704 + 0.209416i$ | $\omega_1^*$ | Unstable |
| 11 | 0.098214 | 0.000000 | 0.360119 | $-0.615875$ | Saddle |
| | 0.641787 | 2.031059 | 4.139533 | 43.163948 | **Stable** |
| | 0.033011 | $-4.893063$ | $-0.056708 + 0.196109i$ | $\omega_1^*$ | Unstable |
| 12 | 0.060000 | 0.000000 | 0.180000 | $-0.318789$ | Saddle |
| | 0.388425 | 2.159716 | 2.624657 | 18.556964 | **Stable** |
| | 0.032458 | $-4.413214$ | $0.005854 + 0.156886i$ | $\omega_1^*$ | **Stable** |
| 13 | 0.037234 | 0.000000 | 0.086879 | $-0.180136$ | Saddle |
| | 0.279220 | 2.286045 | 1.987272 | 11.076848 | **Stable** |
| | 0.028198 | $-3.894191$ | $0.049002 + 0.090548i$ | $\omega_1^*$ | **Stable** |
| 14 | 0.022124 | 0.000000 | 0.036873 | $-0.101809$ | Saddle |
| | 0.218329 | 2.409317 | 1.639661 | 7.719501 | **Stable** |
| | 0.019968 | $-3.455109$ | $0.049602 + 0.026473i$ | $\omega_1^*$ | **Stable** |
| 15 | 0.011364 | 0.000000 | 0.011364 | $-0.051152$ | Saddle |
| | 0.179438 | 2.529300 | 1.421443 | 5.877984 | **Stable** |
| | 0.010986 | $-3.179697$ | 0.012311 | 0.044184 | **Stable** |
| 16 | 0.003311 | 0.000000 | 0.001104 | $-0.014853$ | Saddle |
| | 0.152399 | 2.646029 | 1.271364 | 4.736020 | **Stable** |
| | 0.003287 | $-3.037061$ | 0.001109 | 0.014565 | **Stable** |

Table SM.33: Two loop MOMc scheme $SU(3)$ fixed points in the linear covariant gauge for $9 \leq N_f \leq 16$.

| $N_f$ | $a_\infty$ | $\alpha_\infty$ | $\omega_1$ | $\omega_2$ | Infrared Stability |
|---|---|---|---|---|---|
| 0 | - | - | - | - | - |
| 1 | - | - | - | - | - |
| 2 | - | - | - | - | - |
| 3 | - | - | - | - | - |
| 4 | - | - | - | - | - |
| 5 | - | - | - | - | - |
| 6 | 0.376838 | 0.000000 | 8.967913 | $-17.527803$ | Saddle |
| | $-0.157037$ | 0.000000 | $-1.557339$ | 0.440486 | Saddle |
| | $-0.128194$ | $-1.147531$ | $-1.211368$ | $-0.460430$ | Unstable |
| | $-1.292046$ | $-2.634300$ | 68.690766 | $-3544.055878$ | Saddle |
| 7 | 0.133309 | 0.000000 | 1.925529 | $-1.274016$ | Saddle |
| | $-0.104095$ | 0.000000 | $-1.174057$ | 0.095941 | Saddle |
| | $-0.214683$ | 1.288173 | $-1.573850$ | $-5.801025$ | Unstable |
| | 0.706010 | 1.360097 | 19.380284 | 287.310627 | **Stable** |
| | $-0.095740$ | $-0.603835$ | $-1.013968$ | $-0.107943$ | Unstable |
| | 0.214144 | $-3.237875$ | 2.973070 | 23.991904 | **Stable** |
| 8 | 0.087280 | 0.000000 | 0.994256 | $-0.539222$ | Saddle |
| | $-0.086393$ | 0.000000 | $-0.974148$ | 0.063587 | Saddle |
| | $-0.160471$ | 1.435245 | $-2.220112 + 0.285716i$ | $\omega_1^*$ | Unstable |
| | 0.243561 | 1.517246 | 4.361617 | 17.171076 | **Stable** |
| | $-0.081373$ | $-0.501370$ | $-0.878912$ | $-0.068305$ | Unstable |
| | 0.105376 | $-3.505933$ | 0.821200 | 3.331239 | **Stable** |
| 9 | 0.064858 | 0.000000 | 0.598100 | $-0.329837$ | Saddle |
| | $-0.076815$ | 0.000000 | $-0.838954$ | 0.060985 | Saddle |
| | $-0.144432$ | 1.533260 | $-1.971063 + 0.961219i$ | $\omega_1^*$ | Unstable |
| | 0.173916 | 1.629597 | 3.118963 | 7.679779 | **Stable** |
| | $-0.072489$ | $-0.532671$ | $-0.760841$ | $-0.064394$ | Unstable |
| | 0.069807 | $-3.572069$ | 0.407791 | 1.069856 | **Stable** |
| 10 | 0.050466 | 0.000000 | 0.374550 | $-0.233644$ | Saddle |
| | $-0.070806$ | 0.000000 | $-0.737321$ | 0.065568 | Saddle |
| | $-0.136632$ | 1.581071 | $-1.866288 + 1.211969i$ | $\omega_1^*$ | Unstable |
| | 0.144252 | 1.712801 | 2.884799 | 4.757372 | **Stable** |
| | $-0.066482$ | $-0.609634$ | $-0.663934$ | $-0.068658$ | Unstable |
| | 0.051534 | $-3.505080$ | 0.253430 | 0.491520 | **Stable** |

Table SM.34: Three loop MOMc scheme $SU(3)$ fixed points in the linear covariant gauge for $0 \leq N_f \leq 10$.

| $N_f$ | $a_\infty$ | $\alpha_\infty$ | $\omega_1$ | $\omega_2$ | Infrared Stability |
|---|---|---|---|---|---|
| 11 | 0.039778 | 0.000000 | 0.232633 | −0.176390 | Saddle |
| | −0.066855 | 0.000000 | −0.657133 | 0.072433 | Saddle |
| | −0.132152 | 1.587388 | $-1.787878 + 1.359054i$ | $\omega_1^*$ | Unstable |
| | 0.127850 | 1.773389 | $3.092467 + 0.606642i$ | $\omega_1^*$ | **Stable** |
| | −0.062247 | −0.702927 | −0.583979 | −0.075414 | Unstable |
| | 0.039651 | −3.389029 | 0.171598 | 0.271810 | **Stable** |
| 12 | 0.031047 | 0.000000 | 0.138086 | −0.135538 | Saddle |
| | −0.064339 | 0.000000 | −0.593006 | 0.080029 | Saddle |
| | −0.129350 | 1.558225 | $-1.704032 + 1.434209i$ | $\omega_1^*$ | Unstable |
| | 0.117718 | 1.815119 | $2.680238 + 0.964374i$ | $\omega_1^*$ | **Stable** |
| | −0.059248 | −0.800132 | −0.517357 | −0.082905 | Unstable |
| | 0.030606 | −3.279886 | 0.116888 | 0.163201 | **Stable** |
| 13 | 0.023405 | 0.000000 | 0.074895 | −0.102106 | Saddle |
| | −0.063019 | 0.000000 | −0.542963 | 0.087687 | Saddle |
| | −0.127449 | 1.496387 | $-1.602183 + 1.441337i$ | $\omega_1^*$ | Unstable |
| | 0.111195 | 1.840240 | $2.418995 + 1.132035i$ | $\omega_1^*$ | **Stable** |
| | −0.057229 | −0.893883 | −0.461970 | −0.090382 | Unstable |
| | 0.022969 | −3.195200 | 0.070154 | 0.105894 | **Stable** |
| 14 | 0.016367 | 0.000000 | 0.034376 | −0.071889 | Saddle |
| | −0.062897 | 0.000000 | −0.507681 | 0.094896 | Saddle |
| | −0.125949 | 1.401754 | $-1.476099 + 1.374496i$ | $\omega_1^*$ | Unstable |
| | 0.107062 | 1.849988 | $2.241342 + 1.251320i$ | $\omega_1^*$ | **Stable** |
| | −0.056110 | −0.977448 | −0.417270 | −0.097310 | Unstable |
| | 0.016059 | −3.131502 | 0.033458 | 0.070753 | **Stable** |
| 15 | 0.009655 | 0.000000 | 0.011107 | −0.042821 | Saddle |
| | −0.064209 | 0.000000 | −0.491223 | 0.100802 | Saddle |
| | −0.124402 | 1.270876 | $-1.322550 + 1.220865i$ | $\omega_1^*$ | Unstable |
| | 0.104715 | 1.844808 | $2.114579 + 1.357997i$ | $\omega_1^*$ | **Stable** |
| | −0.055981 | −1.041760 | −0.384692 | −0.102920 | Unstable |
| | 0.009509 | −3.078808 | 0.010998 | 0.041741 | **Stable** |
| 16 | 0.003156 | 0.000000 | 0.001101 | −0.014138 | Saddle |
| | −0.067516 | 0.000000 | −0.503884 | 0.103275 | Saddle |
| | −0.122233 | 1.095037 | $-1.140512 + 0.958182i$ | $\omega_1^*$ | Unstable |
| | 0.103864 | 1.824430 | $2.020475 + 1.468050i$ | $\omega_1^*$ | **Stable** |
| | −0.057170 | −1.071190 | −0.369266 | −0.105569 | Unstable |
| | 0.003136 | −3.027336 | 0.001100 | 0.013963 | **Stable** |

Table SM.35: Three loop MOMc scheme $SU(3)$ fixed points in the linear covariant gauge for $11 \leq N_f \leq 16$.

| $N_f$ | $a_\infty$ | $\alpha_\infty$ | $\omega_1$ | $\omega_2$ | Infrared Stability |
|---|---|---|---|---|---|
| 0 | $-0.107843$ | $0.000000$ | $-1.186275$ | $-0.521228$ | Unstable |
| | $-1.441499$ | $3.444620$ | $-34.161015$ | $49.404040$ | Saddle |
| | $0.017534$ | $-7.058964$ | $-0.127222 + 0.144133i$ | $\omega_1^*$ | Unstable |
| 1 | $-0.115672$ | $0.000000$ | $-1.195274$ | $-0.551089$ | Unstable |
| | $-0.447424$ | $2.927757$ | $-6.783942$ | $6.388273$ | Saddle |
| | $0.017894$ | $-6.976709$ | $-0.119130 + 0.145111i$ | $\omega_1^*$ | Unstable |
| 2 | $-0.126087$ | $0.000000$ | $-1.218841$ | $-0.603296$ | Unstable |
| | $-0.323404$ | $2.543347$ | $-3.957088$ | $3.643666$ | Saddle |
| | $0.018260$ | $-6.891446$ | $-0.110424 + 0.145613i$ | $\omega_1^*$ | Unstable |
| 3 | $-0.140625$ | $0.000000$ | $-1.265625$ | $-0.695787$ | Unstable |
| | $-0.290087$ | $2.253216$ | $-3.028611$ | $3.060670$ | Saddle |
| | $0.018627$ | $-6.802950$ | $-0.101034 + 0.145527i$ | $\omega_1^*$ | Unstable |
| 4 | $-0.162338$ | $0.000000$ | $-1.352814$ | $-0.869962$ | Unstable |
| | $-0.293348$ | $2.036102$ | $-2.670969$ | $3.235144$ | Saddle |
| | $0.018988$ | $-6.710993$ | $-0.090891 + 0.144710i$ | $\omega_1^*$ | Unstable |
| 5 | $-0.198276$ | $0.000000$ | $-1.520115$ | $-1.241606$ | Unstable |
| | $-0.328917$ | $1.881145$ | $-2.635561$ | $4.247897$ | Saddle |
| | $0.019331$ | $-6.615361$ | $-0.079924 + 0.142973i$ | $\omega_1^*$ | Unstable |
| 6 | $-0.269231$ | $0.000000$ | $-1.884615$ | $-2.255046$ | Unstable |
| | $-0.420048$ | $1.783280$ | $-2.974743$ | $7.429881$ | Saddle |
| | $0.019638$ | $-6.515884$ | $-0.068082 + 0.140070i$ | $\omega_1^*$ | Unstable |
| 7 | $-0.475000$ | $0.000000$ | $-3.008333$ | $-7.196934$ | Unstable |
| | $-0.684444$ | $1.739909$ | $-4.311632$ | $21.951341$ | Saddle |
| | $0.019883$ | $-6.412503$ | $-0.055346 + 0.135682i$ | $\omega_1^*$ | Unstable |
| 8 | $-8.500000$ | $0.000000$ | $-48.166667$ | $-2484.589810$ | Unstable |
| | $-3.166699$ | $1.748010$ | $-18.042653$ | $542.343125$ | Saddle |
| | $0.020025$ | $-6.305377$ | $-0.041771 + 0.129403i$ | $\omega_1^*$ | Unstable |

Table SM.36: Two loop MOMc scheme $SU(3)$ fixed points in the Curci-Ferrari gauge for $0 \leq N_f \leq 8$.

| $N_f$ | $a_\infty$ | $\alpha_\infty$ | $\omega_1$ | $\omega_2$ | Infrared Stability |
|---|---|---|---|---|---|
| 9 | 0.416667 | 0.000000 | 2.083333 | $-6.816830$ | Saddle |
| | 0.990163 | 1.801827 | 5.267544 | 62.694245 | **Stable** |
| | 0.020001 | $-6.195104$ | $-0.027551 + 0.120732i$ | $\omega_1^*$ | Unstable |
| 10 | 0.175676 | 0.000000 | 0.761261 | $-1.469864$ | Saddle |
| | 0.406325 | 1.892187 | 2.105797 | 12.566688 | **Stable** |
| | 0.019717 | $-6.083107$ | $-0.013124 + 0.109104i$ | $\omega_1^*$ | Unstable |
| 11 | 0.098214 | 0.000000 | 0.360119 | $-0.592042$ | Saddle |
| | 0.251163 | 2.007962 | 1.322551 | 5.675319 | **Stable** |
| | 0.019038 | $-5.972364$ | $0.000681 + 0.093990i$ | $\omega_1^*$ | **Stable** |
| 12 | 0.060000 | 0.000000 | 0.180000 | $-0.302779$ | Saddle |
| | 0.181025 | 2.138558 | 1.001399 | 3.435452 | **Stable** |
| | 0.017776 | $-5.868665$ | $0.012490 + 0.075147i$ | $\omega_1^*$ | **Stable** |
| 13 | 0.037234 | 0.000000 | 0.086879 | $-0.171230$ | Saddle |
| | 0.141722 | 2.275676 | 0.842433 | 2.413044 | **Stable** |
| | 0.015704 | $-5.782642$ | $0.020391 + 0.053066i$ | $\omega_1^*$ | **Stable** |
| 14 | 0.022124 | 0.000000 | 0.036873 | $-0.097697$ | Saddle |
| | 0.116851 | 2.413714 | 0.756748 | 1.848685 | **Stable** |
| | 0.012603 | $-5.732572$ | $0.022386 + 0.029446i$ | $\omega_1^*$ | **Stable** |
| 15 | 0.011364 | 0.000000 | 0.011364 | $-0.049812$ | Saddle |
| | 0.099800 | 2.549312 | 0.709927 | 1.495426 | **Stable** |
| | 0.008357 | $-5.747686$ | $0.017482 + 0.005512i$ | $\omega_1^*$ | **Stable** |
| 16 | 0.003311 | 0.000000 | 0.001104 | $-0.014717$ | Saddle |
| | 0.087420 | 2.680663 | 0.686914 | 1.252299 | **Stable** |
| | 0.003018 | $-5.873459$ | 0.001123 | 0.012349 | **Stable** |

Table SM.37: Two loop MOMc scheme $SU(3)$ fixed points in the Curci-Ferrari gauge for $9 \leq N_f \leq 16$.

| $N_f$ | $a_\infty$ | $\alpha_\infty$ | $\omega_1$ | $\omega_2$ | Infrared Stability |
|---|---|---|---|---|---|
| 0 | 0.001337 | $-118.546560$ | $-0.198727 + 0.734029i$ | $\omega_1^*$ | Unstable |
| 1 | 0.001520 | $-109.372092$ | $-0.221197 + 0.760714i$ | $\omega_1^*$ | Unstable |
| 2 | 0.001737 | $-100.607646$ | $-0.247051 + 0.789402i$ | $\omega_1^*$ | Unstable |
| 3 | 0.001995 | $-92.247610$ | $-0.276950 + 0.820206i$ | $\omega_1^*$ | Unstable |
| 4 | 0.002306 | $-84.285663$ | $-0.311722 + 0.853191i$ | $\omega_1^*$ | Unstable |
| 5 | $-0.288882$ | 0.000000 | $-1.202685$ | $-1.993810$ | Unstable |
| | $-0.632171$ | 0.000000 | 5.759451 | $-5.895610$ | Saddle |
| | $-0.938008$ | $-0.102806$ | $14.189865 + 11.136201i$ | $\omega_1^*$ | **Stable** |
| | 2.648285 | $-1.223872$ | 349.372742 | 4427.431158 | **Stable** |
| | 0.002682 | $-76.714735$ | $-0.352404 + 0.888330i$ | $\omega_1^*$ | Unstable |
| 6 | 0.196106 | 0.000000 | 3.745391 | $-1.532209$ | Saddle |
| | $-0.113462$ | 0.000000 | $-1.253750$ | $-0.335471$ | Unstable |
| | 0.235280 | 0.841151 | 4.602038 | 3.310527 | **Stable** |
| | 0.202798 | $-2.027821$ | 3.832618 | 7.978391 | **Stable** |
| | 0.003141 | $-69.527006$ | $-0.400312 + 0.925435i$ | $\omega_1^*$ | Unstable |
| 7 | 0.112000 | 0.000000 | 1.585924 | $-0.545641$ | Saddle |
| | $-0.090630$ | 0.000000 | $-1.038468$ | $-0.184902$ | Unstable |
| | 0.132830 | 1.204426 | 1.886041 | 1.262751 | **Stable** |
| | 0.122896 | $-2.432963$ | 1.549627 | 2.978706 | **Stable** |
| | 0.003708 | $-62.713967$ | $-0.457125 + 0.964030i$ | $\omega_1^*$ | Unstable |
| 8 | 0.080350 | 0.000000 | 0.914933 | $-0.330323$ | Saddle |
| | $-0.079597$ | 0.000000 | $-0.897878$ | $-0.112585$ | Unstable |
| | 0.100831 | 1.489840 | $1.059318 + 0.153296i$ | $\omega_1^*$ | **Stable** |
| | 0.091025 | $-2.756078$ | 0.876517 | 1.709318 | **Stable** |
| | 0.004415 | $-56.266599$ | $-0.524999 + 1.003131i$ | $\omega_1^*$ | Unstable |
| 9 | 0.062163 | 0.000000 | 0.575260 | $-0.240091$ | Saddle |
| | $-0.073064$ | 0.000000 | $-0.794695$ | $-0.066135$ | Unstable |
| | 0.085517 | 1.723245 | $0.857209 + 0.283037i$ | $\omega_1^*$ | **Stable** |
| | 0.072915 | $-3.047925$ | 0.565155 | 1.143989 | **Stable** |
| | 0.005308 | $-50.175784$ | $-0.606702 + 1.040873i$ | $\omega_1^*$ | Unstable |
| 10 | 0.049528 | 0.000000 | 0.368737 | $-0.188899$ | Saddle |
| | $-0.068974$ | 0.000000 | $-0.715128$ | $-0.031942$ | Unstable |
| | $-0.072996$ | 0.497447 | $-0.768108$ | 0.029545 | Saddle |
| | 0.077080 | 1.908693 | $0.763121 + 0.343214i$ | $\omega_1^*$ | **Stable** |
| | $-0.097074$ | 2.001161 | $-0.542863 + 0.293545i$ | $\omega_1^*$ | Unstable |
| | 0.060714 | $-3.328911$ | 0.383797 | 0.825087 | **Stable** |
| | 0.006448 | $-44.433112$ | $-0.705767 + 1.073833i$ | $\omega_1^*$ | Unstable |

Table SM.38: Three loop MOMc scheme $SU(3)$ fixed points in the Curci-Ferrari gauge for $0 \leq N_f \leq 10$.

| $N_f$ | $a_\infty$ | $\alpha_\infty$ | $\omega_1$ | $\omega_2$ | Infrared Stability |
|---|---|---|---|---|---|
| 11 | 0.039670 | 0.000000 | 0.232163 | −0.153163 | Saddle |
| | −0.066551 | 0.000000 | −0.653396 | −0.004738 | Unstable |
| | −0.066999 | 0.065284 | −0.659187 | 0.004724 | Saddle |
| | 0.072290 | 2.050258 | $0.719589 + 0.387455i$ | $\omega_1^*$ | **Stable** |
| | −0.106341 | 2.215953 | $-0.631793 + 0.855448i$ | $\omega_1^*$ | Unstable |
| | 0.051508 | −3.611843 | 0.261167 | 0.618788 | **Stable** |
| | 0.007926 | −39.032462 | $-0.826569 + 1.095831i$ | $\omega_1^*$ | Unstable |
| 12 | 0.031319 | 0.000000 | 0.138871 | −0.123892 | Saddle |
| | −0.065521 | 0.000000 | −0.607770 | 0.017922 | Saddle |
| | 0.069815 | 2.152213 | $0.705387 + 0.427713i$ | $\omega_1^*$ | **Stable** |
| | −0.115430 | 2.195272 | $-0.750210 + 1.248399i$ | $\omega_1^*$ | Unstable |
| | −0.064041 | −0.232240 | −0.589306 | −0.017922 | Unstable |
| | 0.043848 | −3.909767 | 0.169678 | 0.470051 | **Stable** |
| | 0.009865 | −33.972941 | $-0.974128 + 1.095776i$ | $\omega_1^*$ | Unstable |
| 13 | 0.023793 | 0.000000 | 0.075559 | −0.096909 | Saddle |
| | −0.065913 | 0.000000 | −0.579856 | 0.037141 | Saddle |
| | −0.125218 | 2.062963 | $-0.909757 + 1.565783i$ | $\omega_1^*$ | Unstable |
| | 0.069084 | 2.217748 | $0.712232 + 0.469340i$ | $\omega_1^*$ | **Stable** |
| | −0.062983 | −0.456057 | −0.544055 | −0.036657 | Unstable |
| | 0.036699 | −4.244411 | 0.097307 | 0.348928 | **Stable** |
| | 0.012431 | −29.264150 | $-1.153020 + 1.053766i$ | $\omega_1^*$ | Unstable |
| 14 | 0.016697 | 0.000000 | 0.034654 | −0.070077 | Saddle |
| | −0.068069 | 0.000000 | −0.575943 | 0.052949 | Saddle |
| | −0.135920 | 1.864293 | $-1.111548 + 1.785903i$ | $\omega_1^*$ | Unstable |
| | 0.069941 | 2.248236 | $0.738201 + 0.516429i$ | $\omega_1^*$ | **Stable** |
| | −0.063733 | −0.608559 | −0.522564 | −0.051182 | Unstable |
| | 0.028567 | −4.674679 | 0.039217 | 0.229427 | **Stable** |
| | 0.015825 | −24.934548 | $-1.364073 + 0.933471i$ | $\omega_1^*$ | Unstable |
| 15 | 0.009829 | 0.000000 | 0.011156 | −0.042456 | Saddle |
| | −0.072785 | 0.000000 | −0.611759 | 0.063534 | Saddle |
| | −0.147346 | 1.616767 | $-1.339504 + 1.830953i$ | $\omega_1^*$ | Unstable |
| | 0.072570 | 2.242597 | $0.786414 + 0.573995i$ | $\omega_1^*$ | **Stable** |
| | −0.066872 | −0.664955 | −0.535377 | −0.059912 | Unstable |
| | 0.014116 | −5.411305 | 0.006890 | 0.071247 | **Stable** |
| | 0.020229 | −21.040822 | $-1.596994 + 0.657042i$ | $\omega_1^*$ | Unstable |
| 16 | 0.003182 | 0.000000 | 0.001102 | −0.014126 | Saddle |
| | −0.081709 | 0.000000 | −0.726557 | 0.061928 | Saddle |
| | −0.157953 | 1.317632 | $-1.527959 + 1.507072i$ | $\omega_1^*$ | Unstable |
| | 0.077644 | 2.196108 | $0.867418 + 0.650571i$ | $\omega_1^*$ | **Stable** |
| | −0.074305 | −0.567105 | −0.620114 | −0.057643 | Unstable |
| | 0.003391 | −5.848457 | 0.001077 | 0.014253 | **Stable** |
| | 0.025653 | −17.666399 | −2.254257 | −1.386753 | Unstable |

Table SM.39: Three loop MOMc scheme $SU(3)$ fixed points in the Curci-Ferrari gauge for $11 \leq N_f \leq 16$.

| $N_f$ | $a_\infty$ | $\alpha_\infty$ | $\omega_1$ | $\omega_2$ | Infrared Stability |
|---|---|---|---|---|---|
| 0 | $-0.105214$ | 1.901148 | $-1.161021$ | $-0.025403$ | Unstable |
| | $-0.104631$ | 2.025591 | $-1.156237$ | 0.026068 | Saddle |
| | 0.027305 | $-10.093993$ | $-0.392487 + 0.307798i$ | $\omega_1^*$ | Unstable |
| 1 | 0.027946 | $-9.938321$ | $-0.375762 + 0.310841i$ | $\omega_1^*$ | Unstable |
| 2 | 0.028622 | $-9.772994$ | $-0.357291 + 0.313350i$ | $\omega_1^*$ | Unstable |
| 3 | 0.029335 | $-9.596497$ | $-0.336761 + 0.315146i$ | $\omega_1^*$ | Unstable |
| 4 | 0.030084 | $-9.406919$ | $-0.313785 + 0.315978i$ | $\omega_1^*$ | Unstable |
| 5 | 0.030863 | $-9.201816$ | $-0.287879 + 0.315482i$ | $\omega_1^*$ | Unstable |
| 6 | 0.031664 | $-8.977998$ | $-0.258445 + 0.313121i$ | $\omega_1^*$ | Unstable |
| 7 | 0.032463 | $-8.731222$ | $-0.224750 + 0.308085i$ | $\omega_1^*$ | Unstable |
| 8 | 0.033217 | $-8.455727$ | $-0.185935 + 0.299125i$ | $\omega_1^*$ | Unstable |
| 9 | 0.033833 | $-8.143603$ | $-0.141127 + 0.284271i$ | $\omega_1^*$ | Unstable |
| 10 | 0.323141 | 0.519306 | 1.041758 | $-4.497781$ | Saddle |
| | $-19.551114$ | 1.319818 | 703.041137 | $-2026.744573$ | Saddle |
| | 0.034117 | $-7.784169$ | $-0.089868 + 0.260414i$ | $\omega_1^*$ | Unstable |
| 11 | 0.123479 | 0.165298 | 0.406388 | $-1.137423$ | Saddle |
| | 5.519238 | 1.674527 | 188.897763 | 396.630816 | **Stable** |
| | 0.033655 | $-7.364723$ | $-0.033540 + 0.222947i$ | $\omega_1^*$ | Unstable |
| 12 | 1.476988 | 1.916484 | $42.559782 + 20.144833i$ | $\omega_1^*$ | **Stable** |
| | 0.067453 | $-0.046271$ | 0.190327 | $-0.515078$ | Saddle |
| | 0.031606 | $-6.879356$ | $0.020789 + 0.167020i$ | $\omega_1^*$ | **Stable** |
| 13 | 0.806259 | 2.117233 | $18.914033 + 11.732178i$ | $\omega_1^*$ | **Stable** |
| | 0.039716 | $-0.191430$ | 0.089168 | $-0.273455$ | Saddle |
| | 0.026761 | $-6.364145$ | $0.055556 + 0.095535i$ | $\omega_1^*$ | **Stable** |
| 14 | 0.546940 | 2.294665 | $11.561464 + 8.159073i$ | $\omega_1^*$ | **Stable** |
| | 0.022912 | $-0.293143$ | 0.037277 | $-0.149419$ | Saddle |
| | 0.019089 | $-5.932927$ | $0.055911 + 0.026515i$ | $\omega_1^*$ | **Stable** |
| 15 | 0.412326 | 2.456372 | $8.208946 + 6.298732i$ | $\omega_1^*$ | **Stable** |
| | 0.011554 | $-0.364086$ | 0.011402 | $-0.073734$ | Saddle |
| | 0.010713 | $-5.675674$ | 0.012346 | 0.056948 | **Stable** |
| 16 | 0.330726 | 2.606374 | $6.351019 + 5.181185i$ | $\omega_1^*$ | **Stable** |
| | 0.003326 | $-0.412862$ | 0.001104 | $-0.021234$ | Saddle |
| | 0.003263 | $-5.575657$ | 0.001109 | 0.020108 | **Stable** |

Table SM.40: Two loop MOMc scheme $SU(3)$ fixed points in the MAG for $0 \leq N_f \leq 16$.

| $N_f$ | $a_\infty$ | $\alpha_\infty$ | $\omega_1$ | $\omega_2$ | Infrared Stability |
|---|---|---|---|---|---|
| 0 | 0.001208 | $-66.671650$ | $-0.140849 + 0.061103i$ | $\omega_1^*$ | Unstable |
| 1 | 0.001220 | $-66.327739$ | $-0.141268 + 0.060997i$ | $\omega_1^*$ | Unstable |
| 2 | 0.001232 | $-65.981196$ | $-0.141690 + 0.060884i$ | $\omega_1^*$ | Unstable |
| 3 | 0.001244 | $-65.631941$ | $-0.142114 + 0.060765i$ | $\omega_1^*$ | Unstable |
| 4 | 0.001256 | $-65.279890$ | $-0.142539 + 0.060640i$ | $\omega_1^*$ | Unstable |
| 5 | 0.001269 | $-64.924953$ | $-0.142967 + 0.060507i$ | $\omega_1^*$ | Unstable |
| 6 | 0.192735 | $-1.788243$ | 3.910974 | $-6.167993$ | Saddle |
| | $-0.376120$ | $-3.470680$ | 15.983527 | $-62.823912$ | Saddle |
| | 0.001282 | $-64.567040$ | $-0.143398 + 0.060366i$ | $\omega_1^*$ | Unstable |
| 7 | 0.107110 | $-1.341657$ | 1.566497 | $-1.213447$ | Saddle |
| | $-0.497653$ | $-4.057287$ | 25.109843 | $-305.605268$ | Saddle |
| | 0.001295 | $-64.206051$ | $-0.143830 + 0.060217i$ | $\omega_1^*$ | Unstable |
| 8 | 0.077117 | $-1.000791$ | 0.900626 | $-0.575398$ | Saddle |
| | $-1.198456$ | $-4.477518$ | 141.812647 | $-6153.234366$ | Saddle |
| | 0.001309 | $-63.841886$ | $-0.144264 + 0.060059i$ | $\omega_1^*$ | Unstable |
| 9 | 0.060025 | $-0.761340$ | 0.568218 | $-0.381005$ | Saddle |
| | 2.014127 | $-4.819139$ | 387.341962 | 37185.984046 | **Stable** |
| | 0.001323 | $-63.474435$ | $-0.144700 + 0.059892i$ | $\omega_1^*$ | Unstable |
| 10 | 0.048050 | $-0.606026$ | 0.365311 | $-0.288998$ | Saddle |
| | 0.525666 | $-5.116521$ | 25.061445 | 792.707980 | **Stable** |
| | 0.001338 | $-63.103585$ | $-0.145138 + 0.059715i$ | $\omega_1^*$ | Unstable |
| 11 | 0.038617 | $-0.508019$ | 0.230425 | $-0.229882$ | Saddle |
| | 0.296834 | $-5.387866$ | 7.437932 | 165.517733 | **Stable** |
| | 0.001352 | $-62.729216$ | $-0.145579 + 0.059527i$ | $\omega_1^*$ | Unstable |
| 12 | 0.030574 | $-0.447329$ | 0.138002 | $-0.183365$ | Saddle |
| | 0.203684 | $-5.644839$ | 3.182526 | 60.810915 | **Stable** |
| | 0.001368 | $-62.351201$ | $-0.146021 + 0.059328i$ | $\omega_1^*$ | Unstable |
| 13 | 0.023297 | $-0.412168$ | 0.075176 | $-0.141737$ | Saddle |
| | 0.152357 | $-5.896500$ | 1.565192 | 28.638488 | **Stable** |
| | 0.001383 | $-61.969404$ | $-0.146465 + 0.059117i$ | $\omega_1^*$ | Unstable |
| 14 | 0.016412 | $-0.396570$ | 0.034530 | $-0.101482$ | Saddle |
| | 0.018678 | $-5.773235$ | 0.017981 | 0.147102 | **Stable** |
| | 0.118778 | $-6.152061$ | 0.789257 | 15.231931 | **Stable** |
| | 0.033568 | $-6.408346$ | $-0.036840$ | 0.581060 | Saddle |
| | 0.001399 | $-61.583684$ | $-0.146910 + 0.058892i$ | $\omega_1^*$ | Unstable |
| 15 | 0.009714 | $-0.398207$ | 0.011136 | $-0.061017$ | Saddle |
| | 0.009926 | $-5.607244$ | 0.009922 | 0.061538 | **Stable** |
| | 0.093250 | $-6.426348$ | 0.350284 | 8.353139 | **Stable** |
| | 0.042793 | $-6.748763$ | $-0.068640$ | 1.158181 | Saddle |
| | 0.001416 | $-61.193890$ | $-0.147358 + 0.058653i$ | $\omega_1^*$ | Unstable |
| 16 | 0.003168 | $-0.416277$ | 0.001102 | $-0.020198$ | Saddle |
| | 0.003158 | $-5.568650$ | 0.001093 | 0.019646 | **Stable** |
| | 0.001433 | $-60.799859$ | $-0.147806 + 0.058400i$ | $\omega_1^*$ | Unstable |

Table SM.41: Three loop MOMc scheme $SU(3)$ fixed points in the MAG for $0 \leq N_f \leq 16$.

| $N_f$ | $a_\infty$ | $\alpha_\infty$ | $\omega_1$ | $\omega_2$ | Infrared Stability |
|---|---|---|---|---|---|
| 0 | $-0.107843$ | 0.000000 | $-1.186275$ | $-0.897640$ | Unstable |
| | $-0.097283$ | 1.883106 | $-1.120821$ | 0.645060 | Saddle |
| 1 | $-0.115672$ | 0.000000 | $-1.195274$ | $-0.759761$ | Unstable |
| | $-0.101756$ | 1.543401 | $-1.074127$ | 0.540432 | Saddle |
| 2 | $-0.126087$ | 0.000000 | $-1.218841$ | $-0.633513$ | Unstable |
| | $-0.110250$ | 1.232369 | $-1.069048$ | 0.457574 | Saddle |
| 3 | $-0.140625$ | 0.000000 | $-1.265625$ | $-0.523342$ | Unstable |
| | $-0.123795$ | 0.959309 | $-1.104866$ | 0.389357 | Saddle |
| 4 | $-0.162338$ | 0.000000 | $-1.352814$ | $-0.441275$ | Unstable |
| | $-0.144680$ | 0.745071 | $-1.189732$ | 0.338084 | Saddle |
| 5 | $-0.198276$ | 0.000000 | $-1.520115$ | $-0.426281$ | Unstable |
| | $-0.177837$ | 0.644155 | $-1.347233$ | 0.325942 | Saddle |
| 6 | $-0.269231$ | 0.000000 | $-1.884615$ | $-0.650422$ | Unstable |
| | $-0.240348$ | 0.890198 | $-1.690745$ | 0.428159 | Saddle |
| 7 | $-0.475000$ | 0.000000 | $-3.008333$ | $-2.580400$ | Unstable |
| | $-0.371380$ | 2.687463 | $-3.097478$ | 7.331940 | Saddle |
| 8 | $-8.500000$ | 0.000000 | $-48.166667$ | $-1349.493689$ | Unstable |
| | $-0.213043$ | 3.143453 | $-2.143310$ | 6.223509 | Saddle |
| 9 | 0.416667 | 0.000000 | 2.083333 | $-5.447734$ | Saddle |
| | $-0.138618$ | 3.346223 | $-1.492823$ | 4.157475 | Saddle |
| 10 | 0.175676 | 0.000000 | 0.761261 | $-1.562849$ | Saddle |
| | $-0.100116$ | 3.457186 | $-1.110629$ | 2.927645 | Saddle |
| 11 | 0.098214 | 0.000000 | 0.360119 | $-0.755891$ | Saddle |
| | $-0.077265$ | 3.517117 | $-0.864991$ | 2.173244 | Saddle |
| 12 | 0.060000 | 0.000000 | 0.180000 | $-0.425300$ | Saddle |
| | $-0.062334$ | 3.542702 | $-0.694318$ | 1.677074 | Saddle |
| 13 | 0.037234 | 0.000000 | 0.086879 | $-0.246309$ | Saddle |
| | $-0.051894$ | 3.542144 | $-0.568418$ | 1.330356 | Saddle |
| 14 | 0.022124 | 0.000000 | 0.036873 | $-0.135558$ | Saddle |
| | $-0.044218$ | 3.519700 | $-0.471081$ | 1.075822 | Saddle |
| 15 | 0.011364 | 0.000000 | 0.011364 | $-0.063193$ | Saddle |
| | $-0.038354$ | 3.477348 | $-0.392874$ | 0.881191 | Saddle |
| 16 | 0.003311 | 0.000000 | 0.001104 | $-0.016175$ | Saddle |
| | $-0.033734$ | 3.415417 | $-0.327904$ | 0.727070 | Saddle |
| | 0.003551 | $-3.032914$ | 0.001072 | 0.017476 | **Stable** |
| | 0.026797 | $-4.022330$ | $-0.049654$ | 0.361768 | Saddle |

Table SM.42: Two loop MOMg scheme $SU(3)$ fixed points in the linear covariant gauge for $0 \leq N_f \leq 16$.

| $N_f$ | $a_\infty$ | $\alpha_\infty$ | $\omega_1$ | $\omega_2$ | Infrared Stability |
|---|---|---|---|---|---|
| 0 | $-0.024396$ | 7.957411 | $-1.984033$ | 6.744064 | Saddle |
| | 0.006758 | 9.948958 | 0.401950 | $-0.494275$ | Saddle |
| | 0.126369 | $-4.051250$ | 17.556517 | $-28.687832$ | Saddle |
| | $-0.107262$ | $-4.682191$ | $-15.245266$ | 42.150738 | Saddle |
| 1 | $-0.022374$ | 7.930429 | $-1.779946$ | 5.672183 | Saddle |
| | 0.006543 | 9.989647 | 0.409703 | $-0.494429$ | Saddle |
| | 0.122032 | $-3.851166$ | 13.583126 | $-20.067494$ | Saddle |
| | $-0.098428$ | $-4.592614$ | $-11.788660$ | 29.555684 | Saddle |
| 2 | $-0.020636$ | 7.908881 | $-1.611342$ | 4.853939 | Saddle |
| | 0.006339 | 10.033440 | 0.417037 | $-0.494769$ | Saddle |
| | 0.119887 | $-3.633800$ | 10.429458 | $-13.985894$ | Saddle |
| | $-0.092364$ | $-4.499097$ | $-9.409931$ | 21.689275 | Saddle |
| 3 | $-0.019145$ | 7.891752 | $-1.472297$ | 4.222783 | Saddle |
| | 0.006146 | 10.079362 | 0.424049 | $-0.495358$ | Saddle |
| | 0.118759 | $-3.389407$ | 7.730391 | $-9.221858$ | Saddle |
| | $-0.087980$ | $-4.404002$ | 16.362714 | $-7.688888$ | Saddle |
| 4 | $-0.017861$ | 7.878276 | $-1.357237$ | 3.729405 | Saddle |
| | 0.005965 | 10.126716 | 0.430815 | $-0.496222$ | Saddle |
| | 0.117551 | $-3.096798$ | 5.290436 | $-5.227323$ | Saddle |
| | $-0.084622$ | $-4.310513$ | 12.553849 | $-6.407687$ | Saddle |
| 5 | $-0.016750$ | 7.867869 | $-1.261473$ | 3.338280 | Saddle |
| | 0.005796 | 10.174999 | 0.437392 | $-0.497368$ | Saddle |
| | $-0.366812$ | $-0.843273$ | $-3.997027 + 5.465032i$ | $\omega_1^*$ | Unstable |
| | 0.296510 | $-1.548366$ | $4.862709 + 3.449374i$ | $\omega_1^*$ | **Stable** |
| | 0.116540 | $-2.669227$ | 2.992075 | $-1.760510$ | Saddle |
| | $-0.081830$ | $-4.223009$ | 9.730971 | $-5.442825$ | Saddle |
| 6 | 0.217931 | 0.000000 | 4.285885 | $-2.361769$ | Saddle |
| | $-0.120440$ | 0.000000 | $-1.309010$ | 0.196551 | Saddle |
| | $-0.015783$ | 7.860089 | $-1.181242$ | 3.023972 | Saddle |
| | 0.005638 | 10.223850 | 0.443825 | $-0.498789$ | Saddle |
| | $-0.112163$ | $-0.522144$ | $-1.254620$ | $-0.215625$ | Unstable |
| | $-0.079236$ | $-4.147092$ | 7.594527 | $-4.716831$ | Saddle |
| 7 | 0.097651 | 0.000000 | 1.364058 | $-0.440222$ | Saddle |
| | $-0.080999$ | 0.000000 | $-0.938512$ | 0.113962 | Saddle |
| | $-0.280359$ | 1.615772 | $-2.000949$ | $-37.003249$ | Unstable |
| | 13.135493 | 1.642706 | 4504.439925 | 3996346.934174 | **Stable** |
| | $-0.014936$ | 7.854597 | $-1.113580$ | 2.768183 | Saddle |
| | 0.005489 | 10.273003 | 0.450148 | $-0.500470$ | Saddle |
| | $-0.080574$ | $-0.657584$ | $-0.960224$ | $-0.134359$ | Unstable |
| | $-0.076529$ | $-4.088971$ | 5.960320 | $-4.171817$ | Saddle |

Table SM.43: Three loop MOMg scheme $SU(3)$ fixed points in the linear covariant gauge for $0 \leq N_f \leq 7$.

| $N_f$ | $a_\infty$ | $\alpha_\infty$ | $\omega_1$ | $\omega_2$ | Infrared Stability |
|---|---|---|---|---|---|
| 8 | 0.064861 | 0.000000 | 0.737894 | −0.276082 | Saddle |
| | −0.064370 | 0.000000 | −0.726760 | 0.115659 | Saddle |
| | −0.014189 | 7.851137 | −1.056166 | 2.557621 | Saddle |
| | 0.005350 | 10.322266 | 0.456388 | −0.502395 | Saddle |
| | −0.065649 | −0.901302 | −0.758414 | −0.140875 | Unstable |
| | −0.073448 | −4.054170 | 4.700143 | −3.753735 | Saddle |
| 9 | 0.047997 | 0.000000 | 0.452324 | −0.224312 | Saddle |
| | −0.054246 | 0.000000 | −0.577766 | 0.127131 | Saddle |
| | −0.013527 | 7.849511 | −1.007180 | 2.382510 | Saddle |
| | 0.005219 | 10.371498 | 0.462563 | −0.504546 | Saddle |
| | −0.056014 | −1.178688 | −0.591311 | −0.163152 | Unstable |
| | −0.069783 | −4.046195 | 3.714472 | −3.406287 | Saddle |
| 10 | 0.037161 | 0.000000 | 0.287998 | −0.193650 | Saddle |
| | −0.047130 | 0.000000 | −0.463256 | 0.139912 | Saddle |
| | −0.012936 | 7.849566 | −0.965192 | 2.235566 | Saddle |
| | 0.005097 | 10.420594 | 0.468688 | −0.506903 | Saddle |
| | −0.048655 | −1.463580 | −0.429732 | −0.199015 | Unstable |
| | −0.065394 | −4.066062 | 2.926588 | −3.075584 | Saddle |
| 11 | 0.029277 | 0.000000 | 0.182697 | −0.166770 | Saddle |
| | −0.041710 | 0.000000 | −0.370824 | 0.151696 | Saddle |
| | −0.012407 | 7.851181 | −0.929065 | 2.111287 | Saddle |
| | 0.004981 | 10.469477 | 0.474774 | −0.509449 | Saddle |
| | −0.042471 | −1.743854 | $-0.257106 + 0.074951i$ | $\omega_1^*$ | Unstable |
| | −0.060255 | −4.112935 | 2.285146 | −2.723389 | Saddle |
| 12 | 0.023018 | 0.000000 | 0.111618 | −0.138971 | Saddle |
| | −0.037345 | 0.000000 | −0.293806 | 0.161408 | Saddle |
| | −0.011929 | 7.854262 | −0.897892 | 2.005466 | Saddle |
| | 0.004872 | 10.518092 | 0.480829 | −0.512167 | Saddle |
| | −0.037002 | −2.012868 | $-0.205209 + 0.117099i$ | $\omega_1^*$ | Unstable |
| | −0.054513 | −4.185258 | 1.762470 | −2.340295 | Saddle |

Table SM.44: Three loop MOMg scheme $SU(3)$ fixed points in the linear covariant gauge for $8 \leq N_f \leq 12$.

| $N_f$ | $a_\infty$ | $\alpha_\infty$ | $\omega_1$ | $\omega_2$ | Infrared Stability |
|---|---|---|---|---|---|
| 13 | 0.017680 | 0.000000 | 0.062919 | $-0.109064$ | Saddle |
| | $-0.033667$ | 0.000000 | $-0.228145$ | 0.168198 | Saddle |
| | $-0.011496$ | 7.858732 | $-0.870941$ | 1.914841 | Saddle |
| | 0.004769 | 10.566397 | 0.486860 | $-0.515042$ | Saddle |
| | $-0.032026$ | $-2.265993$ | $-0.159223 + 0.119920i$ | $\omega_1^*$ | Unstable |
| | 0.020792 | $-3.054531$ | 0.018260 | 0.207582 | **Stable** |
| | 0.024398 | $-3.342847$ | $-0.026999$ | 0.347710 | Saddle |
| | $-0.048471$ | $-4.281782$ | 1.345180 | $-1.946187$ | Saddle |
| 14 | 0.012809 | 0.000000 | 0.030337 | $-0.077336$ | Saddle |
| | $-0.030424$ | 0.000000 | $-0.171141$ | 0.171028 | Saddle |
| | $-0.011102$ | 7.864529 | 1.836856 | $-0.847619$ | Saddle |
| | 0.004672 | 10.614363 | 0.492870 | $-0.518057$ | Saddle |
| | $-0.027400$ | $-2.498603$ | $-0.119377 + 0.105275i$ | $\omega_1^*$ | Unstable |
| | 0.014243 | $-3.058910$ | 0.018658 | 0.106542 | **Stable** |
| | 0.021647 | $-3.678436$ | $-0.051391$ | 0.348938 | Saddle |
| | $-0.042493$ | $-4.402203$ | 1.023153 | $-1.574456$ | Saddle |
| 15 | 0.008032 | 0.000000 | 0.010387 | $-0.045066$ | Saddle |
| | $-0.027396$ | 0.000000 | $-0.120839$ | 0.168226 | Saddle |
| | $-0.010742$ | 7.871597 | 1.769483 | $-0.827437$ | Saddle |
| | 0.004579 | 10.661968 | 0.498863 | $-0.521201$ | Saddle |
| | $-0.022984$ | $-2.704610$ | $-0.085381 + 0.081005i$ | $\omega_1^*$ | Unstable |
| | 0.008466 | $-3.056382$ | 0.009002 | 0.049510 | **Stable** |
| | 0.019127 | $-4.000230$ | $-0.067169$ | 0.340074 | Saddle |
| | $-0.036884$ | $-4.547312$ | 0.783474 | $-1.252408$ | Saddle |
| 16 | 0.002914 | 0.000000 | 0.001088 | $-0.014301$ | Saddle |
| | $-0.024300$ | 0.000000 | $-0.075641$ | 0.156520 | Saddle |
| | $-0.010411$ | 7.879891 | 1.711096 | $-0.809993$ | Saddle |
| | 0.004492 | 10.709199 | 0.504841 | $-0.524461$ | Saddle |
| | $-0.018537$ | $-2.874291$ | $-0.056410 + 0.050604i$ | $\omega_1^*$ | Unstable |
| | 0.002939 | $-3.025985$ | 0.001074 | 0.014300 | **Stable** |
| | 0.016938 | $-4.324124$ | $-0.078445$ | 0.329721 | Saddle |
| | $-0.031826$ | $-4.718612$ | 0.610223 | $-0.991636$ | Saddle |

Table SM.45: Three loop MOMg scheme $SU(3)$ fixed points in the linear covariant gauge for $13 \leq N_f \leq 16$.

| $N_f$ | $a_\infty$ | $\alpha_\infty$ | $\omega_1$ | $\omega_2$ | Infrared Stability |
|---|---|---|---|---|---|
| 0 | $-0.107843$ | 0.000000 | $-1.186275$ | $-0.897640$ | Unstable |
| | $-0.101783$ | 2.304654 | $-1.302085$ | 0.730811 | Saddle |
| 1 | $-0.115672$ | 0.000000 | $-1.195274$ | $-0.759761$ | Unstable |
| | $-0.100264$ | 1.851063 | $-1.099926$ | 0.567363 | Saddle |
| 2 | $-0.126087$ | 0.000000 | $-1.218841$ | $-0.633513$ | Unstable |
| | $-0.106363$ | 1.430227 | $-1.034701$ | 0.467528 | Saddle |
| 3 | $-0.140625$ | 0.000000 | $-1.265625$ | $-0.523342$ | Unstable |
| | $-0.119534$ | 1.059068 | $-1.054351$ | 0.398318 | Saddle |
| 4 | $-0.162338$ | 0.000000 | $-1.352814$ | $-0.441275$ | Unstable |
| | $-0.141229$ | 0.761526 | $-1.144393$ | 0.351915 | Saddle |
| 5 | $-0.198276$ | 0.000000 | $-1.520115$ | $-0.426281$ | Unstable |
| | $-0.175690$ | 0.576664 | $-1.312078$ | 0.351364 | Saddle |
| 6 | $-0.269231$ | 0.000000 | $-1.884615$ | $-0.650422$ | Unstable |
| | $-0.235039$ | 0.581469 | $-1.610259$ | 0.522640 | Saddle |
| 7 | $-0.475000$ | 0.000000 | $-3.008333$ | $-2.580400$ | Unstable |
| | $-0.383899$ | 0.953720 | $-2.426115$ | 1.816884 | Saddle |
| 8 | $-8.500000$ | 0.000000 | $-48.166667$ | $-1349.493689$ | Unstable |
| | 23.639997 | 2.019362 | 133.526908 | 15909.261234 | **Stable** |
| 9 | 0.416667 | 0.000000 | 2.083333 | $-5.447734$ | Saddle |
| | 1.483448 | 2.977585 | 9.783430 | 194.645055 | **Stable** |
| 10 | 0.175676 | 0.000000 | 0.761261 | $-1.562849$ | Saddle |
| | $-0.677078$ | 3.391814 | $-5.076121$ | 74.995039 | Saddle |
| 11 | 0.098214 | 0.000000 | 0.360119 | $-0.755891$ | Saddle |
| | $-0.214653$ | 3.591762 | $-1.704749$ | 11.045625 | Saddle |
| 12 | 0.060000 | 0.000000 | 0.180000 | $-0.425300$ | Saddle |
| | $-0.120190$ | 3.688999 | $-0.977785$ | 4.521607 | Saddle |
| 13 | 0.037234 | 0.000000 | 0.086879 | $-0.246309$ | Saddle |
| | $-0.081565$ | 3.725102 | $-0.665812$ | 2.539106 | Saddle |
| 14 | 0.022124 | 0.000000 | 0.036873 | $-0.135558$ | Saddle |
| | $-0.061017$ | 3.718931 | $-0.491833$ | 1.654252 | Saddle |
| 15 | 0.011364 | 0.000000 | 0.011364 | $-0.063193$ | Saddle |
| | $-0.048395$ | 3.679756 | $-0.379555$ | 1.170275 | Saddle |
| 16 | 0.003311 | 0.000000 | 0.001104 | $-0.016175$ | Saddle |
| | $-0.039895$ | 3.611776 | $-0.299723$ | 0.869324 | Saddle |

Table SM.46: Two loop MOMg scheme $SU(3)$ fixed points in the Curci-Ferrari gauge for $0 \leq N_f \leq 16$.

| $N_f$ | $a_\infty$ | $\alpha_\infty$ | $\omega_1$ | $\omega_2$ | Infrared Stability |
|---|---|---|---|---|---|
| 0 | 0.460064 | 8.495363 | −213.649932 | −12440.927892 | Unstable |
| | 0.007738 | 10.025539 | 0.131205 | −0.219606 | Saddle |
| 1 | −0.097472 | 8.180213 | −10.730693 | 123.618992 | Saddle |
| | 0.007344 | 9.950089 | 0.146455 | −0.214983 | Saddle |
| | 0.308874 | −3.870589 | 49.412006 | −182.357778 | Saddle |
| | −0.179160 | −4.251889 | −16.457458 | 67.399009 | Saddle |
| 2 | −0.049941 | 7.983604 | −3.205340 | 18.833422 | Saddle |
| | 0.007003 | 9.911439 | 0.159443 | −0.214841 | Saddle |
| | 0.215810 | −3.589877 | 21.877513 | −47.960896 | Saddle |
| | −0.131387 | −4.192657 | −9.453637 | 26.751613 | Saddle |
| 3 | −0.035576 | 7.854474 | −1.844967 | 7.903415 | Saddle |
| | 0.006712 | 9.895659 | 0.171161 | −0.217315 | Saddle |
| | 0.179663 | −3.271526 | 11.665619 | −18.741627 | Saddle |
| | −0.108932 | −4.124354 | −6.297661 | 14.316811 | Saddle |
| 4 | −0.028497 | 7.763765 | −1.329949 | 4.720163 | Saddle |
| | 0.006460 | 9.895258 | 0.182136 | −0.221374 | Saddle |
| | 0.162874 | −2.832844 | 6.223685 | −6.955979 | Saddle |
| | −0.094624 | −4.060566 | −4.500192 | 8.545245 | Saddle |
| 5 | −0.024218 | 7.696411 | −1.068127 | 3.342502 | Saddle |
| | 0.006238 | 9.905757 | 0.192642 | −0.226434 | Saddle |
| | −0.260717 | −0.847655 | $-1.907700 + 2.999225i$ | $\omega_1^*$ | Unstable |
| | −0.083877 | −4.011682 | 5.366901 | −3.361659 | Saddle |
| 6 | 0.217931 | 0.000000 | 4.285885 | −2.361769 | Saddle |
| | −0.120440 | 0.000000 | −1.309010 | 0.196551 | Saddle |
| | 0.663420 | 0.713602 | 17.318529 | 120.401859 | **Stable** |
| | −0.179511 | 0.756104 | −1.036050 | −2.478907 | Unstable |
| | −0.021322 | 7.644387 | −0.912218 | 2.607317 | Saddle |
| | 0.006040 | 9.924265 | 0.202829 | −0.232148 | Saddle |
| | −0.108450 | −0.726042 | −1.181799 | −0.262289 | Unstable |
| | −0.074889 | −3.987332 | 3.465577 | −2.593700 | Saddle |
| 7 | 0.097651 | 0.000000 | 1.364058 | −0.440222 | Saddle |
| | −0.080999 | 0.000000 | −0.938512 | 0.113962 | Saddle |
| | 0.120384 | 1.096799 | 2.087750 | 1.190689 | **Stable** |
| | −0.093325 | 1.165708 | −1.119247 | −0.482900 | Unstable |
| | −0.019216 | 7.603181 | −0.809944 | 2.161546 | Saddle |
| | 0.005862 | 9.948807 | 0.212784 | −0.238301 | Saddle |
| | −0.079002 | −0.996971 | −0.904704 | −0.172547 | Unstable |
| | −0.066835 | −3.995538 | 2.276217 | −2.046894 | Saddle |

Table SM.47: Three loop MOMg scheme $SU(3)$ fixed points in the Curci-Ferrari gauge for $0 \leq N_f \leq 7$.

| $N_f$ | $a_\infty$ | $\alpha_\infty$ | $\omega_1$ | $\omega_2$ | Infrared Stability |
|---|---|---|---|---|---|
| 8 | 0.064861 | 0.000000 | 0.737894 | −0.276082 | Saddle |
| | −0.064370 | 0.000000 | −0.726760 | 0.115659 | Saddle |
| | −0.074925 | 1.640844 | −0.893361 | −0.654337 | Unstable |
| | 0.078074 | 1.729775 | $1.037553 + 0.080906i$ | $\omega_1^*$ | **Stable** |
| | −0.017606 | 7.570110 | −0.738452 | 1.867429 | Saddle |
| | 0.005700 | 9.977978 | 0.222556 | −0.244753 | Saddle |
| | −0.063713 | −1.397530 | −0.657419 | −0.183358 | Unstable |
| | −0.059318 | −4.041705 | 1.508793 | −1.633308 | Saddle |
| 9 | 0.047997 | 0.000000 | 0.452324 | −0.224312 | Saddle |
| | −0.054246 | 0.000000 | −0.577766 | 0.127131 | Saddle |
| | −0.071656 | 2.030893 | $-1.044779 + 0.037208i$ | $\omega_1^*$ | Unstable |
| | 0.074090 | 2.243751 | 1.150519 | 1.929714 | **Stable** |
| | −0.016331 | 7.543497 | −0.686264 | 1.661606 | Saddle |
| | 0.005551 | 10.010749 | 0.232176 | −0.251409 | Saddle |
| | −0.052649 | −1.847230 | −0.403795 | −0.229027 | Unstable |
| | −0.052156 | −4.128998 | 1.000679 | −1.301302 | Saddle |
| 10 | 0.037161 | 0.000000 | 0.287998 | −0.193650 | Saddle |
| | −0.047130 | 0.000000 | −0.463256 | 0.139912 | Saddle |
| | −0.084378 | 2.320245 | −1.024011 | −3.745269 | Unstable |
| | 0.106102 | 2.513994 | 1.803711 | 10.416231 | **Stable** |
| | −0.015293 | 7.522247 | −0.647020 | 1.511342 | Saddle |
| | 0.005414 | 10.046341 | 0.241666 | −0.258203 | Saddle |
| | −0.043426 | −2.315486 | $-0.226233 + 0.112100i$ | $\omega_1^*$ | Unstable |
| | −0.045309 | −4.260197 | 0.658740 | −1.024927 | Saddle |
| 11 | 0.029277 | 0.000000 | 0.182697 | −0.166770 | Saddle |
| | −0.041710 | 0.000000 | −0.370824 | 0.151696 | Saddle |
| | −0.014428 | 7.505613 | −0.616919 | 1.398190 | Saddle |
| | 0.005287 | 10.084157 | 0.251038 | −0.265091 | Saddle |
| | −0.035459 | −2.790039 | $-0.156076 + 0.119974i$ | $\omega_1^*$ | Unstable |
| | −0.038832 | −4.440055 | 0.429038 | −0.795503 | Saddle |
| 12 | 0.023018 | 0.000000 | 0.111618 | −0.138971 | Saddle |
| | −0.037345 | 0.000000 | −0.293806 | 0.161408 | Saddle |
| | −0.013694 | 7.493062 | −0.593554 | 1.311029 | Saddle |
| | 0.005168 | 10.123733 | 0.260301 | −0.272037 | Saddle |
| | −0.028558 | −3.266820 | $-0.106170 + 0.098146i$ | $\omega_1^*$ | Unstable |
| | −0.032845 | −4.676981 | 0.278340 | −0.612653 | Saddle |

Table SM.48: Three loop MOMg scheme $SU(3)$ fixed points in the Curci-Ferrari gauge for $8 \leq N_f \leq 12$.

| $N_f$ | $a_\infty$ | $\alpha_\infty$ | $\omega_1$ | $\omega_2$ | Infrared Stability |
|---|---|---|---|---|---|
| 13 | 0.017680 | 0.000000 | 0.062919 | −0.109064 | Saddle |
| | −0.033667 | 0.000000 | −0.228145 | 0.168198 | Saddle |
| | −0.013063 | 7.484203 | −0.575328 | 1.242788 | Saddle |
| | 0.005056 | 10.164697 | 0.269463 | −0.279017 | Saddle |
| | −0.022543 | −3.747910 | $-0.071847 + 0.069964i$ | $\omega_1^*$ | Unstable |
| | −0.027479 | −4.982357 | 0.183305 | −0.476126 | Saddle |
| 14 | 0.012809 | 0.000000 | 0.030337 | −0.077336 | Saddle |
| | −0.030424 | 0.000000 | −0.171141 | 0.171028 | Saddle |
| | −0.012512 | 7.478731 | −0.561137 | 1.188761 | Saddle |
| | 0.004952 | 10.206755 | 0.278528 | −0.286012 | Saddle |
| | −0.017203 | −4.247575 | $-0.047696 + 0.044331i$ | $\omega_1^*$ | Unstable |
| | −0.022821 | −5.365517 | 0.125246 | −0.380475 | Saddle |
| 15 | 0.008032 | 0.000000 | 0.010387 | −0.045066 | Saddle |
| | −0.027396 | 0.000000 | −0.120839 | 0.168226 | Saddle |
| | −0.012027 | 7.476398 | 1.145704 | −0.550192 | Saddle |
| | 0.004853 | 10.249666 | 0.287500 | −0.293008 | Saddle |
| | −0.012363 | −4.799535 | $-0.029962 + 0.023725i$ | $\omega_1^*$ | Unstable |
| | −0.018849 | −5.826901 | 0.089038 | −0.314025 | Saddle |
| 16 | 0.002914 | 0.000000 | 0.001088 | −0.014301 | Saddle |
| | −0.024300 | 0.000000 | −0.075641 | 0.156520 | Saddle |
| | −0.011595 | 7.476996 | 1.111304 | −0.541911 | Saddle |
| | 0.004759 | 10.293237 | 0.296383 | −0.299994 | Saddle |
| | −0.007848 | −5.443983 | $-0.016452 + 0.006638i$ | $\omega_1^*$ | Unstable |
| | 0.003108 | −5.886007 | 0.000830 | 0.018709 | **Stable** |
| | 0.006994 | −6.219624 | −0.004810 | 0.082051 | Saddle |
| | −0.015420 | −6.358049 | 0.064233 | −0.261700 | Saddle |

Table SM.49: Three loop MOMg scheme $SU(3)$ fixed points in the Curci-Ferrari gauge for $13 \leq N_f \leq 16$.

| $N_f$ | $a_\infty$ | $\alpha_\infty$ | $\omega_1$ | $\omega_2$ | Infrared Stability |
|---|---|---|---|---|---|
| 0 | $-0.109677$ | 1.383099 | $-1.206460$ | $-0.237258$ | Unstable |
| 1 | $-0.121476$ | 1.180250 | $-1.253426$ | $-0.347103$ | Unstable |
| 2 | $-0.137091$ | 0.861388 | $-1.322568$ | $-0.497864$ | Unstable |
| 3 | $-0.159142$ | 0.508986 | $-1.433751$ | $-0.718930$ | Unstable |
| 4 | $-0.193210$ | 0.173002 | $-1.630907$ | $-1.105441$ | Unstable |
| 5 | $-0.253394$ | $-0.107514$ | $-1.834461$ | $-2.190962$ | Unstable |
| 6 | $-0.390896$ | $-0.303823$ | $-2.732564$ | $-5.633822$ | Unstable |
| 7 | $-1.066603$ | $-0.410860$ | $-6.826903$ | $-51.801505$ | Unstable |
| 8 | 0.963223 | $-0.451317$ | 5.543599 | $-56.396317$ | Saddle |
| 9 | 0.282170 | $-0.455647$ | 1.435207 | $-6.676079$ | Saddle |
| 10 | 0.146247 | $-0.444967$ | 0.644713 | $-2.483118$ | Saddle |
| | 0.081771 | $-4.742280$ | $0.222481 + 0.293625i$ | $\omega_1^*$ | **Stable** |
| | 0.052312 | $-7.619368$ | 0.162008 | $-0.537242$ | Saddle |
| 11 | 0.088119 | $-0.430186$ | 0.328499 | $-1.242128$ | Saddle |
| | 0.060657 | $-4.773577$ | $0.222545 + 0.182496i$ | $\omega_1^*$ | **Stable** |
| | 0.038554 | $-9.159459$ | 0.146059 | $-0.546162$ | Saddle |
| 12 | 0.055935 | $-0.416406$ | 0.170450 | $-0.689472$ | Saddle |
| | 0.043307 | $-4.932430$ | $0.174963 + 0.089418i$ | $\omega_1^*$ | **Stable** |
| | 0.030897 | $-10.474915$ | 0.133903 | $-0.530531$ | Saddle |
| 13 | 0.035533 | $-0.406183$ | 0.084120 | $-0.389093$ | Saddle |
| | 0.029800 | $-5.120744$ | 0.107161 | 0.140120 | **Stable** |
| | 0.025861 | $-11.675615$ | 0.124813 | $-0.512186$ | Saddle |
| 14 | 0.021460 | $-0.401287$ | 0.036229 | $-0.208086$ | Saddle |
| | 0.019126 | $-5.302003$ | 0.038062 | 0.118135 | **Stable** |
| | 0.022243 | $-12.803936$ | 0.117664 | $-0.494490$ | Saddle |
| 15 | 0.011165 | $-0.403828$ | 0.011279 | $-0.094248$ | Saddle |
| | 0.010462 | $-5.453155$ | 0.011418 | 0.069423 | **Stable** |
| | 0.019494 | $-13.882268$ | 0.111800 | $-0.478042$ | Saddle |
| 16 | 0.003291 | $-0.417578$ | 0.001103 | $-0.023436$ | Saddle |
| | 0.003223 | $-5.550742$ | 0.001104 | 0.021316 | **Stable** |
| | 0.017323 | $-14.924214$ | 0.106835 | $-0.462856$ | Saddle |

Table SM.50: Two loop MOMg scheme $SU(3)$ fixed points in the MAG for $0 \leq N_f \leq 16$.

| $N_f$ | $a_\infty$ | $\alpha_\infty$ | $\omega_1$ | $\omega_2$ | Infrared Stability |
|---|---|---|---|---|---|
| 0 | - | - | - | - | - |
| 1 | - | - | - | - | - |
| 2 | - | - | - | - | - |
| 3 | - | - | - | - | - |
| 4 | - | - | - | - | - |
| 5 | $-0.223165$ | $-4.905614$ | $-16.899574 + 13.535731i$ | $\omega_1^*$ | Unstable |
| | $0.066155$ | $-5.625787$ | $0.500861 + 1.377291i$ | $\omega_1^*$ | **Stable** |
| 6 | $0.263571$ | $-1.160939$ | $4.781310$ | $-18.386573$ | Saddle |
| | $-0.172256$ | $-1.411387$ | $-2.086716$ | $4.364835$ | Saddle |
| | $-0.118628$ | $-4.794817$ | $-2.868213 + 3.513292i$ | $\omega_1^*$ | Unstable |
| | $0.053795$ | $-5.584595$ | $0.267534 + 0.886326i$ | $\omega_1^*$ | **Stable** |
| 7 | $0.090498$ | $-0.924095$ | $1.207317$ | $-1.115280$ | Saddle |
| | $-0.087731$ | $-1.418112$ | $-1.134874$ | $0.524334$ | Saddle |
| | $-0.087062$ | $-4.697580$ | $-1.299021 + 1.501993i$ | $\omega_1^*$ | Unstable |
| | $0.047859$ | $-5.380708$ | $0.202033 + 0.593199i$ | $\omega_1^*$ | **Stable** |
| 8 | $0.058940$ | $-0.743776$ | $0.659212$ | $-0.574769$ | Saddle |
| | $-0.064943$ | $-1.186060$ | $-0.790455$ | $0.262859$ | Saddle |
| | $-0.070536$ | $-4.611365$ | $-0.805681 + 0.757558i$ | $\omega_1^*$ | Unstable |
| | $0.043366$ | $-5.054931$ | $0.188859 + 0.373814i$ | $\omega_1^*$ | **Stable** |
| 9 | $0.043580$ | $-0.624218$ | $0.409796$ | $-0.422838$ | Saddle |
| | $-0.052599$ | $-0.924935$ | $-0.589384$ | $0.232093$ | Saddle |
| | $-0.059787$ | $-4.580227$ | $-0.586277 + 0.434766i$ | $\omega_1^*$ | Unstable |
| | $0.037995$ | $-4.761534$ | $0.184912 + 0.226648i$ | $\omega_1^*$ | **Stable** |
| 10 | $0.033899$ | $-0.544305$ | $0.264565$ | $-0.339202$ | Saddle |
| | $-0.044678$ | $-0.742912$ | $-0.455032$ | $0.235854$ | Saddle |
| | $-0.052033$ | $-4.647743$ | $-0.467614 + 0.305396i$ | $\omega_1^*$ | Unstable |
| | $0.031875$ | $-4.688329$ | $0.164906 + 0.149364i$ | $\omega_1^*$ | **Stable** |

Table SM.51: Three loop MOMg scheme $SU(3)$ fixed points in the MAG for $0 \leq N_f \leq 10$.

| $N_f$ | $a_\infty$ | $\alpha_\infty$ | $\omega_1$ | $\omega_2$ | Infrared Stability |
|---|---|---|---|---|---|
| 11 | 0.026895 | $-0.488788$ | 0.170111 | $-0.275738$ | Saddle |
| | $-0.039020$ | $-0.622314$ | $-0.355625$ | 0.241819 | Saddle |
| | 0.026190 | $-4.789249$ | $0.136174 + 0.102702i$ | $\omega_1^*$ | **Stable** |
| | $-0.046111$ | $-4.809342$ | $-0.391600 + 0.257669i$ | $\omega_1^*$ | Unstable |
| 12 | 0.021325 | $-0.449596$ | 0.105327 | $-0.219575$ | Saddle |
| | $-0.034649$ | $-0.539083$ | $-0.277020$ | 0.244942 | Saddle |
| | 0.021171 | $-4.968311$ | $0.107126 + 0.066067i$ | $\omega_1^*$ | **Stable** |
| | $-0.041372$ | $-5.034183$ | $-0.335640 + 0.234984i$ | $\omega_1^*$ | Unstable |
| 13 | 0.016542 | $-0.422798$ | 0.060186 | $-0.166333$ | Saddle |
| | $-0.031060$ | $-0.479215$ | $-0.212138$ | 0.243998 | Saddle |
| | 0.016638 | $-5.169138$ | $0.080140 + 0.032646i$ | $\omega_1^*$ | **Stable** |
| | $-0.037413$ | $-5.295387$ | $-0.290307 + 0.216175i$ | $\omega_1^*$ | Unstable |
| 14 | 0.012127 | $-0.407119$ | 0.029433 | $-0.114790$ | Saddle |
| | $-0.027940$ | $-0.435102$ | $-0.156949$ | 0.237872 | Saddle |
| | 0.012327 | $-5.355909$ | 0.037773 | 0.072840 | **Stable** |
| | $-0.033971$ | $-5.574945$ | $-0.251162 + 0.194435i$ | $\omega_1^*$ | Unstable |
| 15 | $-0.025037$ | $-0.402875$ | $-0.108876$ | 0.224555 | Saddle |
| | 0.007722 | $-0.403731$ | 0.010226 | $-0.065544$ | Saddle |
| | 0.007915 | $-5.497120$ | 0.011214 | 0.053029 | **Stable** |
| | $-0.030861$ | $-5.860229$ | $-0.215723 + 0.167149i$ | $\omega_1^*$ | Unstable |
| 16 | $-0.022040$ | $-0.381731$ | $-0.066013$ | 0.199799 | Saddle |
| | 0.002865 | $-0.416802$ | 0.001085 | $-0.020495$ | Saddle |
| | 0.002925 | $-5.562587$ | 0.001101 | 0.019448 | **Stable** |
| | $-0.027921$ | $-6.139907$ | $-0.182185 + 0.132059i$ | $\omega_1^*$ | Unstable |

Table SM.52: Three loop MOMg scheme $SU(3)$ fixed points in the MAG for $11 \leq N_f \leq 16$.

| $N_f$ | $a_\infty$ | $\alpha_\infty$ | $\omega_1$ | $\omega_2$ | Infrared Stability |
|---|---|---|---|---|---|
| 0 | $-0.107843$ | 0.000000 | $-1.186275$ | $-0.158561$ | Unstable |
| | $-0.100420$ | 0.524508 | $-1.071865$ | 0.135020 | Saddle |
| | 0.010411 | 13.152600 | $-0.062378$ | 0.421432 | Saddle |
| 1 | $-0.115672$ | 0.000000 | $-1.195274$ | $-0.176651$ | Unstable |
| | $-0.107585$ | 0.529176 | $-1.081287$ | 0.150446 | Saddle |
| | 0.012564 | 11.978164 | $-0.071864$ | 0.467829 | Saddle |
| 2 | $-0.126087$ | 0.000000 | $-1.218841$ | $-0.209237$ | Unstable |
| | $-0.116818$ | 0.555686 | $-1.100933$ | 0.176953 | Saddle |
| | 0.015482 | 10.797643 | $-0.084257$ | 0.526291 | Saddle |
| 3 | $-0.140625$ | 0.000000 | $-1.265625$ | $-0.268866$ | Unstable |
| | $-0.129328$ | 0.613513 | $-1.138312$ | 0.223647 | Saddle |
| | 0.019622 | 9.603542 | $-0.101017$ | 0.603150 | Saddle |
| 4 | $-0.162338$ | 0.000000 | $-1.352814$ | $-0.385315$ | Unstable |
| | $-0.147632$ | 0.719558 | $-1.209709$ | 0.311313 | Saddle |
| | 0.025896 | 8.381822 | $-0.124798$ | 0.711011 | Saddle |
| 5 | $-0.198276$ | 0.000000 | $-1.520115$ | $-0.644361$ | Unstable |
| | $-0.178314$ | 0.907621 | $-1.358564$ | 0.500042 | Saddle |
| | 0.036515 | 7.103158 | $-0.161112$ | 0.880336 | Saddle |
| 6 | $-0.269231$ | 0.000000 | $-1.884615$ | $-1.385686$ | Unstable |
| | $-0.249008$ | 1.262391 | $-1.756848$ | 1.084130 | Saddle |
| | 0.059009 | 5.690447 | $-0.224303$ | 1.217181 | Saddle |
| 7 | $-0.475000$ | 0.000000 | $-3.008333$ | $-5.212492$ | Unstable |
| | $-2.359633$ | 2.247395 | $-9.458117$ | 119.625872 | Saddle |
| | 0.179148 | 3.693536 | $-0.357348$ | 3.106583 | Saddle |
| 8 | $-8.500000$ | 0.000000 | $-48.166667$ | $-2080.205360$ | Unstable |
| 9 | 0.416667 | 0.000000 | 2.083333 | $-6.400386$ | Saddle |
| 10 | 0.175676 | 0.000000 | 0.761261 | $-1.494540$ | Saddle |
| 11 | 0.098214 | 0.000000 | 0.360119 | $-0.630605$ | Saddle |
| 12 | 0.060000 | 0.000000 | 0.180000 | $-0.328685$ | Saddle |
| 13 | 0.037234 | 0.000000 | 0.086879 | $-0.185640$ | Saddle |
| 14 | 0.022124 | 0.000000 | 0.036873 | $-0.104350$ | Saddle |
| | 0.019199 | $-3.718938$ | $0.040359 + 0.019083i$ | $\omega_1^*$ | **Stable** |
| | 0.019368 | $-6.388108$ | 0.053383 | $-0.117395$ | Saddle |
| 15 | 0.011364 | 0.000000 | 0.011364 | $-0.051980$ | Saddle |
| | 0.010692 | $-3.221650$ | 0.011864 | 0.039935 | **Stable** |
| | 0.015028 | $-8.083894$ | 0.051109 | $-0.176883$ | Saddle |
| 16 | 0.003311 | 0.000000 | 0.001104 | $-0.014937$ | Saddle |
| | 0.003259 | $-3.040137$ | 0.001106 | 0.014144 | **Stable** |
| | 0.012174 | $-9.486233$ | 0.046612 | $-0.198161$ | Saddle |

Table SM.53: Two loop MOMq scheme $SU(3)$ fixed points in the linear covariant gauge for $0 \leq N_f \leq 16$.

| $N_f$ | $a_\infty$ | $\alpha_\infty$ | $\omega_1$ | $\omega_2$ | Infrared Stability |
|---|---|---|---|---|---|
| 0 | 0.000789 | 27.599326 | −0.004115 | 0.100522 | Saddle |
| | −0.048186 | −10.626752 | 0.561494 | 46.499313 | **Stable** |
| 1 | 0.000928 | 25.356347 | −0.004480 | 0.109239 | Saddle |
| | −0.052965 | −10.471126 | 0.650242 | 55.516875 | **Stable** |
| 2 | 0.001108 | 23.105636 | −0.004915 | 0.119653 | Saddle |
| | −0.058634 | −10.318804 | 0.759011 | 67.682406 | **Stable** |
| 3 | 0.001347 | 20.843493 | −0.005444 | 0.132336 | Saddle |
| | −0.065498 | −10.169609 | 0.895751 | 84.724394 | **Stable** |
| 4 | 0.463450 | 0.000000 | 18.749865 | 57.840184 | **Stable** |
| | −0.120225 | 0.000000 | −1.261776 | −1.275888 | Unstable |
| | 0.001676 | 18.563656 | −0.006099 | 0.148170 | Saddle |
| | −0.074021 | −10.023385 | 1.073334 | 109.746515 | **Stable** |
| 5 | 0.161196 | 0.000000 | 3.476387 | 1.457551 | **Stable** |
| | −0.088912 | 0.000000 | −1.057642 | −0.445629 | Unstable |
| | 0.002150 | 16.254704 | −0.006928 | 0.168617 | Saddle |
| | −0.084954 | −9.879961 | 1.314052 | 148.783483 | **Stable** |
| 6 | 0.105517 | 0.000000 | 1.766724 | 0.079131 | **Stable** |
| | −0.075807 | 0.000000 | −0.911883 | −0.218127 | Unstable |
| | 0.002879 | 13.893433 | −0.007998 | 0.196365 | Saddle |
| | −0.099604 | −9.739086 | 1.660094 | 214.868461 | **Stable** |
| 7 | 0.079487 | 0.000000 | 1.091084 | −0.143791 | Saddle |
| | −0.068093 | 0.000000 | −0.800686 | −0.108485 | Unstable |
| | −0.067291 | 0.804242 | −0.785007 | 0.071054 | Saddle |
| | −0.065555 | 1.830419 | −0.807364 | −0.195539 | Unstable |
| | 0.069994 | 1.959663 | 1.052189 | 0.431865 | **Stable** |
| | 0.004125 | 11.423558 | −0.009378 | 0.237326 | Saddle |
| | 0.077520 | −1.085495 | 1.013439 | 0.181897 | **Stable** |
| | −0.120501 | −9.600312 | 2.201724 | 340.554261 | **Stable** |
| 8 | 0.063407 | 0.000000 | 0.721295 | −0.189700 | Saddle |
| | −0.062938 | 0.000000 | −0.710653 | −0.041735 | Unstable |
| | −0.062368 | 0.272270 | −0.700759 | 0.038607 | Saddle |
| | −0.055393 | 2.526839 | −0.856731 | −0.379120 | Unstable |
| | 0.038077 | 3.159468 | 0.126365 | 0.801331 | **Stable** |
| | 0.006831 | 8.645201 | −0.010746 | 0.310710 | Saddle |
| | 0.063541 | −1.624601 | 0.691198 | 0.241791 | **Stable** |
| | −0.153305 | −9.462764 | 3.170166 | 626.738510 | **Stable** |
| 9 | 0.051906 | 0.000000 | 0.486729 | −0.189612 | Saddle |
| | −0.059292 | 0.000000 | −0.635110 | 0.004967 | Saddle |
| | −0.048002 | 2.975496 | −0.357705 | −0.957463 | Unstable |
| | −0.059382 | −0.031939 | −0.636583 | −0.005006 | Unstable |
| | 0.053412 | −1.989647 | 0.486461 | 0.235334 | **Stable** |
| | −0.214089 | −9.324643 | 5.360466 | 1521.434436 | **Stable** |

Table SM.54: Three loop MOMq scheme $SU(3)$ fixed points in the linear covariant gauge for $0 \leq N_f \leq 9$.

| $N_f$ | $a_\infty$ | $\alpha_\infty$ | $\omega_1$ | $\omega_2$ | Infrared Stability |
|---|---|---|---|---|---|
| 10 | 0.042853 | 0.000000 | 0.326095 | −0.173917 | Saddle |
| | −0.056679 | 0.000000 | −0.570455 | 0.041073 | Saddle |
| | −0.042345 | 3.345065 | −0.307204 | −1.031021 | Unstable |
| | −0.057575 | −0.263986 | −0.584632 | −0.043561 | Unstable |
| | 0.045054 | −2.279576 | 0.340980 | 0.203465 | **Stable** |
| | −0.375316 | −9.182018 | 13.739858 | 7268.432292 | **Stable** |
| 11 | 0.035202 | 0.000000 | 0.211884 | −0.151840 | Saddle |
| | −0.054867 | 0.000000 | −0.514748 | 0.071399 | Saddle |
| | −0.037783 | 3.678023 | −0.257738 | −1.077095 | Unstable |
| | −0.056703 | −0.456907 | −0.542762 | −0.078898 | Unstable |
| | 0.037600 | −2.524956 | 0.234859 | 0.161027 | **Stable** |
| | −3.048029 | −9.025262 | 706.724575 | 3411401.612173 | **Stable** |
| 12 | 0.028357 | 0.000000 | 0.129936 | −0.126653 | Saddle |
| | −0.053769 | 0.000000 | −0.467171 | 0.098970 | Saddle |
| | −0.033941 | 3.995236 | −0.213830 | −1.103142 | Unstable |
| | −0.056746 | −0.622909 | −0.511369 | −0.113740 | Unstable |
| | 0.030567 | −2.734762 | 0.114118 | 0.159650 | **Stable** |
| | 0.348859 | −8.824271 | 6.230241 | −4335.031090 | Saddle |
| 13 | 0.021939 | 0.000000 | 0.072218 | −0.099677 | Saddle |
| | −0.053405 | 0.000000 | −0.427958 | 0.126285 | Saddle |
| | −0.030585 | 4.310677 | −0.175807 | −1.114167 | Unstable |
| | −0.057870 | −0.766548 | −0.493572 | −0.151459 | Unstable |
| | 0.023664 | −2.903611 | 0.068889 | 0.108181 | **Stable** |
| | 0.096434 | −8.394574 | 0.189748 | −65.665346 | Saddle |
| 14 | 0.015687 | 0.000000 | 0.033752 | −0.071577 | Saddle |
| | −0.053922 | 0.000000 | −0.398775 | 0.156279 | Saddle |
| | −0.027563 | 4.636037 | −0.143260 | −1.113080 | Unstable |
| | −0.060498 | −0.888419 | −0.497778 | −0.197180 | Unstable |
| | 0.016759 | −3.014525 | 0.033421 | 0.071138 | **Stable** |
| | 0.029601 | −7.833650 | 0.050512 | −1.423897 | Saddle |
| 15 | 0.009437 | 0.000000 | 0.011037 | −0.042870 | Saddle |
| | −0.055658 | 0.000000 | −0.383918 | 0.193762 | Saddle |
| | −0.024777 | 4.982772 | −0.115728 | −1.101567 | Unstable |
| | −0.065522 | −0.987214 | −0.546654 | −0.260041 | Unstable |
| | 0.009880 | −3.052463 | 0.011054 | 0.041522 | **Stable** |
| | 0.017283 | −8.405069 | 0.032664 | −0.550762 | Saddle |
| 16 | 0.003136 | 0.000000 | 0.001101 | −0.014144 | Saddle |
| | −0.059301 | 0.000000 | −0.393538 | 0.248917 | Saddle |
| | −0.022160 | 5.363060 | −0.092826 | −1.080715 | Unstable |
| | −0.074870 | −1.063568 | −0.710181 | −0.359075 | Unstable |
| | 0.003189 | −3.026384 | 0.001101 | 0.013944 | **Stable** |
| | 0.010889 | −9.613959 | 0.020653 | −0.362248 | Saddle |

Table SM.55: Three loop MOMq scheme $SU(3)$ fixed points in the linear covariant gauge for $10 \leq N_f \leq 16$.

| $N_f$ | $a_\infty$ | $\alpha_\infty$ | $\omega_1$ | $\omega_2$ | Infrared Stability |
|---|---|---|---|---|---|
| 0 | −0.107843 | 0.000000 | −1.186275 | −0.158561 | Unstable |
| | −0.098874 | 0.601883 | −1.043209 | 0.134450 | Saddle |
| | 0.001254 | 34.192463 | −0.007609 | 0.063332 | Saddle |
| 1 | −0.115672 | 0.000000 | −1.195274 | −0.176651 | Unstable |
| | −0.106012 | 0.595051 | −1.053791 | 0.151033 | Saddle |
| | 0.001445 | 31.692981 | −0.008218 | 0.068074 | Saddle |
| 2 | −0.126087 | 0.000000 | −1.218841 | −0.209237 | Unstable |
| | −0.115122 | 0.609462 | −1.072984 | 0.179217 | Saddle |
| | 0.001684 | 29.185599 | −0.008930 | 0.073632 | Saddle |
| 3 | −0.140625 | 0.000000 | −1.265625 | −0.268866 | Unstable |
| | −0.127330 | 0.651267 | −1.107257 | 0.228944 | Saddle |
| | 0.001991 | 26.667116 | −0.009775 | 0.080258 | Saddle |
| 4 | −0.162338 | 0.000000 | −1.352814 | −0.385315 | Unstable |
| | −0.144854 | 0.729793 | −1.169667 | 0.322987 | Saddle |
| | 0.002394 | 24.132584 | −0.010790 | 0.088320 | Saddle |
| 5 | −0.198276 | 0.000000 | −1.520115 | −0.644361 | Unstable |
| | −0.172836 | 0.859276 | −1.290945 | 0.524698 | Saddle |
| | 0.002941 | 21.573991 | −0.012032 | 0.098404 | Saddle |
| 6 | −0.269231 | 0.000000 | −1.884615 | −1.385686 | Unstable |
| | −0.226749 | 1.061965 | −1.563229 | 1.078643 | Saddle |
| | 0.003719 | 18.977492 | −0.013579 | 0.111499 | Saddle |
| 7 | −0.475000 | 0.000000 | −3.008333 | −5.212492 | Unstable |
| | −0.385797 | 1.374553 | −2.446140 | 3.908295 | Saddle |
| | 0.004897 | 16.316839 | −0.015544 | 0.129479 | Saddle |
| 8 | −8.500000 | 0.000000 | −48.166667 | −2080.205360 | Unstable |
| | 9.165799 | 1.866097 | 51.372663 | 2985.509732 | **Stable** |
| | 0.006875 | 13.534217 | −0.018059 | 0.156564 | Saddle |
| 9 | 0.416667 | 0.000000 | 2.083333 | −6.400386 | Saddle |
| | 0.195908 | 2.717312 | 0.715504 | 2.519692 | **Stable** |
| | 0.010976 | 10.458458 | −0.020950 | 0.206083 | Saddle |
| 10 | 0.175676 | 0.000000 | 0.761261 | −1.494540 | Saddle |
| 11 | 0.098214 | 0.000000 | 0.360119 | −0.630605 | Saddle |
| 12 | 0.060000 | 0.000000 | 0.180000 | −0.328685 | Saddle |
| 13 | 0.037234 | 0.000000 | 0.086879 | −0.185640 | Saddle |
| 14 | 0.022124 | 0.000000 | 0.036873 | −0.104350 | Saddle |
| 15 | 0.011364 | 0.000000 | 0.011364 | −0.051980 | Saddle |
| | 0.011080 | −6.011974 | 0.011097 | 0.040698 | **Stable** |
| | 0.016921 | −9.614908 | 0.050523 | −0.088811 | Saddle |
| 16 | 0.003311 | 0.000000 | 0.001104 | −0.014937 | Saddle |
| | 0.003291 | −5.890246 | 0.001103 | 0.014202 | **Stable** |
| | 0.013873 | −11.594602 | 0.041919 | −0.132720 | Saddle |

Table SM.56: Two loop MOMq scheme $SU(3)$ fixed points in the Curci-Ferrari gauge for $0 \leq N_f \leq 16$.

| $N_f$ | $a_\infty$ | $\alpha_\infty$ | $\omega_1$ | $\omega_2$ | Infrared Stability |
|---|---|---|---|---|---|
| 0 | 0.000158 | 62.474310 | −0.000894 | 0.022316 | Saddle |
| | 0.159197 | −8.229117 | 9.708421 | −242.142654 | Saddle |
| 1 | 0.000182 | 58.017621 | −0.000962 | 0.024008 | Saddle |
| | 0.135321 | −8.125083 | 6.615516 | −132.482983 | Saddle |
| 2 | 0.000212 | 53.556639 | −0.001041 | 0.025980 | Saddle |
| | 0.116725 | −8.022472 | 4.630880 | −75.548067 | Saddle |
| 3 | 0.000251 | 49.089825 | −0.001133 | 0.028309 | Saddle |
| | 0.101744 | −7.922467 | 3.302031 | −44.368612 | Saddle |
| 4 | 0.463450 | 0.000000 | 18.749865 | 57.840184 | **Stable** |
| | −0.120225 | 0.000000 | −1.261776 | −1.275888 | Unstable |
| | 0.000301 | 44.614870 | −0.001243 | 0.031104 | Saddle |
| | 0.089330 | −7.826686 | 2.382932 | −26.606737 | Saddle |
| 5 | 0.161196 | 0.000000 | 3.476387 | 1.457551 | **Stable** |
| | −0.088912 | 0.000000 | −1.057642 | −0.445629 | Unstable |
| | 0.000369 | 40.128150 | −0.001378 | 0.034522 | Saddle |
| | 0.078790 | −7.737351 | 1.731062 | −16.187874 | Saddle |
| 6 | 0.105517 | 0.000000 | 1.766724 | 0.079131 | **Stable** |
| | −0.075807 | 0.000000 | −0.911883 | −0.218127 | Unstable |
| | 0.000463 | 35.623700 | −0.001544 | 0.038807 | Saddle |
| | 0.069641 | −7.657502 | 1.259566 | −9.943347 | Saddle |
| 7 | 0.079487 | 0.000000 | 1.091084 | −0.143791 | Saddle |
| | −0.068093 | 0.000000 | −0.800686 | −0.108485 | Unstable |
| | 0.080573 | 0.938333 | 1.124945 | 0.268925 | **Stable** |
| | 0.000598 | 31.091026 | −0.001755 | 0.044351 | Saddle |
| | 0.077304 | −1.950177 | 0.996925 | 0.330444 | **Stable** |
| | 0.061532 | −7.591338 | 0.913285 | −6.142326 | Saddle |
| 8 | 0.063407 | 0.000000 | 0.721295 | −0.189700 | Saddle |
| | −0.062938 | 0.000000 | −0.710653 | −0.041735 | Unstable |
| | −0.061695 | 0.566542 | −0.689412 | 0.027033 | Saddle |
| | −0.059719 | 1.418303 | −0.670018 | −0.075904 | Unstable |
| | 0.058960 | 1.703146 | 0.677379 | 0.373810 | **Stable** |
| | 0.000806 | 26.509957 | −0.002030 | 0.051847 | Saddle |
| | 0.064053 | −2.560725 | 0.690148 | 0.355984 | **Stable** |
| | 0.054194 | −7.544746 | 0.656008 | −3.803853 | Saddle |

Table SM.57: Three loop MOMq scheme $SU(3)$ fixed points in the Curci-Ferrari gauge for $0 \leq N_f \leq 8$.

| $N_f$ | $a_\infty$ | $\alpha_\infty$ | $\omega_1$ | $\omega_2$ | Infrared Stability |
|---|---|---|---|---|---|
| 9 | 0.051906 | 0.000000 | 0.486729 | −0.189612 | Saddle |
| | −0.059292 | 0.000000 | −0.635110 | 0.004967 | Saddle |
| | −0.052147 | 2.196162 | −0.610396 | −0.240745 | Unstable |
| | 0.041687 | 2.425007 | 0.500575 | 0.240626 | **Stable** |
| | 0.001155 | 21.836295 | −0.002399 | 0.062678 | Saddle |
| | −0.059437 | −0.051990 | −0.637490 | −0.005058 | Unstable |
| | 0.054046 | −3.054338 | 0.482523 | 0.318561 | **Stable** |
| | 0.047413 | −7.526249 | 0.463371 | −2.355528 | Saddle |
| 10 | 0.042853 | 0.000000 | 0.326095 | −0.173917 | Saddle |
| | −0.056679 | 0.000000 | −0.570455 | 0.041073 | Saddle |
| | −0.045912 | 2.699863 | −0.624244 | −0.267752 | Unstable |
| | 0.027602 | 3.319638 | 0.099035 | 0.395201 | **Stable** |
| | 0.001833 | 16.948648 | −0.002895 | 0.080289 | Saddle |
| | −0.057989 | −0.403738 | −0.590662 | −0.045635 | Unstable |
| | 0.045671 | −3.502277 | 0.331905 | 0.263053 | **Stable** |
| | 0.041008 | −7.548878 | 0.318734 | −1.455901 | Saddle |
| 11 | 0.035202 | 0.000000 | 0.211884 | −0.151840 | Saddle |
| | −0.054867 | 0.000000 | −0.514748 | 0.071399 | Saddle |
| | −0.040555 | 3.134255 | −0.233931 | −0.666970 | Unstable |
| | 0.014604 | 5.033905 | 0.018814 | 0.266971 | **Stable** |
| | 0.003793 | 11.252432 | −0.003207 | 0.119916 | Saddle |
| | −0.057400 | −0.679906 | −0.551390 | −0.083032 | Unstable |
| | 0.038154 | −3.932563 | 0.222397 | 0.202316 | **Stable** |
| | 0.034823 | −7.634193 | 0.210695 | −0.898222 | Saddle |
| 12 | 0.028357 | 0.000000 | 0.129936 | −0.126653 | Saddle |
| | −0.053769 | 0.000000 | −0.467171 | 0.098970 | Saddle |
| | −0.035804 | 3.549174 | −0.187622 | −0.702000 | Unstable |
| | −0.057722 | −0.913896 | −0.521150 | −0.119237 | Unstable |
| | 0.031041 | −4.359040 | 0.132427 | 0.155160 | **Stable** |
| | 0.028725 | −7.821260 | 0.131509 | −0.556257 | Saddle |

Table SM.58: Three loop MOMq scheme $SU(3)$ fixed points in the Curci-Ferrari gauge for $9 \leq N_f \leq 12$.

| $N_f$ | $a_\infty$ | $\alpha_\infty$ | $\omega_1$ | $\omega_2$ | Infrared Stability |
|---|---|---|---|---|---|
| 13 | 0.021939 | 0.000000 | 0.072218 | −0.099677 | Saddle |
| | −0.053405 | 0.000000 | −0.427958 | 0.126285 | Saddle |
| | −0.031451 | 3.975800 | −0.143428 | −0.720485 | Unstable |
| | −0.059181 | −1.114317 | −0.503446 | −0.158085 | Unstable |
| | 0.024050 | −4.783367 | 0.074179 | 0.107641 | **Stable** |
| | 0.022644 | −8.185784 | 0.075935 | −0.352293 | Saddle |
| 14 | 0.015687 | 0.000000 | 0.033752 | −0.071577 | Saddle |
| | −0.053922 | 0.000000 | −0.398775 | 0.156279 | Saddle |
| | −0.027332 | 4.445087 | −0.105155 | −0.721398 | Unstable |
| | −0.062267 | −1.278919 | −0.506572 | −0.206274 | Unstable |
| | 0.017042 | −5.188757 | 0.034535 | 0.070715 | **Stable** |
| | 0.016664 | −8.871976 | 0.040072 | −0.236306 | Saddle |
| 15 | 0.009437 | 0.000000 | 0.011037 | −0.042870 | Saddle |
| | −0.055658 | 0.000000 | −0.383918 | 0.193762 | Saddle |
| | −0.023329 | 4.996843 | −0.073922 | −0.704907 | Unstable |
| | −0.067994 | −1.399152 | −0.552686 | −0.277111 | Unstable |
| | 0.010029 | −5.545351 | 0.011166 | 0.041300 | **Stable** |
| | 0.011185 | −10.110528 | 0.019840 | −0.171635 | Saddle |
| 16 | 0.003136 | 0.000000 | 0.001101 | −0.014144 | Saddle |
| | −0.059301 | 0.000000 | −0.393538 | 0.248917 | Saddle |
| | −0.019389 | 5.686553 | −0.050108 | −0.671572 | Unstable |
| | −0.078529 | −1.468615 | −0.715531 | −0.397978 | Unstable |
| | 0.003212 | −5.850425 | 0.001102 | 0.013933 | **Stable** |
| | 0.006866 | −12.145076 | 0.010067 | −0.131190 | Saddle |

Table SM.59: Three loop MOMq scheme $SU(3)$ fixed points in the Curci-Ferrari gauge for $13 \leq N_f \leq 16$.

| $N_f$ | $a_\infty$ | $\alpha_\infty$ | $\omega_1$ | $\omega_2$ | Infrared Stability |
|---|---|---|---|---|---|
| 0 | $-0.108938$ | 1.311930 | $-1.198568$ | $-0.217866$ | Unstable |
| 1 | $-0.119047$ | 1.163898 | $-1.229414$ | $-0.306319$ | Unstable |
| 2 | $-0.132573$ | 1.008287 | $-1.276511$ | $-0.446159$ | Unstable |
| 3 | $-0.151728$ | 0.852220 | $-1.346409$ | $-0.688642$ | Unstable |
| 4 | $-0.181203$ | 0.699959 | $-1.384926$ | $-1.229336$ | Unstable |
| 5 | $-0.232944$ | 0.554065 | $-1.948795 + 0.277625i$ | $\omega_1^*$ | Unstable |
| 6 | $-0.348880$ | 0.416129 | $-2.594464$ | $-5.348860$ | Unstable |
| 7 | $-0.853278$ | 0.287200 | $-5.639210$ | $-38.255431$ | Unstable |
| 8 | 1.124855 | 0.168024 | 6.607879 | $-79.353529$ | Saddle |
| 9 | 0.288339 | 0.059136 | 1.488876 | $-6.295121$ | Saddle |
| 10 | 0.146833 | $-0.039110$ | 0.655156 | $-2.008844$ | Saddle |
| 11 | 0.088191 | $-0.126566$ | 0.332011 | $-0.916372$ | Saddle |
| 12 | 0.056013 | $-0.203322$ | 0.171992 | $-0.485701$ | Saddle |
| 13 | 0.035634 | $-0.269731$ | 0.084791 | $-0.273169$ | Saddle |
| 14 | 0.021543 | $-0.326389$ | 0.036456 | $-0.151946$ | Saddle |
| | 0.018512 | $-6.159115$ | $0.047360 + 0.021765i$ | $\omega_1^*$ | **Stable** |
| | 0.014689 | $-12.833072$ | 0.037846 | $-0.203833$ | Saddle |
| 15 | 0.011208 | $-0.374099$ | 0.011320 | $-0.074906$ | Saddle |
| | 0.010513 | $-5.718031$ | 0.011908 | 0.052660 | **Stable** |
| | 0.011319 | $-15.419119$ | 0.037767 | $-0.227775$ | Saddle |
| 16 | 0.003298 | $-0.413797$ | 0.001103 | $-0.021365$ | Saddle |
| | 0.003244 | $-5.578975$ | 0.001107 | 0.019664 | **Stable** |
| | 0.009224 | $-17.653356$ | 0.036603 | $-0.233917$ | Saddle |

Table SM.60: Two loop MOMq scheme $SU(3)$ fixed points in the MAG for $0 \leq N_f \leq 16$.

| $N_f$ | $a_\infty$ | $\alpha_\infty$ | $\omega_1$ | $\omega_2$ | Infrared Stability |
|---|---|---|---|---|---|
| 0 | 0.006779 | 15.474743 | −0.016250 | 0.535961 | Saddle |
| | 0.047319 | −21.140026 | 3.164171 | −77.627668 | Saddle |
| 1 | 0.012040 | 11.448766 | −0.022295 | 0.793574 | Saddle |
| | 0.045538 | −21.053065 | 2.790223 | −66.512426 | Saddle |
| 2 | 0.033560 | 6.778824 | −0.076145 | 1.813529 | Saddle |
| | 0.043786 | −20.963951 | 2.448264 | −56.791860 | Saddle |
| 3 | −0.665536 | 2.665792 | −15.689446 | −340.701858 | Unstable |
| | 0.042055 | −20.872321 | 2.135472 | −48.285699 | Saddle |
| 4 | −0.075840 | 3.291147 | −1.549964 | −0.516707 | Unstable |
| | 0.040336 | −20.777719 | 1.849360 | −40.839158 | Saddle |
| 5 | −0.048410 | 4.493928 | −1.266585 | −0.251572 | Unstable |
| | 0.038619 | −20.679566 | 1.587738 | −34.319061 | Saddle |
| 6 | −0.036457 | 5.550299 | −0.187178 | −1.171737 | Unstable |
| | 0.119330 | −2.398239 | 1.862012 | −0.657513 | Saddle |
| | 0.129608 | −3.646004 | 2.278040 | 1.210152 | **Stable** |
| | 0.036894 | −20.577117 | 1.348685 | −28.610636 | Saddle |
| 7 | −0.029445 | 6.483814 | −0.149050 | −1.116821 | Unstable |
| | 0.087019 | −1.414583 | 1.158636 | −0.464991 | Saddle |
| | 0.096943 | −4.272717 | 0.910177 | 1.910487 | **Stable** |
| | 0.035146 | −20.469402 | 1.130528 | −23.614862 | Saddle |
| 8 | −0.024599 | 7.364805 | −0.120855 | −1.073686 | Unstable |
| | 0.067519 | −0.911374 | 0.752315 | −0.394390 | Saddle |
| | 0.075989 | −4.636468 | 0.584048 | 1.317206 | **Stable** |
| | 0.033360 | −20.355136 | 0.931831 | −19.246291 | Saddle |
| 9 | −0.020924 | 8.237475 | −0.098905 | −1.034559 | Unstable |
| | 0.054006 | −0.667233 | 0.497658 | −0.342335 | Saddle |
| | 0.061286 | −4.909881 | 0.385468 | 0.884638 | **Stable** |
| | 0.031513 | −20.232594 | 0.751395 | −15.431281 | Saddle |

Table SM.61: Three loop MOMq scheme $SU(3)$ fixed points in the MAG for $0 \leq N_f \leq 9$.

| $N_f$ | $a_\infty$ | $\alpha_\infty$ | $\omega_1$ | $\omega_2$ | Infrared Stability |
|---|---|---|---|---|---|
| 10 | $-0.017981$ | 9.130273 | $-0.081613$ | $-0.996844$ | Unstable |
| | 0.043845 | $-0.537236$ | 0.328935 | $-0.290481$ | Saddle |
| | 0.049928 | $-5.130987$ | 0.257178 | 0.587363 | **Stable** |
| | 0.029577 | $-20.099427$ | 0.588279 | $-12.106627$ | Saddle |
| 11 | $-0.015546$ | 10.062269 | $-0.068010$ | $-0.959744$ | Unstable |
| | 0.035586 | $-0.463038$ | 0.211976 | $-0.240656$ | Saddle |
| | 0.040453 | $-5.311340$ | 0.170527 | 0.382337 | **Stable** |
| | 0.027507 | $-19.952443$ | 0.441854 | $-9.218653$ | Saddle |
| 12 | $-0.013496$ | 11.045490 | $-0.057374$ | $-0.923233$ | Unstable |
| | 0.028421 | $-0.420266$ | 0.129425 | $-0.193323$ | Saddle |
| | 0.032062 | $-5.449734$ | 0.110184 | 0.242308 | **Stable** |
| | 0.025232 | $-19.787516$ | 0.311952 | $-6.723035$ | Saddle |
| 13 | $-0.011756$ | 12.085634 | $-0.049118$ | $-0.887631$ | Unstable |
| | 0.021860 | $-0.397787$ | 0.071832 | $-0.148058$ | Saddle |
| | 0.024313 | $-5.538771$ | 0.066195 | 0.151202 | **Stable** |
| | 0.022628 | $-19.600872$ | 0.199245 | $-4.586462$ | Saddle |
| 14 | $-0.010275$ | 13.182597 | $-0.042740$ | $-0.853372$ | Unstable |
| | 0.015582 | $-0.390539$ | 0.033600 | $-0.104311$ | Saddle |
| | 0.016971 | $-5.576405$ | 0.032969 | 0.095094 | **Stable** |
| | 0.019436 | $-19.401103$ | 0.106411 | $-2.795470$ | Saddle |
| 15 | $-0.009017$ | 14.331539 | $-0.037815$ | $-0.820852$ | Unstable |
| | 0.009372 | $-0.396713$ | 0.011011 | $-0.061715$ | Saddle |
| | 0.009925 | $-5.576887$ | 0.011034 | 0.056072 | **Stable** |
| | 0.015116 | $-19.320511$ | 0.042076 | $-1.406090$ | Saddle |
| 16 | $-0.007949$ | 15.524505 | $-0.033992$ | $-0.790348$ | Unstable |
| | 0.003126 | $-0.416216$ | 0.001100 | $-0.020225$ | Saddle |
| | 0.003192 | $-5.567723$ | 0.001101 | 0.019496 | **Stable** |
| | 0.009942 | $-20.187144$ | 0.018596 | $-0.664811$ | Saddle |

Table SM.62: Three loop MOMq scheme $SU(3)$ fixed points in the MAG for $10 \leq N_f \leq 16$.

| $N_f$ | Type | $\gamma_A$ | $\gamma_c$ | $\gamma_\psi$ | $\rho_m$ |
|---|---|---|---|---|---|
| 8 | - | - | - | - | - |
| 9 | BZ | 4.153646 | $-2.076823$ | 1.793981 | 19.768519 |
| | IRS | 0 | $-2.538034$ | $-1.580138$ | 19.768519 |
| 10 | BZ | 1.118449 | $-0.559224$ | 0.277757 | 4.189838 |
| | IRS | 0 | $-0.822792$ | $-0.666928$ | 4.189838 |
| 11 | BZ | 0.520338 | $-0.260169$ | 0.073953 | 1.613131 |
| | IRS | 0 | $-0.426165$ | $-0.375258$ | 1.613131 |
| 12 | BZ | 0.290250 | $-0.145125$ | 0.022800 | 0.772800 |
| | IRS | 0 | $-0.254627$ | $-0.231054$ | 0.772800 |
| 13 | BZ | 0.171886 | $-0.085943$ | 0.006932 | 0.404469 |
| | IRS | 0 | $-0.158033$ | $-0.144588$ | 0.404469 |
| 14 | BZ | 0.099863 | $-0.049932$ | 0.001795 | 0.212450 |
| | IRS | 0 | $-0.094940$ | $-0.086646$ | 0.212450 |
| 15 | BZ | 0.050894 | $-0.025447$ | 0.000301 | 0.099690 |
| | IRS | 0 | $-0.049590$ | $-0.044885$ | 0.099690 |
| 16 | BZ | 0.014853 | $-0.007426$ | 0.000011 | 0.027187 |
| | IRS | 0 | $-0.014742$ | $-0.013190$ | 0.027187 |

Table SM.63: Two loop $\overline{\text{MS}}$ scheme $SU(3)$ linear covariant gauge critical exponents.

| $N_f$ | Type | $\gamma_A$ | $\gamma_c$ | $\gamma_\psi$ | $\rho_m$ |
|---|---|---|---|---|---|
| 8 | BZ | 0.176683 | $-0.088341$ | 0.295688 | 2.179000 |
| | IRS | 0 | $-0.101414$ | 0.175278 | 2.179000 |
| 9 | BZ | 0.193341 | $-0.096670$ | 0.090126 | 1.061659 |
| | IRS | 0 | $-0.131133$ | $-0.053277$ | 1.061659 |
| 10 | BZ | 0.175883 | $-0.087941$ | 0.031336 | 0.646806 |
| | IRS | 0 | $-0.134414$ | $-0.107533$ | 0.646806 |
| 11 | BZ | 0.151892 | $-0.075946$ | 0.010955 | 0.439241 |
| | IRS | 0 | $-0.126326$ | $-0.114398$ | 0.439241 |
| 12 | BZ | 0.125974 | $-0.062987$ | 0.003509 | 0.311751 |
| | IRS | 0 | $-0.111280$ | $-0.103668$ | 0.311751 |
| 13 | BZ | 0.099007 | $-0.049504$ | 0.000920 | 0.220154 |
| | IRS | 0 | $-0.091342$ | $-0.085041$ | 0.220154 |
| 14 | BZ | 0.071194 | $-0.035597$ | 0.000163 | 0.146369 |
| | IRS | 0 | $-0.067800$ | $-0.062448$ | 0.146369 |
| 15 | BZ | 0.042753 | $-0.021377$ | 0.000015 | 0.082573 |
| | IRS | 0 | $-0.041686$ | $-0.037857$ | 0.082573 |
| 16 | BZ | 0.014138 | $-0.007069$ | 0.000002 | 0.025833 |
| | IRS | 0 | $-0.014034$ | $-0.012561$ | 0.025833 |

Table SM.64: Three loop $\overline{\text{MS}}$ scheme $SU(3)$ linear covariant gauge critical exponents.

| $N_f$ | Type | $\gamma_A$ | $\gamma_c$ | $\gamma_\psi$ | $\rho_m$ |
|---|---|---|---|---|---|
| 8 | (IRS)/BZ | −0.595200 | 0.297600 | −0.095887 | −1.562280 |
| 9 | BZ | −0.017807 | 0.008903 | −0.048726 | −0.143490 |
| 10 | BZ | 0.096514 | −0.048257 | −0.026915 | 0.155885 |
| | IRS | 0 | −0.070828 | −0.098415 | 0.155885 |
| 11 | BZ | 0.125835 | −0.062918 | −0.012892 | 0.249686 |
| | IRS | 0 | −0.105421 | −0.115454 | 0.249686 |
| 12 | BZ | 0.121873 | −0.060936 | −0.005073 | 0.253328 |
| | IRS | 0 | −0.109067 | −0.108915 | 0.253328 |
| 13 | BZ | 0.101310 | −0.050655 | −0.001559 | 0.209757 |
| | IRS | 0 | −0.094220 | −0.089777 | 0.209757 |
| 14 | BZ | 0.073373 | −0.036686 | −0.000337 | 0.147421 |
| | IRS | 0 | −0.070098 | −0.064964 | 0.147421 |
| 15 | BZ | 0.043478 | −0.021739 | −0.000034 | 0.083600 |
| | IRS | 0 | −0.042422 | −0.038564 | 0.083600 |
| 16 | BZ | 0.014174 | −0.007087 | 0.000001 | 0.025895 |
| | IRS | 0 | −0.014069 | −0.012594 | 0.025895 |

Table SM.65: Four loop $\overline{\text{MS}}$ scheme $SU(3)$ linear covariant gauge critical exponents.

| $N_f$ | Type | $\gamma_A$ | $\gamma_c$ | $\gamma_\psi$ | $\rho_m$ |
|---|---|---|---|---|---|
| 8 | - | - | - | - | - |
| 9 | - | - | - | - | - |
| 10 | - | - | - | - | - |
| 11 | - | - | - | - | - |
| 12 | - | - | - | - | - |
| 13 | BZ | 0.122684 | −0.061342 | −0.001436 | 0.238701 |
| | IRS | 0 | −0.115113 | −0.109348 | 0.238701 |
| 14 | BZ | 0.076782 | −0.038391 | −0.000170 | 0.154060 |
| | IRS | 0 | −0.073395 | −0.067884 | 0.154060 |
| 15 | BZ | 0.043850 | −0.021925 | −0.000019 | 0.084340 |
| | IRS | 0 | −0.042786 | −0.038884 | 0.084340 |
| 16 | BZ | 0.014178 | −0.007089 | 0.000001 | 0.025903 |
| | IRS | 0 | −0.014074 | −0.012597 | 0.025903 |

Table SM.66: Five loop $\overline{\text{MS}}$ scheme $SU(3)$ linear covariant gauge critical exponents.

| $N_f$ | Type | $\gamma_A$ | $\gamma_c$ | $\gamma_\psi$ | $\rho_m$ |
|---|---|---|---|---|---|
| 8 | - | - | - | - | - |
| 9 | BZ | 4.153646 | $-2.076823$ | 1.793981 | 19.768519 |
| | IRS | $-1.355339$ | $-2.033009$ | $-2.849135$ | 19.768519 |
| 10 | BZ | 1.118449 | $-0.559224$ | 0.277757 | 4.189838 |
| | IRS | $-0.497322$ | $-0.745983$ | $-1.156792$ | 4.189838 |
| 11 | BZ | 0.520338 | $-0.260169$ | 0.073953 | 1.613131 |
| | IRS | $-0.289313$ | $-0.433969$ | $-0.664499$ | 1.613131 |
| 12 | BZ | 0.290250 | $-0.145125$ | 0.022800 | 0.772800 |
| | IRS | $-0.191143$ | $-0.286714$ | $-0.420940$ | 0.772800 |
| 13 | BZ | 0.171886 | $-0.085943$ | 0.006932 | 0.404469 |
| | IRS | $-0.129128$ | $-0.193693$ | $-0.270575$ | 0.404469 |
| 14 | BZ | 0.099863 | $-0.049932$ | 0.001795 | 0.212450 |
| | IRS | $-0.083276$ | $-0.124914$ | $-0.165961$ | 0.212450 |
| 15 | BZ | 0.050894 | $-0.025447$ | 0.000301 | 0.099690 |
| | IRS | $-0.046156$ | $-0.069234$ | $-0.087676$ | 0.099690 |
| 16 | BZ | 0.014853 | $-0.007426$ | 0.000011 | 0.027187 |
| | IRS | $-0.014422$ | $-0.021633$ | $-0.026191$ | 0.027187 |

Table SM.67: Two loop $\overline{\text{MS}}$ scheme $SU(3)$ Curci-Ferrari gauge critical exponents.

| $N_f$ | Type | $\gamma_A$ | $\gamma_c$ | $\gamma_\psi$ | $\rho_m$ |
|---|---|---|---|---|---|
| 8 | BZ | 0.176683 | $-0.088341$ | 0.295688 | 2.179000 |
| | IRS | $-0.067584$ | $-0.101375$ | 0.127278 | 2.179000 |
| 9 | BZ | 0.193341 | $-0.096670$ | 0.090126 | 1.061659 |
| | IRS | $-0.090313$ | $-0.135470$ | $-0.125421$ | 1.061659 |
| 10 | BZ | 0.175883 | $-0.087941$ | 0.031336 | 0.646806 |
| | IRS | $-0.097064$ | $-0.145596$ | $-0.191691$ | 0.646806 |
| 11 | BZ | 0.151892 | $-0.075946$ | 0.010955 | 0.439241 |
| | IRS | $-0.096303$ | $-0.144454$ | $-0.202326$ | 0.439241 |
| 12 | BZ | 0.125974 | $-0.062987$ | 0.003509 | 0.311751 |
| | IRS | $-0.089656$ | $-0.134484$ | $-0.187751$ | 0.311751 |
| 13 | BZ | 0.099007 | $-0.049504$ | 0.000920 | 0.220154 |
| | IRS | $-0.077623$ | $-0.116434$ | $-0.158385$ | 0.220154 |
| 14 | BZ | 0.071194 | $-0.035597$ | 0.000163 | 0.146369 |
| | IRS | $-0.060582$ | $-0.090873$ | $-0.119302$ | 0.146369 |
| 15 | BZ | 0.042753 | $-0.021377$ | 0.000015 | 0.082573 |
| | IRS | $-0.039041$ | $-0.058561$ | $-0.073881$ | 0.082573 |
| 16 | BZ | 0.014138 | $-0.007069$ | 0.000002 | 0.025833 |
| | IRS | $-0.013738$ | $-0.020607$ | $-0.024940$ | 0.025833 |

Table SM.68: Three loop $\overline{\text{MS}}$ scheme $SU(3)$ Curci-Ferrari gauge critical exponents.

| $N_f$ | Type | $\gamma_A$ | $\gamma_c$ | $\gamma_\psi$ | $\rho_m$ |
|---|---|---|---|---|---|
| 8 | - | - | - | - | - |
| 9 | (BZ) | 8.791607 | −3.026102 | 2.603599 | 19.768519 |
| | IRS | −0.724122 | 0.388339 | −2.714750 | 19.768519 |
| 10 | (BZ) | 1.980957 | −0.807301 | 0.392405 | 4.189838 |
| | IRS | −0.006334 | −0.236891 | −0.853011 | 4.189838 |
| 11 | (BZ) | 0.811461 | −0.381386 | 0.092940 | 1.613131 |
| | IRS | 0.043139 | −0.220809 | −0.443534 | 1.613131 |
| 12 | (BZ) | 0.414151 | −0.218715 | 0.019593 | 0.772800 |
| | IRS | 0.035621 | −0.171335 | −0.272414 | 0.772800 |
| 13 | (BZ) | 0.230993 | −0.133747 | −0.000737 | 0.404469 |
| | IRS | 0.022787 | −0.126007 | −0.176141 | 0.404469 |
| 14 | (BZ) | 0.129083 | −0.080209 | −0.004955 | 0.212450 |
| | IRS | 0.012573 | −0.086243 | −0.110508 | 0.212450 |
| 15 | (BZ) | 0.064206 | −0.042075 | −0.003912 | 0.099690 |
| | IRS | 0.005746 | −0.050102 | −0.059815 | 0.099690 |
| 16 | (BZ) | 0.018468 | −0.012592 | −0.001362 | 0.027187 |
| | IRS | 0.001493 | −0.016242 | −0.018163 | 0.027187 |

Table SM.69: Two loop $\overline{\text{MS}}$ scheme $SU(3)$ MAG critical exponents.

| $N_f$ | Type | $\gamma_A$ | $\gamma_c$ | $\gamma_\psi$ | $\rho_m$ |
|---|---|---|---|---|---|
| 8 | (BZ) | 0.374693 | 0.161641 | 0.489827 | 2.179000 |
| | IRS | −0.042784 | −0.003098 | −0.064876 | 1.061659 |
| | (IRS) | −9.124149 | 1.564490 | −16.490480 | 2.179000 |
| 9 | (BZ) | 0.247184 | −0.044242 | 0.114079 | 1.061659 |
| | IRS | −0.042784 | −0.003098 | −0.064876 | 1.061659 |
| | (IRS) | −3.064659 | 0.207862 | −6.026855 | 1.061659 |
| 10 | (BZ) | 0.210181 | −0.095121 | 0.023153 | 0.646806 |
| | IRS | 0.007792 | −0.074209 | −0.115217 | 0.646806 |
| | (IRS) | −0.979274 | −0.169934 | −2.142705 | 0.646806 |
| 11 | (BZ) | 0.184032 | −0.102846 | −0.001552 | 0.439241 |
| | IRS | 0.013114 | −0.093589 | −0.131558 | 0.439241 |
| 12 | (BZ) | 0.155165 | −0.094095 | −0.007726 | 0.311751 |
| | IRS | 0.011108 | −0.093971 | −0.128012 | 0.311751 |
| 13 | (BZ) | 0.123140 | −0.077901 | −0.007952 | 0.220154 |
| | IRS | 0.008810 | −0.083851 | −0.110302 | 0.220154 |
| 14 | (BZ) | 0.088884 | −0.057836 | −0.006199 | 0.146369 |
| | IRS | 0.006669 | −0.066415 | −0.083384 | 0.146369 |
| 15 | (BZ) | 0.053337 | −0.035544 | −0.003845 | 0.082573 |
| | IRS | 0.004207 | −0.043332 | −0.051470 | 0.082573 |
| 16 | (BZ) | 0.017559 | −0.011995 | −0.001317 | 0.025833 |
| | IRS | 0.001395 | −0.015512 | −0.017340 | 0.025833 |

Table SM.70: Three loop $\overline{\text{MS}}$ scheme $SU(3)$ MAG critical exponents.

| $N_f$ | Type | $\gamma_A$ | $\gamma_c$ | $\gamma_\psi$ | $\rho_m$ |
|---|---|---|---|---|---|
| 9 | BZ | 6.171875 | $-3.085938$ | 1.793981 | 23.356481 |
| 10 | BZ | 1.508081 | $-0.754040$ | 0.277757 | 4.882518 |
| 11 | BZ | 0.651766 | $-0.325883$ | 0.073953 | 1.846779 |
| | IRS | 0 | $-0.163909$ | $-0.144679$ | 0.432450 |
| 12 | BZ | 0.342900 | $-0.171450$ | 0.022800 | 0.866400 |
| | IRS | 0 | $-0.137790$ | $-0.123655$ | 0.341168 |
| 13 | BZ | 0.193548 | $-0.096774$ | 0.006932 | 0.442979 |
| | IRS | 0 | $-0.108182$ | $-0.097979$ | 0.249582 |
| 14 | BZ | 0.108001 | $-0.054000$ | 0.001795 | 0.226917 |
| | IRS | 0 | $-0.076533$ | $-0.069446$ | 0.163790 |
| 15 | BZ | 0.053170 | $-0.026585$ | 0.000301 | 0.103736 |
| | IRS | 0 | $-0.044713$ | $-0.040388$ | 0.088677 |
| 16 | BZ | 0.015057 | $-0.007528$ | 0.000011 | 0.027550 |
| | (IRS) | 0 | $-91.367197$ | 2894.769714 | 7197.354087 |
| | IRS | 0 | $-0.014335$ | $-0.012823$ | 0.026403 |

Table SM.71: Two loop mMOM scheme $SU(3)$ linear covariant gauge critical exponents.

| $N_f$ | Type | $\gamma_A$ | $\gamma_c$ | $\gamma_\psi$ | $\rho_m$ |
|---|---|---|---|---|---|
| 8 | BZ | 0.712285 | −0.356143 | 0.122653 | 2.317969 |
| | (IRS) | 0 | −0.869483 | 3.672944 | 9.044054 |
| 9 | BZ | 0.406353 | −0.203177 | 0.042526 | 1.191042 |
| | (IRS) | 0 | −0.138769 | 2.011884 | 3.329677 |
| 10 | BZ | 0.275001 | −0.137501 | 0.016702 | 0.734781 |
| | (IRS) | 0 | 0.066624 | 1.466664 | 1.617427 |
| 11 | BZ | 0.199789 | −0.099894 | 0.006576 | 0.492300 |
| | (IRS) | 0 | 0.158099 | 1.193988 | 0.804280 |
| | (IRS) | 0 | 5.263439 | −20.472913 | −8.104262 |
| | IRS | 0 | −0.177596 | −0.174859 | 0.475825 |
| 12 | BZ | 0.148283 | −0.074142 | 0.002376 | 0.340313 |
| | (IRS) | 0 | 0.209297 | 1.026036 | 0.312490 |
| | IRS | 0 | −0.132536 | −0.126333 | 0.323759 |
| 13 | BZ | 0.108285 | −0.054143 | 0.000708 | 0.233293 |
| | (IRS) | 0 | 0.242465 | 0.908042 | −0.038344 |
| | IRS | 0 | −0.099736 | −0.093436 | 0.225995 |
| 14 | BZ | 0.074248 | −0.037124 | 0.000146 | 0.151029 |
| | (IRS) | 0 | 0.266495 | 0.816547 | −0.323621 |
| | IRS | 0 | −0.070435 | −0.064967 | 0.148741 |
| 15 | BZ | 0.043354 | −0.021677 | 0.000017 | 0.083547 |
| | (IRS) | 0 | 0.285685 | 0.739247 | −0.583029 |
| | IRS | 0 | −0.042179 | −0.038314 | 0.083151 |
| 16 | BZ | 0.014158 | −0.007079 | 0.000002 | 0.025868 |
| | (IRS) | 0 | 0.302482 | 0.668239 | −0.843203 |
| | IRS | 0 | −0.014050 | −0.012576 | 0.025858 |

Table SM.72: Three loop mMOM scheme $SU(3)$ linear covariant gauge critical exponents.

| $N_f$ | Type | $\gamma_A$ | $\gamma_c$ | $\gamma_\psi$ | $\rho_m$ |
|---|---|---|---|---|---|
| 8 | BZ | 0.474778 | −0.237389 | −0.017956 | 2.025675 |
| | (IRS) | 0 | −2.258175 | −60.188725 | 260.687360 |
| | IRS | 0 | −0.265079 | −0.226746 | 1.044736 |
| 9 | BZ | 0.292463 | −0.146232 | −0.010391 | 0.979184 |
| | (IRS) | 0 | 0.001655 | −2.579132 | 7.594993 |
| | IRS | 0 | −0.222793 | −0.215257 | 0.836272 |
| 10 | BZ | 0.218958 | −0.109479 | −0.006569 | 0.620806 |
| | (IRS) | 0 | 0.117721 | −1.072557 | 1.658957 |
| | IRS | 0 | −0.184374 | −0.182289 | 0.593885 |
| 11 | BZ | 0.173654 | −0.086827 | −0.003834 | 0.436592 |
| | (IRS) | 0 | 0.154522 | −0.702656 | 0.071329 |
| | IRS | 0 | −0.154669 | −0.151401 | 0.434220 |
| 12 | BZ | 0.137930 | −0.068965 | −0.001939 | 0.317156 |
| | (IRS) | 0 | 0.171764 | −0.572375 | −0.740644 |
| | IRS | 0 | −0.127538 | −0.122541 | 0.320300 |
| 13 | BZ | 0.105460 | −0.052730 | −0.000786 | 0.226367 |
| | (IRS) | 0 | 0.180910 | −0.539644 | −1.365889 |
| | IRS | 0 | −0.099963 | −0.094153 | 0.229135 |
| 14 | BZ | 0.074090 | −0.037045 | −0.000220 | 0.150241 |
| | (IRS) | 0 | 0.184904 | −0.573180 | −2.017939 |
| | IRS | 0 | −0.071427 | −0.066024 | 0.151374 |
| 15 | BZ | 0.043538 | −0.021769 | −0.000027 | 0.083816 |
| | IRS | 0 | −0.042586 | −0.038701 | 0.084007 |
| 16 | BZ | 0.014174 | −0.007087 | 0.000001 | 0.025896 |
| | IRS | 0 | −0.014072 | −0.012595 | 0.025899 |

Table SM.73: Four loop mMOM scheme $SU(3)$ linear covariant gauge critical exponents.

| $N_f$ | Type | $\gamma_A$ | $\gamma_c$ | $\gamma_\psi$ | $\rho_m$ |
|---|---|---|---|---|---|
| 8 | BZ | 0.249221 | −0.124610 | −0.001137 | 1.005585 |
| | (IRS) | 0 | 2.952013 | 6.488203 | 20.134644 |
| | IRS | 0 | −0.189463 | −0.182394 | 0.692361 |
| 9 | BZ | 0.202835 | −0.101418 | −0.005582 | 0.672233 |
| | (IRS) | 0 | 0.575398 | 0.816390 | 0.424152 |
| | IRS | 0 | −0.166196 | −0.162738 | 0.551290 |
| 10 | BZ | 0.178382 | −0.089191 | −0.005186 | 0.503784 |
| | (IRS) | 0 | 0.414674 | 0.449910 | −1.079122 |
| | IRS | 0 | −0.151697 | −0.148790 | 0.450991 |
| 11 | BZ | 0.158660 | −0.079330 | −0.003476 | 0.395544 |
| | (IRS) | 0 | 0.325593 | 0.276743 | −1.666897 |
| | IRS | 0 | −0.139217 | −0.135229 | 0.373631 |
| 12 | BZ | 0.135918 | −0.067959 | −0.001749 | 0.309177 |
| | (IRS) | 0 | 0.227143 | 0.131599 | −2.007590 |
| | IRS | 0 | −0.123246 | −0.117907 | 0.302656 |
| 13 | BZ | 0.107263 | −0.053632 | −0.000633 | 0.228539 |
| | IRS | 0 | −0.100243 | −0.094248 | 0.227759 |
| 14 | BZ | 0.075242 | −0.037621 | −0.000158 | 0.152168 |
| | IRS | 0 | −0.071998 | −0.066518 | 0.152228 |
| 15 | BZ | 0.043759 | −0.021879 | −0.000019 | 0.084206 |
| | IRS | 0 | −0.042706 | −0.038808 | 0.084220 |
| 16 | BZ | 0.014178 | −0.007089 | 0.000001 | 0.025902 |
| | IRS | 0 | −0.014073 | −0.012597 | 0.025902 |

Table SM.74: Five loop mMOM scheme $SU(3)$ linear covariant gauge critical exponents.

| $N_f$ | Type | $\gamma_A$ | $\gamma_c$ | $\gamma_\psi$ | $\rho_m$ |
|---|---|---|---|---|---|
| 8 | - | - | - | - | - |
| 9 | BZ | 5.817419 | $-4.680990$ | 1.793981 | 29.027778 |
| | (IRS) | 0 | 1.570016 | 28.136864 | 44.532366 |
| 10 | BZ | 1.523369 | $-0.960430$ | 0.277757 | 5.616346 |
| | (IRS) | 0 | 0.794732 | 6.637821 | 8.967722 |
| 11 | BZ | 0.666726 | $-0.366276$ | 0.073953 | 1.990398 |
| | (IRS) | 0 | 0.501850 | 2.838337 | 3.274273 |
| 12 | BZ | 0.346950 | $-0.177525$ | 0.022800 | 0.888000 |
| | (IRS) | 0 | 0.355315 | 1.534977 | 1.492824 |
| 13 | BZ | 0.192463 | $-0.095647$ | 0.006932 | 0.438974 |
| | (IRS) | 0 | 0.267722 | 0.936275 | 0.748855 |
| 14 | BZ | 0.105959 | $-0.052379$ | 0.001795 | 0.221152 |
| | (IRS) | 0 | 0.206413 | 0.603742 | 0.380389 |
| | IRS | 0 | $-0.108380$ | $-0.104932$ | 0.225962 |
| 15 | BZ | 0.052003 | $-0.025835$ | 0.000301 | 0.101067 |
| | (IRS) | 0 | 0.153927 | 0.382828 | 0.174164 |
| | IRS | 0 | $-0.051262$ | $-0.047124$ | 0.101429 |
| 16 | BZ | 0.014888 | $-0.007437$ | 0.000011 | 0.027226 |
| | (IRS) | 0 | 0.090324 | 0.189610 | 0.046578 |
| | IRS | 0 | $-0.014786$ | $-0.013250$ | 0.027231 |

Table SM.75: Two loop RI′ scheme $SU(3)$ linear covariant gauge critical exponents.

| $N_f$ | Type | $\gamma_A$ | $\gamma_c$ | $\gamma_\psi$ | $\rho_m$ |
|---|---|---|---|---|---|
| 8 | BZ | 1.969208 | −0.840848 | 0.417516 | 6.218224 |
| | (IRS) | 0 | −0.802910 | 3.537411 | 9.309335 |
| 9 | BZ | 0.961698 | −0.303232 | 0.114563 | 2.227195 |
| | (IRS) | 0 | −0.209281 | 1.656031 | 3.601901 |
| 10 | BZ | 0.527751 | −0.152657 | 0.035491 | 1.035691 |
| | (IRS) | 0 | −0.048009 | 0.947492 | 1.755827 |
| 11 | BZ | 0.309329 | −0.096292 | 0.010810 | 0.571757 |
| | (IRS) | 0 | 0.010831 | 0.622941 | 0.988692 |
| 12 | BZ | 0.190370 | −0.068839 | 0.002878 | 0.354129 |
| | (IRS) | 0 | 0.039212 | 0.455543 | 0.612727 |
| 13 | BZ | 0.121177 | −0.050884 | 0.000557 | 0.231734 |
| | (IRS) | 0 | 0.056824 | 0.357346 | 0.397958 |
| | IRS | 0 | −0.110919 | −0.119632 | 0.242113 |
| 14 | BZ | 0.076742 | −0.035819 | 0.000043 | 0.148685 |
| | (IRS) | 0 | 0.067946 | 0.286092 | 0.253423 |
| | IRS | 0 | −0.071055 | −0.068592 | 0.149260 |
| 15 | BZ | 0.043455 | −0.021392 | −0.000003 | 0.082807 |
| | (IRS) | 0 | 0.070279 | 0.216611 | 0.140469 |
| | IRS | 0 | −0.042049 | −0.038568 | 0.082807 |
| 16 | BZ | 0.014147 | −0.007069 | 0.000002 | 0.025836 |
| | (IRS) | 0 | 0.053490 | 0.123017 | 0.043647 |
| | IRS | 0 | −0.014038 | −0.012569 | 0.025835 |

Table SM.76: Three loop RI′ scheme $SU(3)$ linear covariant gauge critical exponents.

| $N_f$ | Type | $\gamma_A$ | $\gamma_c$ | $\gamma_\psi$ | $\rho_m$ |
|---|---|---|---|---|---|
| 8 | BZ | 6.471485 | −0.141493 | −0.216872 | 10.793654 |
| | (IRS) | 0 | −2.424696 | 3.827038 | 19.536414 |
| 9 | BZ | 1.758067 | 0.145285 | −0.189162 | 1.462828 |
| | (IRS) | 0 | −0.419659 | 0.935252 | 3.663383 |
| 10 | BZ | 0.655285 | 0.059319 | −0.099279 | 0.342432 |
| | (IRS) | 0 | −0.121571 | 0.388783 | 1.145796 |
| 11 | BZ | 0.287141 | −0.011344 | −0.042769 | 0.221298 |
| | (IRS) | 0 | −0.056209 | 0.264999 | 0.589514 |
| | IRS | 0 | −0.020924 | −0.095855 | 0.186593 |
| 12 | BZ | 0.159018 | −0.042487 | −0.014862 | 0.224515 |
| | (IRS) | 0 | −0.025747 | 0.250893 | 0.442411 |
| | IRS | 0 | −0.082487 | −0.104959 | 0.209696 |
| 13 | BZ | 0.107236 | −0.045861 | −0.003945 | 0.199534 |
| | (IRS) | 0 | 0.006053 | 0.249136 | 0.348713 |
| | IRS | 0 | −0.087072 | −0.087682 | 0.196374 |
| 14 | BZ | 0.073867 | −0.035894 | −0.000711 | 0.145441 |
| | (IRS) | 0 | 0.033897 | 0.227024 | 0.245013 |
| | IRS | 0 | −0.068745 | −0.064264 | 0.144981 |
| 15 | BZ | 0.043484 | −0.021684 | −0.000059 | 0.083448 |
| | (IRS) | 0 | 0.049227 | 0.181022 | 0.139471 |
| | IRS | 0 | −0.042316 | −0.038493 | 0.083421 |
| 16 | BZ | 0.014174 | −0.007087 | 0.000001 | 0.025894 |
| | (IRS) | 0 | 0.043509 | 0.105463 | 0.043333 |
| | IRS | 0 | −0.014069 | −0.012593 | 0.025894 |

Table SM.77: Four loop RI′ scheme $SU(3)$ linear covariant gauge critical exponents.

| $N_f$ | Type | $\gamma_A$ | $\gamma_c$ | $\gamma_\psi$ | $\gamma_m$ |
|---|---|---|---|---|---|
| 8 | - | - | - | - | - |
| 9 | - | - | - | - | - |
| 10 | - | - | - | - | - |
| 11 | - | - | - | - | - |
| 12 | - | - | - | - | - |
| 13 | BZ | 0.070465 | −0.051662 | −0.004040 | 0.187491 |
| | (IRS) | 0 | −0.033365 | 0.181740 | 0.313061 |
| | IRS | 0 | −0.081046 | −0.060264 | 0.187045 |
| 14 | BZ | 0.073887 | −0.037954 | −0.000270 | 0.151600 |
| | (IRS) | 0 | 0.016256 | 0.203936 | 0.249187 |
| | IRS | 0 | −0.071499 | −0.064958 | 0.151500 |
| 15 | BZ | 0.043744 | −0.021913 | −0.000020 | 0.084266 |
| | (IRS) | 0 | 0.038957 | 0.163924 | 0.138931 |
| | IRS | 0 | −0.042724 | −0.038782 | 0.084269 |
| 16 | BZ | 0.014178 | −0.007089 | 0.000001 | 0.025902 |
| | (IRS) | 0 | 0.038776 | 0.097100 | 0.043049 |
| | IRS | 0 | −0.014074 | −0.012597 | 0.025902 |

Table SM.78: Five loop RI′ scheme $SU(3)$ linear covariant gauge critical exponents.

| $N_f$ | Type | $\gamma_A$ | $\gamma_c$ | $\gamma_\psi$ | $\rho_m$ |
|---|---|---|---|---|---|
| 9 | BZ | 6.559457 | −1.341820 | 1.793981 | 9.016606 |
| 10 | BZ | 1.485115 | −0.443998 | 0.277757 | 2.526293 |
| | (IRS) | 0 | −18.815949 | 73.368336 | −41.791157 |
| 11 | BZ | 0.615875 | −0.228978 | 0.073953 | 1.170622 |
| | (IRS) | 0 | −2.116580 | 9.894103 | −1.966910 |
| 12 | BZ | 0.318789 | −0.135284 | 0.022800 | 0.636553 |
| | (IRS) | 0 | −0.705376 | 4.178601 | 0.318714 |
| | IRS | 0 | −0.172893 | −0.176307 | 0.306141 |
| 13 | BZ | 0.180136 | −0.082846 | 0.006932 | 0.363130 |
| | (IRS) | 0 | −0.308539 | 2.478980 | 0.691704 |
| | IRS | 0 | −0.138099 | −0.135299 | 0.270434 |
| 14 | BZ | 0.101809 | −0.049083 | 0.001795 | 0.201785 |
| | (IRS) | 0 | −0.142972 | 1.729998 | 0.741307 |
| | IRS | 0 | −0.092263 | −0.086901 | 0.185871 |
| 15 | BZ | 0.051152 | −0.025288 | 0.000301 | 0.097913 |
| | (IRS) | 0 | −0.058429 | 1.325349 | 0.714344 |
| | IRS | 0 | −0.049486 | −0.045233 | 0.096541 |
| 16 | BZ | 0.014853 | −0.007418 | 0.000011 | 0.027124 |
| | (IRS) | 0 | −0.009651 | 1.077437 | 0.668925 |
| | IRS | 0 | −0.014749 | −0.013209 | 0.027124 |

Table SM.79: Two loop MOMc scheme $SU(3)$ linear covariant gauge critical exponents.

| $N_f$ | Type | $\gamma_A$ | $\gamma_c$ | $\gamma_\psi$ | $\rho_m$ |
|---|---|---|---|---|---|
| 8 | BZ | 0.539222 | −0.227391 | 0.047982 | 0.170883 |
| | (IRS) | 0 | 0.822621 | −1.002580 | −27.398080 |
| | IRS | 0 | −0.622517 | −0.425194 | 1.134986 |
| 9 | BZ | 0.329837 | −0.149574 | 0.017904 | 0.375534 |
| | (IRS) | 0 | 0.391474 | −0.086183 | −9.428263 |
| | IRS | 0 | −0.347993 | −0.304238 | 0.754394 |
| 10 | BZ | 0.233644 | −0.110954 | 0.006969 | 0.377682 |
| | (IRS) | 0 | 0.277219 | 0.102546 | −4.979258 |
| | IRS | 0 | −0.241319 | −0.224706 | 0.544544 |
| 11 | BZ | 0.176390 | −0.086067 | 0.002517 | 0.330763 |
| | (IRS) | 0 | 0.228272 | 0.166763 | −3.142147 |
| | IRS | 0 | −0.179505 | −0.169441 | 0.408303 |
| 12 | BZ | 0.135538 | −0.067109 | 0.000730 | 0.270097 |
| | (IRS) | 0 | 0.202150 | 0.193153 | −2.170112 |
| | IRS | 0 | −0.136076 | −0.128086 | 0.305591 |
| 13 | BZ | 0.102106 | −0.050907 | 0.000115 | 0.206167 |
| | (IRS) | 0 | 0.186388 | 0.203886 | −1.568987 |
| | IRS | 0 | −0.101443 | −0.094591 | 0.220930 |
| 14 | BZ | 0.071889 | −0.035931 | −0.000017 | 0.142818 |
| | (IRS) | 0 | 0.176148 | 0.206352 | −1.150713 |
| | IRS | 0 | −0.071000 | −0.065379 | 0.147737 |
| 15 | BZ | 0.042821 | −0.021412 | −0.000007 | 0.082094 |
| | (IRS) | 0 | 0.169193 | 0.203158 | −0.827549 |
| | IRS | 0 | −0.042282 | −0.038392 | 0.083079 |
| 16 | BZ | 0.014138 | −0.007069 | 0.000001 | 0.025826 |
| | (IRS) | 0 | 0.164339 | 0.194794 | −0.550086 |
| | IRS | 0 | −0.014052 | −0.012578 | 0.025860 |

Table SM.80: Three loop MOMc scheme $SU(3)$ linear covariant gauge critical exponents.

| $N_f$ | Type | $\gamma_A$ | $\gamma_c$ | $\gamma_\psi$ | $\rho_m$ |
|---|---|---|---|---|---|
| 9 | BZ | $-6.816830$ | $-0.183639$ | 1.793981 | 4.898631 |
| | (IRS) | 0 | 1.805887 | 13.765601 | $-32.911760$ |
| 10 | BZ | $-1.469864$ | $-0.238114$ | 0.277757 | 1.794262 |
| | (IRS) | 0 | 0.315309 | 2.805440 | $-3.632455$ |
| 11 | BZ | $-0.592042$ | $-0.164628$ | 0.073953 | 0.941822 |
| | (IRS) | 0 | 0.151402 | 1.313020 | $-0.697130$ |
| | IRS | 0 | $-0.071425$ | $-0.107237$ | 0.112278 |
| 12 | BZ | $-0.302779$ | $-0.111268$ | 0.022800 | 0.551163 |
| | (IRS) | 0 | 0.110962 | 0.834012 | $-0.024288$ |
| | IRS | 0 | $-0.070007$ | $-0.101960$ | 0.110359 |
| 13 | BZ | $-0.171230$ | $-0.073598$ | 0.006932 | 0.330246 |
| | (IRS) | 0 | 0.097846 | 0.618438 | 0.180170 |
| | IRS | 0 | $-0.066527$ | $-0.093143$ | 0.102873 |
| 14 | BZ | $-0.097697$ | $-0.045818$ | 0.001795 | 0.190175 |
| | (IRS) | 0 | 0.093078 | 0.501230 | 0.247944 |
| | IRS | 0 | $-0.058988$ | $-0.078817$ | 0.087186 |
| 15 | BZ | $-0.049812$ | $-0.024426$ | 0.000301 | 0.094850 |
| | (IRS) | 0 | 0.091276 | 0.429153 | 0.268001 |
| | IRS | 0 | $-0.044374$ | $-0.056402$ | 0.061051 |
| 16 | BZ | $-0.014717$ | $-0.007345$ | 0.000011 | 0.026864 |
| | (IRS) | 0 | 0.090593 | 0.380798 | 0.269721 |
| | IRS | 0 | $-0.018666$ | $-0.022612$ | 0.023355 |

Table SM.81: Two loop MOMc scheme $SU(3)$ Curci-Ferrari gauge critical exponents.

| $N_f$ | Type | $\gamma_A$ | $\gamma_c$ | $\gamma_\psi$ | $\rho_m$ |
|---|---|---|---|---|---|
| 8 | BZ | $-0.330323$ | $-0.191580$ | 0.007528 | 0.137041 |
| | (IRS) | 0 | $-0.040892$ | 0.102395 | $-0.994712$ |
| | IRS | 0 | $-0.822281$ | $-0.574560$ | 0.776123 |
| 9 | BZ | $-0.240091$ | $-0.133464$ | 0.002704 | 0.306029 |
| | (IRS) | 0 | 0.003384 | 0.147923 | $-0.471734$ |
| | IRS | 0 | $-0.541331$ | $-0.439621$ | 0.684557 |
| 10 | BZ | $-0.188899$ | $-0.102092$ | 0.000514 | 0.326369 |
| | (IRS) | 0 | 0.028004 | 0.173992 | $-0.254634$ |
| | IRS | 0 | $-0.399200$ | $-0.360987$ | 0.582751 |
| 11 | BZ | $-0.153163$ | $-0.080911$ | $-0.000309$ | 0.298706 |
| | (IRS) | 0 | 0.044654 | 0.192948 | $-0.142850$ |
| | IRS | 0 | $-0.312859$ | $-0.306670$ | 0.490657 |
| 12 | BZ | $-0.123892$ | $-0.064194$ | $-0.000459$ | 0.252326 |
| | (IRS) | 0 | 0.057411 | 0.209116 | $-0.074662$ |
| | IRS | 0 | $-0.252137$ | $-0.263491$ | 0.407208 |
| 13 | BZ | $-0.096909$ | $-0.049431$ | $-0.000326$ | 0.197780 |
| | (IRS) | 0 | 0.068224 | 0.224669 | $-0.025628$ |
| | IRS | 0 | $-0.202447$ | $-0.223580$ | 0.326803 |
| 14 | BZ | $-0.070077$ | $-0.035343$ | $-0.000140$ | 0.139805 |
| | (IRS) | 0 | 0.078333 | 0.241159 | 0.016759 |
| | IRS | 0 | $-0.151857$ | $-0.177302$ | 0.237937 |
| 15 | BZ | $-0.042456$ | $-0.021275$ | $-0.000025$ | 0.081477 |
| | (IRS) | 0 | 0.088848 | 0.260182 | 0.062111 |
| | IRS | 0 | $-0.074893$ | $-0.092871$ | 0.106324 |
| 16 | BZ | $-0.014126$ | $-0.007064$ | 0.000001 | 0.025806 |
| | (IRS) | 0 | 0.101281 | 0.283939 | 0.123768 |
| | IRS | 0 | $-0.020939$ | $-0.025335$ | 0.026249 |

Table SM.82: Three loop MOMc scheme $SU(3)$ Curci-Ferrari gauge critical exponents.

| $N_f$ | Type | $\gamma_A$ | $\gamma_c$ | $\gamma_\psi$ | $\rho_m$ |
|---|---|---|---|---|---|
| 10 | (BZ) | 5.627662 | −0.365986 | 1.106413 | 3.258964 |
| 11 | BZ | 1.153991 | −0.279318 | 0.136805 | 1.250131 |
| | (IRS) | 974.215588 | −10.931634 | 271.143232 | −491.504350 |
| 12 | (IRS) | 65.246419 | −5.408677 | 19.476890 | −33.138962 |
| | (BZ) | 0.484443 | −0.187110 | 0.025759 | 0.652360 |
| | IRS | 0.020883 | −0.095157 | −0.185533 | 0.289555 |
| 13 | (IRS) | 18.499173 | −2.894417 | 6.027139 | −8.319827 |
| | (BZ) | 0.247763 | −0.123940 | 0.000398 | 0.366591 |
| | IRS | 0.016317 | −0.090164 | −0.150947 | 0.247989 |
| 14 | (IRS) | 8.177347 | −1.878144 | 2.946372 | −2.904424 |
| | (BZ) | 0.132598 | −0.077561 | −0.004726 | 0.202364 |
| | IRS | 0.010482 | −0.074204 | −0.104898 | 0.173045 |
| 15 | (IRS) | 4.492027 | −1.354512 | 1.804956 | −1.057708 |
| | (BZ) | 0.064619 | −0.041585 | −0.003873 | 0.097925 |
| | IRS | 0.005295 | −0.047439 | −0.058506 | 0.092806 |
| 16 | (IRS) | 2.805750 | −1.042350 | 1.262701 | −0.271566 |
| | (BZ) | 0.018463 | −0.012567 | −0.001360 | 0.027114 |
| | IRS | 0.001468 | −0.016044 | −0.017999 | 0.026808 |

Table SM.83: Two loop MOMc scheme $SU(3)$ MAG critical exponents.

| $N_f$ | Type | $\gamma_A$ | $\gamma_c$ | $\gamma_\psi$ | $\rho_m$ |
|---|---|---|---|---|---|
| 8 | (BZ) | 0.411564 | −0.380500 | −0.043446 | 0.400525 |
| 9 | (BZ) | 0.295832 | −0.240449 | −0.034696 | 0.409975 |
| | IRS | −2715.990473 | −15974.919978 | −7524.837593 | 9467.421651 |
| 10 | (BZ) | 0.234670 | −0.175561 | −0.025879 | 0.372691 |
| | IRS | −56.221412 | −301.361636 | −170.525780 | 231.933695 |
| 11 | (BZ) | 0.191903 | −0.135957 | −0.019136 | 0.320416 |
| | IRS | −11.249839 | −57.735060 | −38.212415 | 54.336768 |
| 12 | (BZ) | 0.155944 | −0.106659 | −0.014011 | 0.262295 |
| | IRS | −3.920648 | −19.973268 | −15.156930 | 22.089447 |
| 13 | (BZ) | 0.122059 | −0.081811 | −0.009984 | 0.201901 |
| | IRS | −1.731560 | −9.032689 | −7.739827 | 11.403803 |
| 14 | (BZ) | 0.088049 | −0.058618 | −0.006705 | 0.141149 |
| | IRS | 0.006603 | −0.090235 | −0.113243 | 0.185858 |
| | (IRS) | −0.849158 | −4.683999 | −4.483094 | 6.606901 |
| 15 | (BZ) | 0.053091 | −0.035578 | −0.003909 | 0.081733 |
| | IRS | 0.004338 | −0.046830 | −0.055569 | 0.087995 |
| | (IRS) | −0.414965 | −2.533893 | −2.698436 | 3.938682 |
| 16 | (BZ) | 0.017550 | −0.011991 | −0.001317 | 0.025814 |
| | IRS | 0.001402 | −0.015624 | −0.017464 | 0.026006 |

Table SM.84: Three loop MOMc scheme $SU(3)$ MAG critical exponents.

| $N_f$ | Type | $\gamma_A$ | $\gamma_c$ | $\gamma_\psi$ | $\rho_m$ |
|---|---|---|---|---|---|
| 8 | - | - | - | - | - |
| 9 | BZ | 5.447734 | −6.344571 | 1.793981 | 26.804168 |
| 10 | BZ | 1.562849 | −1.493417 | 0.277757 | 6.257561 |
| 11 | BZ | 0.755891 | −0.607020 | 0.073953 | 2.514774 |
| 12 | BZ | 0.425300 | −0.295049 | 0.022800 | 1.204608 |
| 13 | BZ | 0.246309 | −0.151565 | 0.006932 | 0.607462 |
| 14 | BZ | 0.135558 | −0.075884 | 0.001795 | 0.297076 |
| 15 | BZ | 0.063193 | −0.033028 | 0.000301 | 0.125435 |
| 16 | BZ | 0.016175 | −0.008132 | 0.000011 | 0.029663 |
| | IRS | 0 | −0.017477 | −0.015641 | 0.032143 |

Table SM.85: Two loop MOMg scheme $SU(3)$ linear covariant gauge critical exponents.

| $N_f$ | Type | $\gamma_A$ | $\gamma_c$ | $\gamma_\psi$ | $\rho_m$ |
|---|---|---|---|---|---|
| 8 | BZ | 0.276082 | −0.413130 | 0.099159 | 1.331235 |
| 9 | BZ | 0.224312 | −0.262619 | 0.042710 | 0.954324 |
| 10 | BZ | 0.193650 | −0.182608 | 0.020019 | 0.701362 |
| 11 | BZ | 0.166770 | −0.131130 | 0.009440 | 0.516777 |
| 12 | BZ | 0.138971 | −0.094074 | 0.004212 | 0.374024 |
| 13 | BZ | 0.109064 | −0.065442 | 0.001649 | 0.259356 |
| | IRS | 0 | −0.155825 | −0.139024 | 0.343730 |
| 14 | BZ | 0.077336 | −0.042319 | 0.000497 | 0.165375 |
| | IRS | 0 | −0.093956 | −0.084584 | 0.196204 |
| 15 | BZ | 0.045066 | −0.023188 | 0.000086 | 0.088262 |
| | IRS | 0 | −0.048493 | −0.043719 | 0.095293 |
| 16 | BZ | 0.014301 | −0.007163 | 0.000003 | 0.026154 |
| | IRS | 0 | −0.014374 | −0.012860 | 0.026451 |

Table SM.86: Three loop MOMg scheme $SU(3)$ linear covariant gauge critical exponents.

| $N_f$ | Type | $\gamma_A$ | $\gamma_c$ | $\gamma_\psi$ | $\rho_m$ |
|---|---|---|---|---|---|
| 8 | (IRS) | 26977.745240 | −8761.999812 | 46537.011944 | 84393.768368 |
| 9 | BZ | 5.447734 | −6.344571 | 1.793981 | 26.804168 |
| | (IRS) | 213.089603 | 26.617298 | 342.886669 | 382.664602 |
| 10 | BZ | 1.562849 | −1.493417 | 0.277757 | 6.257561 |
| 11 | BZ | 0.755891 | −0.607020 | 0.073953 | 2.514774 |
| 12 | BZ | 0.425300 | −0.295049 | 0.022800 | 1.204608 |
| 13 | BZ | 0.246309 | −0.151565 | 0.006932 | 0.607462 |
| 14 | BZ | 0.135558 | −0.075884 | 0.001795 | 0.297076 |
| 15 | BZ | 0.063193 | −0.033028 | 0.000301 | 0.125435 |
| 16 | BZ | 0.016175 | −0.008132 | 0.000011 | 0.029663 |

Table SM.87: Two loop MOMg scheme $SU(3)$ Curci-Ferrari gauge critical exponents.

| $N_f$ | Type | $\gamma_A$ | $\gamma_c$ | $\gamma_\psi$ | $\rho_m$ |
|---|---|---|---|---|---|
| 8 | BZ | 0.276082 | −0.413130 | 0.099159 | 1.331235 |
| | (IRS) | 0.924163 | −0.415299 | 1.476117 | 2.308828 |
| 9 | BZ | 0.224312 | −0.262619 | 0.042710 | 0.954324 |
| | (IRS) | 1.452883 | −0.120220 | 2.190266 | 2.552738 |
| 10 | BZ | 0.193650 | −0.182608 | 0.020019 | 0.701362 |
| | (IRS) | 5.227316 | 0.353456 | 7.616440 | 7.175322 |
| 11 | BZ | 0.166770 | −0.131130 | 0.009440 | 0.516777 |
| 12 | BZ | 0.138971 | −0.094074 | 0.004212 | 0.374024 |
| 13 | BZ | 0.109064 | −0.065442 | 0.001649 | 0.259356 |
| 14 | BZ | 0.077336 | −0.042319 | 0.000497 | 0.165375 |
| 15 | BZ | 0.045066 | −0.023188 | 0.000086 | 0.088262 |
| 16 | BZ | 0.014301 | −0.007163 | 0.000003 | 0.026154 |
| | IRS | −0.017872 | −0.026734 | −0.032502 | 0.033489 |

Table SM.88: Three loop MOMg scheme $SU(3)$ Curci-Ferrari gauge critical exponents.

| $N_f$ | Type | $\gamma_A$ | $\gamma_c$ | $\gamma_\psi$ | $\rho_m$ |
|---|---|---|---|---|---|
| 8 | (BZ) | 36.397695 | −57.496361 | 2.920863 | 160.076441 |
| 9 | (BZ) | 4.832977 | −6.307717 | −0.035783 | 17.080470 |
| 10 | (BZ) | 1.923910 | −2.134559 | −0.086521 | 5.627511 |
| | IRS | 0.039337 | −0.387246 | −0.572603 | 1.545150 |
| 11 | (BZ) | 1.004061 | −0.971472 | −0.061414 | 2.496533 |
| | IRS | 0.033682 | −0.326589 | −0.436505 | 1.054771 |
| 12 | (BZ) | 0.573103 | −0.494757 | −0.038956 | 1.239105 |
| | IRS | 0.025944 | −0.244727 | −0.312662 | 0.673473 |
| 13 | (BZ) | 0.329645 | −0.259395 | −0.023295 | 0.631797 |
| | IRS | 0.018216 | −0.170761 | −0.211732 | 0.410243 |
| 14 | (BZ) | 0.178604 | −0.130875 | −0.012822 | 0.308626 |
| | IRS | 0.011373 | −0.108758 | −0.131105 | 0.230845 |
| 15 | (BZ) | 0.081561 | −0.056999 | −0.005940 | 0.129125 |
| | IRS | 0.005758 | −0.057981 | −0.067596 | 0.109151 |
| 16 | (BZ) | 0.020344 | −0.013983 | −0.001528 | 0.030026 |
| | IRS | 0.001541 | −0.017087 | −0.019051 | 0.028417 |

Table SM.89: Two loop MOMg scheme $SU(3)$ MAG critical exponents.

| $N_f$ | Type | $\gamma_A$ | $\gamma_c$ | $\gamma_\psi$ | $\rho_m$ |
|---|---|---|---|---|---|
| 8 | (BZ) | 0.438993 | −0.692748 | −0.039557 | 1.646751 |
| | IRS | −0.029698 | −0.200073 | −0.183746 | 0.486993 |
| 9 | (BZ) | 0.335178 | −0.440643 | −0.034855 | 1.079969 |
| | IRS | −0.009456 | −0.193145 | −0.197174 | 0.506658 |
| 10 | (BZ) | 0.275999 | −0.306410 | −0.027619 | 0.758291 |
| | IRS | 0.001070 | −0.171865 | −0.185892 | 0.450244 |
| 11 | (BZ) | 0.228961 | −0.220004 | −0.021271 | 0.544096 |
| | IRS | 0.005716 | −0.145500 | −0.164339 | 0.367052 |
| 12 | (BZ) | 0.185274 | −0.157883 | −0.015932 | 0.387345 |
| | IRS | 0.007434 | −0.119473 | −0.139186 | 0.284884 |
| 13 | (BZ) | 0.142121 | −0.109950 | −0.011408 | 0.265692 |
| | IRS | 0.007438 | −0.094446 | −0.111933 | 0.210196 |
| 14 | (BZ) | 0.099005 | −0.071251 | −0.007537 | 0.168103 |
| | IRS | 0.006239 | −0.069643 | −0.082647 | 0.142984 |
| 15 | (BZ) | 0.056867 | −0.039180 | −0.004211 | 0.089115 |
| | IRS | 0.004116 | −0.043831 | −0.051081 | 0.081838 |
| 16 | (BZ) | 0.017803 | −0.012188 | −0.001338 | 0.026215 |
| | IRS | 0.001392 | −0.015520 | −0.017328 | 0.025816 |

Table SM.90: Three loop MOMg scheme $SU(3)$ MAG critical exponents.

| $N_f$ | Type | $\gamma_A$ | $\gamma_c$ | $\gamma_\psi$ | $\rho_m$ |
|---|---|---|---|---|---|
| 8 | - | - | - | - | - |
| 9 | BZ | 6.400386 | $-2.057640$ | 1.793981 | 11.561746 |
| 10 | BZ | 1.494540 | $-0.571245$ | 0.277757 | 2.978729 |
| 11 | BZ | 0.630605 | $-0.268749$ | 0.073953 | 1.312033 |
| 12 | BZ | 0.328685 | $-0.150127$ | 0.022800 | 0.689329 |
| 13 | BZ | 0.185640 | $-0.088562$ | 0.006932 | 0.383454 |
| 14 | BZ | 0.104350 | $-0.051101$ | 0.001795 | 0.208960 |
| | IRS | 0 | $-0.081047$ | $-0.078943$ | 0.157971 |
| 15 | BZ | 0.051980 | $-0.025820$ | 0.000301 | 0.099806 |
| | IRS | 0 | $-0.045219$ | $-0.041596$ | 0.088008 |
| 16 | BZ | 0.014937 | $-0.007464$ | 0.000011 | 0.027285 |
| | IRS | 0 | $-0.014337$ | $-0.012847$ | 0.026365 |

Table SM.91: Two loop MOMq scheme $SU(3)$ linear covariant gauge critical exponents.

| $N_f$ | Type | $\gamma_A$ | $\gamma_c$ | $\gamma_\psi$ | $\rho_m$ |
|---|---|---|---|---|---|
| 8 | BZ | 0.189700 | $-0.247108$ | 0.042127 | 0.671162 |
| | (IRS) | 0 | 0.019875 | 0.713320 | 0.520984 |
| | IRS | 0 | $-0.292880$ | $-0.141041$ | 0.568651 |
| 9 | BZ | 0.189612 | $-0.170966$ | 0.020033 | 0.553462 |
| | IRS | 0 | $-0.225997$ | $-0.144117$ | 0.482308 |
| 10 | BZ | 0.173917 | $-0.125391$ | 0.009356 | 0.452897 |
| | IRS | 0 | $-0.180608$ | $-0.134742$ | 0.406464 |
| 11 | BZ | 0.151840 | $-0.094592$ | 0.004063 | 0.364656 |
| | IRS | 0 | $-0.146612$ | $-0.120352$ | 0.336490 |
| 12 | BZ | 0.126653 | $-0.071608$ | 0.001526 | 0.285218 |
| | IRS | 0 | $-0.118634$ | $-0.103174$ | 0.269817 |
| 13 | BZ | 0.099677 | $-0.052935$ | 0.000439 | 0.212345 |
| | IRS | 0 | $-0.093224$ | $-0.083658$ | 0.205116 |
| 14 | BZ | 0.071577 | $-0.036630$ | 0.000074 | 0.144860 |
| | IRS | 0 | $-0.067999$ | $-0.061735$ | 0.142206 |
| 15 | BZ | 0.042870 | $-0.021550$ | 0.000005 | 0.082504 |
| | IRS | 0 | $-0.041642$ | $-0.037698$ | 0.081920 |
| 16 | BZ | 0.014144 | $-0.007073$ | 0.000002 | 0.025840 |
| | IRS | 0 | $-0.014030$ | $-0.012556$ | 0.025819 |

Table SM.92: Three loop MOMq scheme $SU(3)$ linear covariant gauge critical exponents.

| $N_f$ | Type | $\gamma_A$ | $\gamma_c$ | $\gamma_\psi$ | $\rho_m$ |
|---|---|---|---|---|---|
| 8 | (IRS) | 2537.518045 | −939.486535 | 4435.846505 | 6653.893118 |
| 9 | BZ | 6.400386 | −2.057640 | 1.793981 | 11.561746 |
| | (IRS) | 2.863306 | 0.145466 | 4.607263 | 5.401336 |
| 10 | BZ | 1.494540 | −0.571245 | 0.277757 | 2.978729 |
| 11 | BZ | 0.630605 | −0.268749 | 0.073953 | 1.312033 |
| 12 | BZ | 0.328685 | −0.150127 | 0.022800 | 0.689329 |
| 13 | BZ | 0.185640 | −0.088562 | 0.006932 | 0.383454 |
| 14 | BZ | 0.104350 | −0.051101 | 0.001795 | 0.208960 |
| 15 | BZ | 0.051980 | −0.025820 | 0.000301 | 0.099806 |
| | IRS | −0.045251 | −0.065684 | −0.086820 | 0.089073 |
| 16 | BZ | 0.014937 | −0.007464 | 0.000011 | 0.027285 |
| | IRS | −0.014114 | −0.021112 | −0.025641 | 0.026415 |

Table SM.93: Two loop MOMq scheme $SU(3)$ Curci-Ferrari gauge critical exponents.

| $N_f$ | Type | $\gamma_A$ | $\gamma_c$ | $\gamma_\psi$ | $\rho_m$ |
|---|---|---|---|---|---|
| 8 | BZ | 0.189700 | −0.247108 | 0.042127 | 0.671162 |
| | (IRS) | 0.325308 | −0.155226 | 0.508723 | 0.844402 |
| | IRS | −0.179695 | −0.376253 | −0.262788 | 0.583274 |
| 9 | BZ | 0.189612 | −0.170966 | 0.020033 | 0.553462 |
| | (IRS) | 0.312662 | −0.008175 | 0.475178 | 0.589581 |
| | IRS | −0.153980 | −0.292270 | −0.245203 | 0.493722 |
| 10 | BZ | 0.173917 | −0.125391 | 0.009356 | 0.452897 |
| | (IRS) | 0.256557 | 0.063582 | 0.393010 | 0.363224 |
| | IRS | −0.130485 | −0.231574 | −0.221890 | 0.412805 |
| 11 | BZ | 0.151840 | −0.094592 | 0.004063 | 0.364656 |
| | (IRS) | 0.177706 | 0.088548 | 0.280144 | 0.169961 |
| | IRS | −0.110305 | −0.186018 | −0.198121 | 0.338608 |
| 12 | BZ | 0.126653 | −0.071608 | 0.001526 | 0.285218 |
| | IRS | −0.092896 | −0.150331 | −0.174062 | 0.269299 |
| 13 | BZ | 0.099677 | −0.052935 | 0.000439 | 0.212345 |
| | IRS | −0.076738 | −0.120097 | −0.147352 | 0.203649 |
| 14 | BZ | 0.071577 | −0.036630 | 0.000074 | 0.144860 |
| | IRS | −0.059450 | −0.090785 | −0.114343 | 0.141085 |
| 15 | BZ | 0.042870 | −0.021550 | 0.000005 | 0.082504 |
| | IRS | −0.038683 | −0.058270 | −0.072841 | 0.081552 |
| 16 | BZ | 0.014144 | −0.007073 | 0.000002 | 0.025840 |
| | IRS | −0.013724 | −0.020589 | −0.024909 | 0.025802 |

Table SM.94: Three loop MOMq scheme $SU(3)$ Curci-Ferrari gauge critical exponents.

| $N_f$ | Type | $\gamma_A$ | $\gamma_c$ | $\gamma_\psi$ | $\rho_m$ |
|---|---|---|---|---|---|
| 8 | - | - | - | - | - |
| 9 | (BZ) | 4.648447 | $-2.204111$ | 0.905996 | 7.514205 |
| 10 | (BZ) | 1.559730 | $-0.774502$ | 0.183526 | 2.579218 |
| 11 | (BZ) | 0.740227 | $-0.390259$ | 0.043253 | 1.232651 |
| 12 | (BZ) | 0.404325 | $-0.226997$ | 0.005304 | 0.669361 |
| 13 | (BZ) | 0.232342 | $-0.138443$ | $-0.004877$ | 0.378241 |
| 14 | (BZ) | 0.131021 | $-0.082316$ | $-0.006009$ | 0.207777 |
| | IRS | 0.009890 | $-0.063807$ | $-0.095001$ | 0.152523 |
| 15 | (BZ) | 0.065028 | $-0.042737$ | $-0.004102$ | 0.099636 |
| | IRS | 0.005004 | $-0.043885$ | $-0.054696$ | 0.086454 |
| 16 | (BZ) | 0.018558 | $-0.012656$ | $-0.001372$ | 0.027281 |
| | IRS | 0.001438 | $-0.015691$ | $-0.017617$ | 0.026233 |

Table SM.95: Two loop MOMq scheme $SU(3)$ MAG critical exponents.

| $N_f$ | Type | $\gamma_A$ | $\gamma_c$ | $\gamma_\psi$ | $\rho_m$ |
|---|---|---|---|---|---|
| 8 | (BZ) | 0.346592 | $-0.411508$ | $-0.041294$ | 0.717971 |
| | IRS | $-0.132028$ | $-0.841025$ | $-0.383689$ | 0.643444 |
| 9 | (BZ) | 0.297538 | $-0.279798$ | $-0.027555$ | 0.592685 |
| | IRS | $-0.077144$ | $-0.495177$ | $-0.299364$ | 0.530421 |
| 10 | BZ | 0.250981 | $-0.204323$ | $-0.020839$ | 0.479055 |
| | IRS | $-0.041489$ | $-0.313878$ | $-0.239936$ | 0.434601 |
| 11 | (BZ) | 0.207877 | $-0.154160$ | $-0.016380$ | 0.380314 |
| | IRS | $-0.018655$ | $-0.209733$ | $-0.193922$ | 0.351356 |
| 12 | (BZ) | 0.167371 | $-0.117002$ | $-0.012761$ | 0.293629 |
| | IRS | $-0.004711$ | $-0.145483$ | $-0.155019$ | 0.276501 |
| 13 | (BZ) | 0.128545 | $-0.086897$ | $-0.009551$ | 0.216209 |
| | IRS | 0.002606 | $-0.102882$ | $-0.119598$ | 0.207414 |
| 14 | (BZ) | 0.090759 | $-0.060566$ | $-0.006621$ | 0.146218 |
| | IRS | 0.004944 | $-0.071411$ | $-0.085559$ | 0.142727 |
| 15 | (BZ) | 0.053726 | $-0.036016$ | $-0.003913$ | 0.082779 |
| | IRS | 0.003965 | $-0.043956$ | $-0.051686$ | 0.081985 |
| 16 | (BZ) | 0.017573 | $-0.012008$ | $-0.001319$ | 0.025849 |
| | IRS | 0.001391 | $-0.015517$ | $-0.017339$ | 0.025820 |

Table SM.96: Three loop MOMq scheme $SU(3)$ MAG critical exponents.
